# Supplementary material for: Simultaneous $\gamma$-ray and electron spectroscopy of $^{182,184,186}$Hg isotopes
Source: arXiv:2305.16442 ancillary file (2023-06-06)
Supplement: Supplementary file 1 [file suppl.pdf]

# Supplemental Material for "Simultaneous $\gamma$-ray and electron spectroscopy of $^{182,184,186}$Hg isotopes"


M. Stryjczyk,[1,2,*] B. Andel,[1,3,†] J. G. Cubiss,[4,5,†] K. Rezynkina,[1,6,†] T. R. Rodríguez,[7,8] J. E. García-Ramos,[9,10] A. N. Andreyev,[5,11] J. Pakarinen,[2,12] P. Van Duppen,[1] S. Antalic,[3] T. Berry,[13] M. J. G. Borge,[14,4] C. Clisu,[15] D. M. Cox,[16] H. De Witte,[1] L. M. Fraile,[8] H. O. U. Fynbo,[17] L. P. Gaffney,[4,18] L. J. Harkness-Brennan,[18] M. Huyse,[1] A. Illana,[19,2,8] D. S. Judson,[18] J. Konki,[4] J. Kurcewicz,[4] I. Lazarus,[20] R. Lica,[15,4] M. Madurga,[4] N. Marginean,[15] R. Marginean,[15] C. Mihai,[15] P. Mosat,[3] E. Nacher,[21] A. Negret,[15] J. Ojala,[2,12] J. D. Ovejas,[14] R. D. Page,[18] P. Papadakis,[18,20] S. Pascu,[15] A. Perea,[14] Zs. Podolyák,[13] L. Próchniak,[22] V. Pucknell,[20] E. Rapisarda,[4] F. Rotaru,[15] C. Sotty,[15] O. Tengblad,[14] V. Vedia,[8] S. Viñals,[14] R. Wadsworth,[5] N. Warr,[23] and K. Wrzosek-Lipska[22]

(IDS Collaboration)

[1] *KU Leuven, Instituut voor Kern- en Stralingsfysica, Celestijnenlaan 200D, 3001 Leuven, Belgium*
[2] *University of Jyvaskyla, Department of Physics, Accelerator laboratory, P.O. Box 35, FI-40014 University of Jyvaskyla, Finland*
[3] *Department of Nuclear Physics and Biophysics, Comenius University in Bratislava, 84248 Bratislava, Slovakia*
[4] *ISOLDE, CERN, CH-1211 Geneva 23, Switzerland*
[5] *School of Physics, Engineering and Technology, University of York, York, YO10 5DD, United Kingdom*
[6] *INFN Sezione di Padova, I-35131 Padova, Italy*
[7] *Departamento de Física Teórica and Centro de Investigación Avanzada en Física Fundamental, Universidad Autónoma de Madrid, E-28049 Madrid, Spain*
[8] *Grupo de Física Nuclear, Universidad Complutense de Madrid, 28040, Madrid, Spain*
[9] *Departamento de Ciencias Integradas y Centro de Estudios Avanzados en Física, Matemática y Computación, Universidad de Huelva, 21071 Huelva, Spain*
[10] *Instituto Carlos I de Física Teórica y Computacional, Universidad de Granada, Fuentenueva s/n, 18071 Granada, Spain*
[11] *Advanced Science Research Center, Japan Atomic Energy Agency, Tokai-mura, Japan*
[12] *Helsinki Institute of Physics, University of Helsinki, P.O. Box 64, FI-00014, Helsinki, Finland*
[13] *Department of Physics, University of Surrey, Guildford GU2 7XH, United Kingdom*
[14] *Instituto de Estructura de la Materia, CSIC, Serrano 113 bis, E-28006 Madrid, Spain*
[15] *"Horia Hulubei" National Institute for Physics and Nuclear Engineering, RO-077125 Bucharest, Romania*
[16] *Department of Physics, Lund University, Lund S-22100, Sweden*
[17] *Department of Physics and Astronomy, Aarhus University, DK-8000 Aarhus C, Denmark*
[18] *Department of Physics, Oliver Lodge Laboratory, University of Liverpool, Liverpool L69 7ZE, United Kingdom*
[19] *Istituto Nazionale di Fisica Nucleare, Laboratori Nazionali di Legnaro, Legnaro 35020, Italy*
[20] *STFC Daresbury Laboratory, Daresbury, Warrington WA4 4AD, United Kingdom*
[21] *Instituto de Física Corpuscular, CSIC - Universidad de Valencia, E-46980, Valencia, Spain*
[22] *Heavy Ion Laboratory, University of Warsaw, PL-02-093, Warsaw, Poland*
[23] *Institut für Kernphysik, Universität zu Köln, 50937 Köln, Germany*



(Dated: May 25, 2023)


The $\gamma$-ray intensities were extracted from the $\gamma$-ray singles energy spectra, unless it was not possible due to the overlap with lines from daughter nuclei, low $\gamma$-ray intensity or a complex peak structure. These transitions are labeled with an asterisk (*) in the following tables.

The branching ratios $Br_\gamma$ in Tables I, III and V are calculated using the formula:

$$Br_\gamma = 100 \times \frac{N_\gamma}{N_\gamma^s}, \quad (1)$$

where $N_\gamma$ and $N_\gamma^s$ are the efficiency-corrected numbers of counts of the $\gamma$-ray of interest and the strongest $\gamma$ ray de-exciting a given state, respectively. In case of the transition intensities $I_\gamma$ in Tables II, IV and VI, they are calculated as follows:

$$I_\gamma = 100 \times \frac{N_\gamma}{N_\gamma(2_1^+ \rightarrow 0_1^+)}, \quad (2)$$

where where $N_\gamma$ and $N_\gamma(2_1^+ \rightarrow 0_1^+)$ are the efficiency-corrected numbers of counts of the $\gamma$-ray of interest and the $2_1^+ \rightarrow 0_1^+$ $\gamma$ ray in a given nucleus, respectively. The uncertainties were calculated using a standard propagation method.

Decay schemes have the same color code as in the manuscript: levels and transitions known from the previous $\beta$-decay studies are plotted in black, shifted in the


* marek.m.stryjczyk@jyu.fi, he/him
† These authors contributed equally

decay scheme in blue, known from other studies in green and newly identified in red. Please note that the lower and upper part of each page is on a different scale for visualization purposes.

TABLE I: Transition properties obtained in the present work for $^{182}$Hg. Level energies, spins and parities of the initial ($E_i$, $J_i^\pi$) and final ($E_f$, $J_f^\pi$) states, transition energies ($E_t$) and $\gamma$-branching ratios ($Br_\gamma$) have been listed. Pure $E0$ transitions are written in italics. The spins and parities of the states are taken from this work and Ref. [1].

| $E_i$ (keV) | $J_i^\pi$ | $E_f$ (keV) | $J_f^\pi$ | $E_t$ (keV) | $Br_\gamma$ |
|---|---|---|---|---|---|
| 335.0(1) | $0^+$ | 0.0 | $0^+$ | *335.0(1)* | *100* |
| 351.1(1) | $2^+$ | 0.0 | $0^+$ | 351.1(1) | 100(5) |
| | | 335.0(1) | $0^+$ | 16.1(2) | $5.8(8) \times 10^{-5}$ [1] |
| 547.6(1) | $2^+$ | 0.0 | $0^+$ | 547.6(1) | 100(5) |
| | | 335.0(1) | $0^+$ | 212.6(1) | 4.8(6)* |
| | | 351.1(1) | $2^+$ | 196.5(1) | 6.7(8)* |
| 612.0(1) | $4^+$ | 351.1(1) | $2^+$ | 260.9(1) | 100 |
| 944.4(1) | $6^+$ | 612.0(1) | $4^+$ | 332.4(1) | 100 |
| 972.6(1) | $2^+$ | 0.0 | $0^+$ | 972.6(1) | < 4.0 [2] |
| | | 335.0(1) | $0^+$ | 637.7(1) | 97(10)* |
| | | 351.1(1) | $2^+$ | 621.5(1) | 100(5) |
| 1073.8(1) | | 351.1(1) | $2^+$ | 722.7(1) | 100(5) |
| | | 547.6(1) | $2^+$ | 526.2(1) | 68(5)* |
| | | 612.0(1) | $4^+$ | 462.0(2) | 30(7)* |
| 1123.9(1) | $4^+$ | 351.1(1) | $2^+$ | 772.8(1) | 51(4)* |
| | | 547.6(1) | $2^+$ | 576.4(1) | 100(5)* |
| | | 612.0(1) | $4^+$ | 511.9(1) | 9.9(59) [3] |
| 1295.0(1) | | 351.1(1) | $2^+$ | 943.9(1) | < 0.7 [2] |
| | | 547.6(1) | $2^+$ | 747.5(1) | 100(5) |
| | | 612.0(1) | $4^+$ | 683.1(1) | 30(2) |
| | | 972.6(1) | $2^+$ | 322.4(1) | 5.7(4) |
| 1357.5(1) | $8^+$ | 944.4(1) | $6^+$ | 413.1(1) | 100 |
| 1382.3(1) | | 612.0(1) | $4^+$ | 770.2(1) | 100(5)* |
| | | 944.4(1) | $6^+$ | 438.0(1) | 15.7(15)* |
| | | 1073.8(1) | | 308.5(1) | 23.8(18) |
| 1507.4(1) | $3^-$, $4^+$ | 351.1(1) | $2^+$ | 1156.4(1) | 100(6)* |
| | | 547.6(1) | $2^+$ | 959.8(1) | 58(6)* |
| | | 972.6(1) | $2^+$ | 534.8(1) | 16.0(15) |
| 1530.6(1) | $(6)^+$ | 612.0(1) | $4^+$ | 918.5(1) | 22.0(17) |
| | | 944.4(1) | $6^+$ | 586.3(1) | 100(5) |
| | | 1123.9(1) | $4^+$ | 406.7(1) | 63(5) |
| 1547.4(1) | $4^+$ | 351.1(1) | $2^+$ | 1196.3(1) | 100(5) |
| | | 612.0(1) | $4^+$ | 935.4(2) | 54(9)* |
| | | 944.4(1) | $6^+$ | 603.0(2) | 27(3)* |
| 1673.8(1) | | 972.6(1) | $2^+$ | 701.3(1) | 100(77)* |
| | | 1073.8(1) | | 600.0(1) | 45(35)* |
| 1718.5(1) | $3^-$, $4^+$ | 351.1(1) | $2^+$ | 1367.2(5) | 12.5(45)* |
| | | 547.6(1) | $2^+$ | 1171.0(1) | 100(5) |
| | | 1073.8(1) | | 644.7(2) | 28(6)* |
| | | 1295.0(1) | | 423.2(2) | 26(5)* |
| | | 1507.4(1) | $3^-$, $4^+$ | 211.0(2) | < 12 [4] |
| 1760.6(1) | | 944.4(1) | $6^+$ | 816.0(1) | 100(5) |
| | | 1357.5(1) | $8^+$ | 403.1(2) | 3.9(13) |
| | | 1382.3(1) | | 378.3(1) | 68(7)* |
| 1766.1(1) | $(5^-)$ | 612.0(1) | $4^+$ | 1154.2(1) | 33(4)* |
| | | 1123.9(1) | $4^+$ | 642.2(2) | 23(4)* |
| | | 1295.0(1) | | 471.0(1) | 100(5) |
| | | 1507.4(1) | $3^-$, $4^+$ | 258.4(2) | 17(6)* |
| | | 1547.4(1) | $4^+$ | 218.6(2) | 10(2)* |
| 1787.2(1) | | 1073.8(1) | | 713.5(1) | 100(9)* |

*Continued Table I*

| $E_i$ (keV) | $J_i^\pi$ | $E_f$ (keV) | $J_f^\pi$ | $E_t$ (keV) | $Br_\gamma$ |
|---|---|---|---|---|---|
| | | 1123.9(1) | $4^+$ | 663.1(3) | 10(3)* |
| 1794.3(1) | | 612.0(1) | $4^+$ | 1182.3(2) | 100(15)* |
| | | 944.4(1) | $6^+$ | 849.9(1) | 40(7) |
| 1816.3(1) | | 547.6(1) | $2^+$ | 1268.7(1) | 100 |
| 1820.7(1) | | 612.0(1) | $4^+$ | 1208.7(1) | 98(7) |
| | | 944.4(1) | $6^+$ | 876.6(3) | 41(9)* |
| | | 1123.9(1) | $4^+$ | 696.7(1) | 100(5) |
| | | 1295.0(1) | | 525.7(1) | 72(10)* |
| 1843.8(2) | $10^+$ | 1357.5(1) | $8^+$ | 486.3(1) | 100 |
| 1849.9(2) | | 1123.9(1) | $4^+$ | 726.1(1) | 75.6(58) |
| | | 1295.0(1) | | 554.6(1) | 100.0(54) |
| | | 1382.3(1) | | 467.8(1) | 99.5(76) |
| 1932.6(1) | | 1073.8(1) | | 858.7(1) | 100 |
| 1942.4(2) | $(8)^+$ | 1530.6(1) | $(6)^+$ | 411.8(2) | 100 |
| 1962.9(1) | | 1073.8(1) | | 889.2(1) | 100(11)* |
| | | 1507.4(1) | $3^-$, $4^+$ | 455.3(2) | 22(6)* |
| 1963.5(1) | | 1123.9(1) | $4^+$ | 839.6(1) | 100(5) |
| | | 1295.0(1) | | 668.4(2) | 24(5)* |
| 1964.0(2) | | 612.0(1) | $4^+$ | 1352.0(1) | 54(16) |
| | | 944.4(1) | $6^+$ | 1019.4(1) | 46(13) |
| | | 1382.3(1) | | 582.0(4) | 95(39)* |
| | | 1547.4(1) | $4^+$ | 416.9(4) | 100(27)* |
| 1984.9(1) | $(5^-)$ | 612.0(1) | $4^+$ | 1372.8(1) | 29(2) |
| | | 944.4(1) | $6^+$ | 1040.7(3) | 3.6(18)* |
| | | 1123.9(1) | $4^+$ | 861.0(1) | 100(5) |
| | | 1295.0(1) | | 689.7(1) | 47(3) |
| | | 1507.4(1) | $3^-$, $4^+$ | 477.4(1) | 14.4(11) |
| | | 1673.8(1) | | 311.2(1) | 5.1(5) |
| | | 1766.1(1) | $(5^-)$ | 219.1(2) | 12(2)* |
| 2004.9(1) | $(7^-)$ | 944.4(1) | $6^+$ | 1060.6(3) | 16(5)* |
| | | 1766.1(1) | $(5^-)$ | 238.8(1) | 100(6) |
| 2009.0(2) | | 1718.5(1) | $3^-$, $4^+$ | 290.5(1) | 100 |
| 2009.7(2) | | 1073.8(1) | | 936.0(2) | 26(4)* |
| | | 1123.9(1) | $4^+$ | 886.0(1) | 37(4)* |
| | | 1382.3(1) | | 627.2(1) | 100(5) |
| | | 1787.2(1) | | 222.2(3) | 7(2)* |
| 2025.4(1) | | 612.0(1) | $4^+$ | 1413.4(1) | 100(5) |
| | | 1073.8(1) | | 951.5(1) | 58(6) |
| 2036.5(2) | $(5^-)$ | 612.0(1) | $4^+$ | 1424.9(2) | 32(8)* |
| | | 944.4(1) | $6^+$ | 1092.2(1) | 12.2(12) |
| | | 1123.9(1) | $4^+$ | 912.5(1) | 100(8)* |
| | | 1295.0(1) | | 741.5(2) | 48(9)* |
| | | 1673.8(1) | | 362.7(3) | 10(3)* |
| 2052.8(2) | | 612.0(1) | $4^+$ | 1440.7(1) | 71(6) |
| | | 1073.8(1) | | 979.3(2) | 81(13)* |
| | | 1123.9(1) | $4^+$ | 928.7(1) | 100(6) |
| 2059.4(1) | | 1295.0(1) | | 764.2(2) | 100(15)* |
| | | 1382.3(1) | | 677.2(2) | 56(14)* |
| 2097.3(1) | | 547.6(1) | $2^+$ | 1549.8(1) | 100 |
| 2099.0(2) | | 612.0(1) | $4^+$ | 1487.0(1) | 100 |
| 2108.2(1) | | 1295.0(1) | | 813.1(1) | 100(9)* |
| | | 1547.4(1) | $4^+$ | 560.8(2) | 10(3)* |
| 2121.4(1) | | 612.0(1) | $4^+$ | 1509.4(1) | 100 |
| 2138.8(1) | | 1295.0(1) | | 843.7(1) | 100 |
| 2139.6(2) | | 1382.3(1) | | 757.3(2) | 100 |
| 2151.5(4) | | 1507.4(1) | $3^-$, $4^+$ | 644.0(4) | 100 |
| 2152.2(1) | | 1123.9(1) | $4^+$ | 1028.3(1) | 100 |
| 2161.9(1) | | 1295.0(1) | | 866.9(1) | 100 |
| 2173.7(2) | | 1295.0(1) | | 878.3(5) | 78(53)* |
| | | 1382.3(1) | | 791.4(2) | 100(28)* |
| 2186.7(2) | | 1530.6(1) | $(6)^+$ | 656.1(2) | 100 |

*Continued Table I*

| $E_i$ (keV) | $J_i^\pi$ | $E_f$ (keV) | $J_f^\pi$ | $E_t$ (keV) | $Br_\gamma$ |
|---|---|---|---|---|---|
| 2187.7(1) | | 612.0(1) | $4^+$ | 1575.7(1) | 100 |
| 2192.1(2) | | 1530.6(1) | $(6)^+$ | 661.4(2) | 100 |
| 2207.1(1) | | 1760.6(1) | | 446.5(1) | 100 |
| 2235.3(2) | | 944.4(1) | $6^+$ | 1291.1(4) | 6.2(19) |
| | | 1382.3(1) | | 853.1(1) | 100(5) |
| | | 1530.6(1) | $(6)^+$ | 704.2(2) | 6.5(12) |
| 2237.2(2) | | 1507.4(1) | $3^-$, $4^+$ | 729.7(2) | 100 |
| 2241.2(2) | | 944.4(1) | $6^+$ | 1296.8(1) | 100 |
| 2242.6(3) | | 1530.6(1) | $(6)^+$ | 711.9(3) | 100 |
| 2276.5(2) | | 1530.6(1) | $(6)^+$ | 745.9(2) | 100 |
| 2283.7(2) | | 1530.6(1) | $(6)^+$ | 753.1(2) | 100 |
| 2285.5(1) | | 612.0(1) | $4^+$ | 1673.4(1) | 100(5) |
| | | 944.4(1) | $6^+$ | 1341.0(1) | 86(7) |
| | | 1766.1(1) | $(5^-)$ | 519.5(2) | 51(16)* |
| | | 1787.2(1) | | 498.9(5) | 18(6)* |
| 2304.9(1) | | 944.4(1) | $6^+$ | 1360.5(1) | 100 |
| 2307.7(3) | | 944.4(1) | $6^+$ | 1363.3(2) | 100 |
| 2310.4(1) | | 1760.6(1) | | 549.9(1) | 100(5) |
| | | 2009.7(2) | | 300.8(1) | 45(4) |
| 2341.9(2) | $(5^-)$ | 944.4(1) | $6^+$ | 1397.4(1) | 86(8) |
| | | 1123.9(1) | $4^+$ | 1217.9(1) | 100(7)* |
| | | 1295.0(1) | | 1046.7(1) | 45(4) |
| | | 1382.3(1) | | 959.9(3) | 7(2)* |
| | | 1507.4(1) | $3^-$, $4^+$ | 834.2(2) | 15(3)* |
| | | 1766.1(1) | $(5^-)$ | 576.0(2) | 27(5)* |
| | | 1984.9(1) | $(5^-)$ | 357.1(2) | 15(3)* |
| 2354.1(4) | | 1295.0(1) | | 1059.1(3) | 100 |
| 2357.5(1) | | 612.0(1) | $4^+$ | 1745.5(1) | 76(7) |
| | | 1530.6(1) | $(6)^+$ | 826.9(1) | 100(6) |
| 2360.3(5) | | 1382.3(1) | | 978.0(5) | 100 |
| 2369.6(2) | | 612.0(1) | $4^+$ | 1757.7(1) | 100(6) |
| | | 944.4(1) | $6^+$ | 1425.2(3) | 59(13)* |
| | | 1123.9(1) | $4^+$ | 1245.2(4) | 42(14)* |
| 2378.5(1) | | 944.4(1) | $6^+$ | 1434.1(1) | 100 |
| 2381.1(4) | | 1123.9(1) | $4^+$ | 1257.2(4) | 100 |
| 2391.7(1) | | 612.0(1) | $4^+$ | 1779.8(1) | 100(8) |
| | | 944.4(1) | $6^+$ | 1447.2(1) | 89(9) |
| 2418.2(2) | $(5^-)$ | 612.0(1) | $4^+$ | 1806.2(1) | 100(5) |
| | | 944.4(1) | $6^+$ | 1473.9(1) | 90(7) |
| | | 1123.9(1) | $4^+$ | 1294.0(1) | 49(4) |
| | | 1295.0(1) | | 1123.0(2) | 19(3)* |
| | | 1382.3(1) | | 1036.0(1) | 30(2) |
| | | 1507.4(1) | $3^-$, $4^+$ | 910.9(1) | 28(4)* |
| | | 1673.8(1) | | 744.7(2) | 31(8)* |
| | | 1787.2(1) | | 630.8(1) | 12.0(16)* |
| | | 1984.9(1) | $(5^-)$ | 433.3(2) | 27(6)* |
| | | 2036.5(2) | $(5^-)$ | 381.8(3) | 22(5)* |
| 2447.9(2) | $(5^-)$ | 612.0(1) | $4^+$ | 1835.9(1) | 100(5) |
| | | 944.4(1) | $6^+$ | 1504.7(8) | 2.3(12)* |
| | | 1123.9(1) | $4^+$ | 1324.2(2) | 9.1(16)* |
| | | 1382.3(1) | | 1066.1(4) | 3.3(13)* |
| | | 1507.4(1) | $3^-$, $4^+$ | 940.4(1) | 13.1(18)* |
| | | 1673.8(1) | | 774.3(2) | 11(3)* |
| | | 1718.5(1) | $3^-$, $4^+$ | 729.8(2) | 7(2)* |
| | | 1766.1(1) | $(5^-)$ | 681.7(1) | 23(2) |
| | | 1787.2(1) | | 660.4(2) | 5.0(8)* |
| | | 1984.9(1) | $(5^-)$ | 463.2(1) | 21(3)* |
| | | 2009.7(2) | | 437.9(2) | 11(3)* |
| | | 2052.8(2) | | 395.0(5) | 4.0(18)* |
| 2464.2(3) | | 1357.5(1) | $8^+$ | 1106.7(3) | 100 |
| 2480.3(1) | | 944.4(1) | $6^+$ | 1535.8(1) | 100(10) |
| | | 1673.8(1) | | 806.5(1) | 95(11) |
| 2501.4(1) | | 612.0(1) | $4^+$ | 1889.4(1) | 100(7) |
| | | 944.4(1) | $6^+$ | 1557.0(1) | 79(7) |
| 2548.8(2) | | 944.4(1) | $6^+$ | 1604.3(1) | 100 |
| 2564.0(1) | | 612.0(1) | $4^+$ | 1952.0(1) | 100 |
| 2565.0(2) | | 944.4(1) | $6^+$ | 1620.5(1) | 100 |
| 2574.2(1) | | 944.4(1) | $6^+$ | 1629.7(1) | 100 |
| 2586.1(1) | | 612.0(1) | $4^+$ | 1974.2(1) | 100(6) |
| | | 1123.9(1) | $4^+$ | 1462.5(5) | 28(12)* |
| | | 1766.1(1) | $(5^-)$ | 819.8(2) | 44(10)* |
| 2616.5(2) | | 1547.4(1) | $4^+$ | 1069.1(2) | 100 |
| 2633.4(1) | | 612.0(1) | $4^+$ | 2021.4(1) | 100 |
| 2645.9(2) | | 1507.4(1) | $3^-$, $4^+$ | 1138.4(2) | 100 |
| 2686.4(2) | | 944.4(1) | $6^+$ | 1742.2(1) | 100(6) |
| | | 1123.9(1) | $4^+$ | 1562.4(1) | 76(6) |
| | | 1295.0(1) | | 1391.6(6) | 17(8)* |
| | | 1673.8(1) | | 1012.3(1) | 72(6) |
| 2711.2(1) | | 612.0(1) | $4^+$ | 2099.2(1) | 100 |
| 2712.0(2) | | 944.4(1) | $6^+$ | 1767.5(1) | 100 |
| 2722.6(5) | | 944.4(1) | $6^+$ | 1778.1(5) | 100 |
| 2744.0(2) | | 612.0(1) | $4^+$ | 2132.0(2) | 100 |
| 2768.1(2) | | 944.4(1) | $6^+$ | 1823.7(1) | 100 |
| 2990.1(1) | | 1507.4(1) | $3^-$, $4^+$ | 1482.7(1) | 100 |

[1] $\gamma$ ray not observed, transition intensity obtained from $\gamma$-electron coincidence data, see text for details.

[2] $\gamma$ ray not observed, upper limit, given within 95% credible interval, obtained from the $\gamma$-$\gamma$ coincidence data.

[3] Branching ratio obtained by comparing the intensity of the 1218-keV transition in different gates and by subtracting the contribution from conversion electrons, see text for details.

[4] Observed only as conversion electrons, $\gamma$-ray intensity limits given with 95% credible interval.

TABLE II: The relative $\gamma$-ray intensities in $^{182}$Hg, normalized to the strongest $2_1^+ \rightarrow 0_1^+$ 351-keV transition. The intensities of transitions marked with * were determined from coincidences. The relative intensity of the 335-keV $E0$ transition was not determined as the K-conversion electrons overlaps with the K conversion electrons of the yrast 332-keV transition and the L-and M+-conversion electrons of the yrast 261-keV transition.

| $E_\gamma$ (keV) | $I_\gamma$ | $E_i$ (keV) | $E_f$ (keV) |
|---|---|---|---|
| 16.1(2)[1] | $5.8(8) \times 10^{-5}$ | 351.1(1) | 335.0(1) |
| 196.5(1) | 1.35(15)* | 547.6(1) | 351.1(1) |
| 211.0(2) | < 0.121[2] | 1718.5(1) | 1507.4(1) |
| 212.6(1) | 0.97(12)* | 547.6(1) | 335.0(1) |
| 218.6(2) | 0.40(8)* | 1766.1(1) | 1547.4(1) |
| 219.1(2) | 0.59(11)* | 1984.9(1) | 1766.1(1) |
| 222.2(3) | 0.16(5)* | 2009.7(2) | 1787.2(1) |
| 238.8(1) | 1.17(9) | 2004.9(1) | 1766.1(1) |
| 258.4(2) | 0.7(2)* | 1766.1(1) | 1507.4(1) |
| 260.9(1) | 65(5) | 612.0(1) | 351.1(1) |
| 290.5(1) | 0.17(2) | 2009.0(2) | 1718.5(1) |
| 300.8(1) | 0.35(3) | 2310.4(1) | 2009.7(2) |
| 308.5(1) | 1.58(12) | 1382.3(1) | 1073.8(1) |
| 311.2(1) | 0.26(3) | 1984.9(1) | 1673.8(1) |
| 322.4(1) | 0.57(4) | 1295.0(1) | 972.6(1) |
| 332.4(1) | 28(2) | 944.4(1) | 612.0(1) |
| 351.1(1) | 100 | 351.1(1) | 0.0 |
| 357.1(2) | 0.37(8)* | 2341.9(1) | 1984.9(1) |

| $E_\gamma$ (keV) | $I_\gamma$ | $E_i$ (keV) | $E_f$ (keV) |
|---|---|---|---|
| 362.7(3) | 0.17(6)* | 2036.5(2) | 1673.8(1) |
| 378.3(1) | 1.16(11)* | 1760.6(1) | 1382.3(1) |
| 381.8(3) | 0.41(10)* | 2418.2(2) | 2036.5(2) |
| 395.0(5) | 0.17(8)* | 2447.9(2) | 2052.8(2) |
| 403.1(2) | 0.07(2) | 1760.6(1) | 1357.5(1) |
| 406.7(1) | 2.00(14) | 1530.6(1) | 1123.9(1) |
| 411.8(2) | 1.1(3)* | 1942.4(2) | 1530.6(1) |
| 413.1(1) | 4.3(3)* | 1357.5(1) | 944.4(1) |
| 416.9(4) | 0.21(6)* | 1964.0(2) | 1547.4(1) |
| 423.2(2) | 0.27(5)* | 1718.5(1) | 1295.0(1) |
| 433.3(2) | 0.51(10)* | 2418.2(2) | 1984.9(1) |
| 437.9(2) | 0.47(13)* | 2447.9(2) | 2009.7(2) |
| 438.0(1) | 1.04(10)* | 1382.3(1) | 944.4(1) |
| 446.5(1) | 0.27(2) | 2207.1(1) | 1760.6(1) |
| 455.3(2) | 0.21(5)* | 1962.9(1) | 1507.4(1) |
| 462.0(2) | 1.5(4)* | 1073.8(1) | 612.0(1) |
| 463.2(1) | 0.89(11)* | 2447.9(2) | 1984.9(1) |
| 467.8(1) | 0.49(4) | 1849.9(2) | 1382.3(1) |
| 471.0(1) | 3.9(3) | 1766.1(1) | 1295.0(1) |
| 477.4(1) | 0.73(5) | 1984.9(1) | 1507.4(1) |
| 486.3(1) | 0.34(3) | 1843.8(2) | 1357.5(1) |
| 498.9(5) | 0.12(4)* | 2285.5(1) | 1787.2(1) |
| 511.9(1)[1] | 1.18(70)* | 1123.9(1) | 612.0(1) |
| 519.5(2) | 0.34(11)* | 2285.5(1) | 1766.1(1) |
| 525.7(1) | 0.54(7)* | 1820.7(1) | 1295.0(1) |
| 526.2(1) | 3.5(3)* | 1073.8(1) | 547.6(1) |
| 534.8(1) | 0.39(3) | 1507.4(1) | 972.6(1) |
| 547.6(1) | 20.1(14) | 547.6(1) | 0.0 |
| 549.9(1) | 0.76(6) | 2310.4(1) | 1760.6(1) |
| 554.6(1) | 0.49(4) | 1849.9(2) | 1295.0(1) |
| 560.8(2) | 0.09(3)* | 2108.2(1) | 1547.4 |
| 576.0(2) | 0.68(11)* | 2341.9(1) | 1766.1(1) |
| 576.4(1) | 11.9(9)* | 1123.9(1) | 547.6(1) |
| 582.0(4) | 0.20(6)* | 1964.0(2) | 1382.3(1) |
| 586.3(1) | 3.2(2) | 1530.6(1) | 944.4(1) |
| 600.0(1) | 0.89(11)* | 1673.8(1) | 1073.8(1) |
| 603.0(2) | 0.37(4)* | 1547.4(1) | 944.4(1) |
| 621.5(1) | 2.03(15) | 972.6(1) | 351.1(1) |
| 627.2(1) | 2.20(16) | 2009.7(2) | 1382.3(1) |
| 630.8(1) | 0.23(3)* | 2418.2(2) | 1787.2(1) |
| 637.7(1) | 2.0(2)* | 972.6(1) | 335.0(1) |
| 642.2(2) | 0.91(17)* | 1766.1(1) | 1123.9(1) |
| 644.0(4) | 0.16(6)* | 2151.5(4) | 1507.4(1) |
| 644.7(2) | 0.29(6)* | 1718.5(1) | 1073.8(1) |
| 656.1(2) | 0.17(6)* | 2186.7(2) | 1530.6(1) |
| 660.4(2) | 0.21(3)* | 2447.9(2) | 1787.2(1) |
| 661.4(2) | 0.24(8)* | 2192.1(2) | 1530.6(1) |
| 663.1(3) | 0.31(8)* | 1787.2(1) | 1123.9(1) |
| 668.4(2) | 0.23(5)* | 1963.5(1) | 1295.0(1) |
| 677.2(2) | 0.21(4)* | 2059.4(1) | 1382.3(1) |
| 681.7(1) | 1.01(9) | 2447.9(2) | 1766.1(1) |
| 683.1(1) | 3.0(2) | 1295.0(1) | 612.0(1) |
| 689.7(1) | 2.40(17) | 1984.9(1) | 1295.0(1) |
| 696.7(1) | 0.76(6) | 1820.7(1) | 1123.9(1) |
| 701.3(1) | 2.0(15)* | 1673.8(1) | 972.6(1) |
| 704.2(2) | 0.051(9) | 2235.3(2) | 1530.6(1) |
| 711.9(3) | 0.27(10)* | 2242.6(3) | 1530.6(1) |
| 713.5(1) | 3.1(3)* | 1787.2(1) | 1073.8(1) |
| 722.7(1) | 5.2(4) | 1073.8(1) | 351.1(1) |
| 726.1(1) | 0.37(3) | 1849.9(2) | 1123.9(1) |
| 729.7(2) | 0.27(5)* | 2237.2(2) | 1507.4(1) |
| 729.8(2) | 0.31(10)* | 2447.9(2) | 1718.5(1) |
| 741.5(2) | 0.78(13)* | 2036.5(2) | 1295.0(1) |
| 744.7(2) | 0.58(14)* | 2418.2(2) | 1673.8(1) |
| 745.9(2) | 0.28(8)* | 2276.5(2) | 1530.6(1) |
| 747.5(1) | 10.1(7) | 1295.0(1) | 547.6(1) |
| 753.1(2) | 0.26(7)* | 2283.7(2) | 1530.6(1) |
| 757.3(2) | 0.22(5)* | 2139.6(2) | 1382.3(1) |
| 764.2(2) | 0.37(6)* | 2059.4(1) | 1295.0(1) |
| 770.2(1) | 6.6(5)* | 1382.3(1) | 612.0(1) |
| 772.8(1) | 6.1(4)* | 1123.9(1) | 351.1(1) |
| 774.3(2) | 0.47(13)* | 2447.9(2) | 1673.8(1) |
| 791.4(2) | 0.11(3)* | 2173.7(2) | 1382.3(1) |
| 806.5(1) | 0.28(2) | 2480.3(1) | 1673.8(1) |
| 813.1(1) | 0.96(10)* | 2108.2(1) | 1295.0(1) |
| 816.0(1) | 1.71(12) | 1760.6(1) | 944.4(1) |
| 819.8(2) | 0.21(5)* | 2586.1(2) | 1766.1(1) |
| 826.9(1) | 0.29(2) | 2357.5(1) | 1530.6(1) |
| 834.2(2) | 0.38(7)* | 2341.9(1) | 1507.4(1) |
| 839.6(1) | 0.93(7) | 1963.5(1) | 1123.9(1) |
| 843.7(1) | 0.97(7) | 2138.8(1) | 1295.0(1) |
| 849.9(1) | 0.197(18) | 1794.3(1) | 944.4(1) |
| 853.1(1) | 0.78(6) | 2235.3(2) | 1382.3(1) |
| 858.7(1) | 0.53(4) | 1932.6(1) | 1073.8(1) |
| 861.0(1) | 5.1(4) | 1984.9(1) | 1123.9(1) |
| 866.9(1) | 0.30(2) | 2161.9(1) | 1295.0(1) |
| 876.6(3) | 0.31(7)* | 1820.7(1) | 944.4(1) |
| 878.3(5) | 0.09(5)* | 2173.7(2) | 1295.0(1) |
| 886.0(1) | 0.81(9)* | 2009.7(2) | 1123.9(1) |
| 889.2(1) | 0.96(12)* | 1962.9(1) | 1073.8(1) |
| 910.9(1) | 0.53(8)* | 2418.2(2) | 1507.4(1) |
| 912.5(1) | 1.65(15)* | 2036.5(2) | 1123.9(1) |
| 918.5(1) | 0.70(5) | 1530.6(1) | 612.0(1) |
| 928.7(1) | 0.62(5) | 2052.8(2) | 1123.9(1) |
| 935.4(2) | 0.74(12)* | 1547.4(1) | 612.0(1) |
| 936.0(2) | 0.58(8)* | 2009.7(2) | 1073.8(1) |
| 940.4(1) | 0.57(8)* | 2447.9(2) | 1507.4(1) |
| 943.9(1) | < 0.074[2] | 1295.0(1) | 351.1(1) |
| 951.5(1) | 0.29(3) | 2025.4(1) | 1073.8(1) |
| 959.8(1) | 1.40(14)* | 1507.4(1) | 547.6(1) |
| 959.9(3) | 0.17(5)* | 2341.9(1) | 1382.3(1) |
| 972.6(1) | < 0.080[2] | 972.6(1) | 0.0 |
| 978.0(5) | 0.13(6)* | 2360.3(5) | 1382.3(1) |
| 979.3(2) | 0.50(8)* | 2052.8(2) | 1073.8(1) |
| 1012.3(1) | 0.25(2) | 2686.4(2) | 1673.8(1) |
| 1019.4(1) | 0.096(10) | 1964.0(2) | 944.4(1) |
| 1028.3(1) | 0.82(6) | 2152.2(1) | 1123.9(1) |
| 1036.0(1) | 0.57(4) | 2418.2(2) | 1382.3(1) |
| 1040.7(3) | 0.18(9)* | 1984.9(1) | 944.4(1) |
| 1046.7(1) | 1.13(8) | 2341.9(1) | 1295.0(1) |
| 1059.1(3) | 0.13(5)* | 2354.1(4) | 1295.0(1) |
| 1060.6(3) | 0.19(6)* | 2004.9(1) | 944.4(1) |
| 1066.1(4) | 0.14(6)* | 2447.9(2) | 1382.3(1) |
| 1069.1(2) | 0.13(3)* | 2616.5(2) | 1547.4(1) |
| 1092.2(1) | 0.200(17) | 2036.5(2) | 944.4(1) |
| 1106.7(3) | 0.20(8)* | 2464.2(3) | 1357.5(1) |
| 1123.0(2) | 0.35(5)* | 2418.2(2) | 1295.0(1) |
| 1138.4(2) | 0.082(11) | 2645.9(2) | 1507.4(1) |
| 1154.2(1) | 1.30(14)* | 1766.1(1) | 612.0(1) |
| 1156.4(1) | 2.4(2)* | 1507.4(1) | 351.1(1) |
| 1171.0(1) | 1.04(8) | 1718.5(1) | 547.6(1) |
| 1182.3(2) | 0.49(8)* | 1794.3(1) | 612.0(1) |
| 1196.3(1) | 1.38(10) | 1547.4(1) | 351.1(1) |
| 1208.7(1) | 0.74(5) | 1820.7(1) | 612.0(1) |
| 1217.9(1) | 2.5(2)* | 2341.9(1) | 1123.9(1) |
| 1245.2(4) | 0.11(4)* | 2369.6(2) | 1123.9(1) |

| $E_\gamma$ (keV) | $I_\gamma$ | $E_i$ (keV) | $E_f$ (keV) |
|---|---|---|---|
| 1257.2(4) | 0.09(4)* | 2381.1(4) | 1123.9(1) |
| 1268.7(1) | 0.24(3) | 1816.3(1) | 547.6(1) |
| 1291.1(4) | 0.049(15) | 2235.3(2) | 944.4(1) |
| 1294.0(1) | 0.93(7) | 2418.2(2) | 1123.9(1) |
| 1296.8(1) | 0.32(3) | 2241.2(2) | 944.4(1) |
| 1324.2(2) | 0.39(7)* | 2447.9(2) | 1123.9(1) |
| 1341.0(1) | 0.57(4) | 2285.5(1) | 944.4(1) |
| 1352.0(1) | 0.114(12) | 1964.0(2) | 612.0(1) |
| 1360.5(1) | 0.38(3) | 2304.9(1) | 944.4(1) |
| 1363.3(2) | 0.058(10) | 2307.7(3) | 944.4(1) |
| 1367.2(5) | 0.13(5)* | 1718.5(1) | 351.1(1) |
| 1372.8(1) | 1.45(10) | 1984.9(1) | 612.0(1) |
| 1391.6(6) | 0.06(3)* | 2686.4(2) | 1295.0(1) |
| 1397.4(1) | 2.16(15) | 2341.9(1) | 944.4(1) |
| 1413.4(1) | 0.50(4) | 2025.4(1) | 612.0(1) |
| 1424.9(2) | 0.52(12)* | 2036.5(2) | 612.0(1) |
| 1425.2(3) | 0.15(3)* | 2369.6(2) | 944.4(1) |
| 1434.1(1) | 0.36(3) | 2378.5(1) | 944.4(1) |
| 1440.7(1) | 0.44(3) | 2052.8(2) | 612.0(1) |
| 1447.2(1) | 0.64(5) | 2391.7(1) | 944.4(1) |
| 1462.5(5) | 0.13(6)* | 2586.1(2) | 1123.9(1) |
| 1473.9(1) | 1.70(12) | 2418.2(2) | 944.4(1) |
| 1482.7(1) | 0.176(14) | 2990.1(1) | 1507.4(1) |
| 1487.0(1) | 0.093(9) | 2099.0(2) | 612.0(1) |
| 1504.7(8) | 0.10(5)* | 2447.9(2) | 944.4(1) |
| 1509.4(1) | 0.66(5) | 2121.4(1) | 612.0(1) |
| 1535.8(1) | 0.30(3) | 2480.3(1) | 944.4(1) |
| 1549.8(1) | 0.32(3) | 2097.3(1) | 547.6(1) |
| 1557.0(1) | 0.37(3) | 2501.4(1) | 944.4(1) |
| 1562.4(1) | 0.26(2) | 2686.4(2) | 1123.9(1) |
| 1575.7(1) | 0.217(18) | 2187.7(1) | 612.0(1) |
| 1604.3(1) | 0.189(16) | 2548.8(2) | 944.4(1) |
| 1620.5(1) | 0.132(12) | 2565.0(2) | 944.4(1) |
| 1629.7(1) | 0.22(2) | 2574.2(1) | 944.4(1) |
| 1673.4(1) | 0.66(5) | 2285.5(1) | 612.0(1) |
| 1742.2(1) | 0.34(3) | 2686.4(2) | 944.4(1) |
| 1745.5(1) | 0.220(17) | 2357.5(1) | 612.0(1) |
| 1757.7(1) | 0.26(2) | 2369.6(2) | 612.0(1) |
| 1767.5(1) | 0.178(15) | 2712.0(2) | 944.4(1) |
| 1778.1(5) | 0.08(5) | 2722.6(5) | 944.4(1) |
| 1779.8(1) | 0.71(7) | 2391.7(1) | 612.0(1) |
| 1806.2(1) | 1.88(14) | 2418.2(2) | 612.0(1) |
| 1823.7(1) | 0.140(12) | 2768.1(2) | 944.4(1) |
| 1835.9(1) | 4.3(3) | 2447.9(2) | 612.0(1) |
| 1889.4(1) | 0.47(4) | 2501.4(1) | 612.0(1) |
| 1952.0(1) | 2.04(15) | 2564.0(1) | 612.0(1) |
| 1974.2(1) | 0.47(4) | 2586.1(2) | 612.0(1) |
| 2021.4(1) | 0.39(3) | 2633.4(1) | 612.0(1) |
| 2099.2(1) | 0.230(19) | 2711.2(1) | 612.0(1) |
| 2132.0(2) | 0.16(2) | 2744.0(2) | 612.0(1) |

[1] Not observed directly.

[2] Limit given in 95% credible interval.

TABLE III: Transition properties obtained in the present work for $^{184}$Hg. Level energies, spins and parities of the initial ($E_i$, $J_i^\pi$) and final ($E_f$, $J_f^\pi$) states, transition energies ($E_t$) and $\gamma$-branching ratios ($Br_\gamma$) have been listed. Pure $E0$ transitions are written in italics. The spins and parities are taken from this work and Refs. [2, 3].

| $E_i$ (keV) | $J_i^\pi$ | $E_f$ (keV) | $J_f^\pi$ | $E_\gamma$ (keV) | $Br_\gamma$ |
|---|---|---|---|---|---|
| 366.9(1) | $2^+$ | 0.0 | $0^+$ | 366.9(1) | 100 |
| 375.4(1) | $0^+$ | 366.9(1) | $2^+$ | 8.5(2) | 5.9(12)[1] |

*Continued Table III*

| $E_i$ (keV) | $J_i^\pi$ | $E_f$ (keV) | $J_f^\pi$ | $E_\gamma$ (keV) | $Br_\gamma$ |
|---|---|---|---|---|---|
| | $0^+$ | 0.0 | $0^+$ | *375.4(1)* | *100* |
| 534.8(1) | $2^+$ | 0.0 | $0^+$ | 534.8(1) | 100(5) |
| | | 366.9(1) | $2^+$ | 168.0(1) | 8.0(11)* |
| | | 375.4(1) | $0^+$ | 159.4(1) | 3.2(3)* |
| 654.0(1) | $4^+$ | 366.9(1) | $2^+$ | 287.1(1) | 100(5) |
| | | 534.8(1) | $2^+$ | 119.2(2) | <0.6[3] |
| 983.5(1) | $2^+$ | 0.0 | $0^+$ | 983.5(1) | < 11.7[4] |
| | | 366.9(1) | $2^+$ | 616.6(1) | 100(5) |
| | | 375.4(1) | $0^+$ | 608.2(1) | 91(7) |
| | | 534.8(1) | $2^+$ | 448.7(1) | <3.7[2] |
| 994.2(1) | $6^+$ | 654.0(1) | $4^+$ | 340.3(1) | 100 |
| 1086.6(1) | $4^+$ | 366.9(1) | $2^+$ | 719.6(1) | 68(5) |
| | | 534.8(1) | $2^+$ | 551.9(1) | 100(5) |
| | | 654.0(1) | $4^+$ | 432.8(2) | 20(2)* |
| 1089.0(2) | $(3)^+$ | 366.9(1) | $2^+$ | 722.0(1) | 42(3) |
| | | 534.8(1) | $2^+$ | 554.4(1) | 100(5) |
| | | 654.0(1) | $4^+$ | 435.1(2) | 17.1(18)* |
| 1123.9(2) | $0^+$ | 534.8(1) | $2^+$ | 589.1(2) | 100(15)* |
| | | 375.4(1) | $0^+$ | *748.5(2)* | *4.5(14)*[5] |
| 1178.8(2) | $2^+$ | 0.0 | $0^+$ | 1179.2(5) | 58(7)[6] |
| | | 366.9(1) | $2^+$ | 812.2(2) | 19(4)* |
| | | 375.4(1) | $0^+$ | 803.3(1) | 29(2) |
| | | 534.8(1) | $2^+$ | 643.9(1) | 100(5) |
| 1300.2(1) | $4^+$ | 366.9(1) | $2^+$ | 933.3(2) | < 10.2[4] |
| | | 534.8(1) | $2^+$ | 765.3(1) | 100(8)[6] |
| | | 654.0(1) | $4^+$ | 646.3(1) | 67(6) |
| | | 983.5(1) | $2^+$ | 316.6(3) | 6.2(24)* |
| | | 1086.6(1) | $4^+$ | 213.6(2) | <5.4[2] |
| 1412.7(1) | $8^+$ | 994.2(1) | $6^+$ | 418.5(1) | 100 |
| 1413.3(1) | $(5^+)$ | 654.0(1) | $4^+$ | 759.3(1) | 100(5)* |
| | | 1089.0(2) | $(3)^+$ | 324.4(1) | 22.8(17) |
| 1445.0(1) | | 366.9(1) | $2^+$ | 1078.1(1) | 100 |
| 1449.6(1) | | 0.0 | $0^+$ | 1449.7(1)[7] | 14.9(18) |
| | | 366.9(1) | $2^+$ | 1082.7(2) | 24(5)[6] |
| | | 534.8(1) | $2^+$ | 914.8(1) | 100(9)* |
| 1463.8(4) | | 366.9(1) | $2^+$ | 1096.2(5) | 100(41)* |
| | | 375.4(1) | $0^+$ | 1088.6(2) | 68(32) |
| 1513.8(1) | | 534.8(1) | $2^+$ | 979.0(1) | 100 |
| 1549.6(2) | $6^+$ | 654.0(1) | $4^+$ | 895.4(1) | 28.9(28) |
| | | 994.2(1) | $6^+$ | 555.5(1) | 100(8)* |
| | | 1086.6(1) | $4^+$ | 462.9(1) | 99(9) |
| 1557.4(1) | | 366.9(1) | $2^+$ | 1190.5(1) | 100(5) |
| | | 534.8(1) | $2^+$ | 1022.4(3) | 41(10)* |
| | | 983.5(1) | $2^+$ | 573.9(3) | 20(5)* |
| 1603.0(1) | | 366.9(1) | $2^+$ | 1236.1(1) | 100(9) |
| | | 375.4(1) | $0^+$ | 1227.7(1) | 38(5)* |
| | | 534.8(1) | $2^+$ | 1068.1(1) | 53(6) |
| 1658.4(1) | | 983.5(1) | $2^+$ | 674.8(1) | 100(5) |
| | | 1089.0(2) | $(3)^+$ | 569.6(3) | 58(13)* |
| 1665.3(2) | | 366.9(1) | $2^+$ | 1298.4(2) | 100 |
| 1705.8(2) | | 366.9(1) | $2^+$ | 1338.9(1) | 95(17) |
| | | 534.8(1) | $2^+$ | 1170.7(2) | 100(17)* |
| | | 1178.8(2) | $2^+$ | 527.3(3) | 75(23)* |
| 1737.7(2) | | 366.9(1) | $2^+$ | 1370.9(5) | 70(20)* |
| | | 534.8(1) | $2^+$ | 1203.0(5) | 37(13)* |
| | | 983.5(1) | $2^+$ | 754.1(2) | 100(15)* |
| 1790.2(3) | | 375.4(1) | $0^+$ | 1414.7(3) | 100 |
| 1792.7(2) | | 366.9(1) | $2^+$ | 1425.8(2) | 100 |
| 1794.0(3) | | 654.0(1) | $4^+$ | 1140.0(2) | 100 |
| 1803.3(1) | $(7^+)$ | 994.2(1) | $6^+$ | 809.1(1) | 100(5) |

*Continued Table III*

| $E_i$ (keV) | $J_i^\pi$ | $E_f$ (keV) | $J_f^\pi$ | $E_\gamma$ (keV) | $Br_\gamma$ |
|---|---|---|---|---|---|
| | | 1412.7(1) | $8^+$ | 390.3(3) | 25(7)* |
| | | 1413.3(1) | $(5^+)$ | 389.9(1) | 60(10)* |
| 1804.6(1) | | 366.9(1) | $2^+$ | 1437.7(1) | 44(4) |
| | | 534.8(1) | $2^+$ | 1269.7(1) | 100(5) |
| | | 983.5(1) | $2^+$ | 821.0(2) | 51(12)* |
| 1817.3(2) | $(5,6^+)$ | 654.0(1) | $4^+$ | 1163.2(4) | 23(7)* |
| | | 994.2(1) | $6^+$ | 823.2(2) | 28(7)* |
| | | 1086.6(1) | $4^+$ | 730.7(1) | 100(12)* |
| | | 1300.2(1) | $4^+$ | 516.6(3) | 38(10)* |
| 1824.9(2) | | 1089.0(2) | $(3)^+$ | 735.9(1) | 100 |
| 1832.6(1) | | 366.9(1) | $2^+$ | 1465.6(1) | 100(5) |
| | | 654.0(1) | $4^+$ | 1178.7(6) | 30(16)* |
| | | 1178.8(2) | $2^+$ | 653.8(4) | 22(8)* |
| 1847.7(1) | 5 | 654.0(1) | $4^+$ | 1193.7(1) | 97(23) |
| | | 1086.6(1) | $4^+$ | 760.8(3) | 100(23)* |
| | | 1300.2(1) | $4^+$ | 547.6(2) | 81(23)* |
| 1854.3(2) | | 1089.0(2) | $(3)^+$ | 765.4(1) | 100(15)* |
| | | 1413.3(1) | $(5^+)$ | 440.5(4) | 10.6(47)* |
| 1862.4(1) | | 534.8(1) | $2^+$ | 1327.6(1) | 100 |
| 1871.7(1) | | 994.2(1) | $6^+$ | 877.4(1) | 100 |
| 1901.7(1) | $10^+$ | 1412.7(1) | $8^+$ | 489.0(1) | 100 |
| 1910.0(3) | | 983.5(1) | $2^+$ | 926.8(4) | 91(47)* |
| | | 1086.6(1) | $4^+$ | 823.2(3) | 100(40)* |
| 1929.1(2) | | 366.9(1) | $2^+$ | 1562.2(1) | 100(8) |
| | | 983.5(1) | $2^+$ | 945.4(3) | 62(17)* |
| 1930.6(2) | | 1086.6(1) | $4^+$ | 843.9(2) | 100 |
| 1938.1(3) | | 1086.6(1) | $4^+$ | 851.5(3) | 100 |
| 1948.5(4) | | 654.0(1) | $4^+$ | 1294.7(6) | 100(31)* |
| | | 983.5(1) | $2^+$ | 964.8(5) | 73(36)* |
| 1969.1(2) | | 1549.6(2) | $6^+$ | 419.5(1) | 100 |
| 1991.5(2) | | 1086.6(1) | $4^+$ | 904.8(1) | 100 |
| 1992.4(3) | | 1300.2(1) | $4^+$ | 692.2(3) | 100 |
| 2008.6(5) | | 654.0(1) | $4^+$ | 1354.6(5) | 100 |
| 2035.7(2) | | 0.0 | $0^+$ | 2035.6(1)[7] | 100(8) |
| | | 375.4(1) | $0^+$ | 1660.3(2) | 30(4) |
| 2050.9(2) | | 1086.6(1) | $4^+$ | 964.3(2) | 100 |
| 2054.4(3) | | 1300.2(1) | $4^+$ | 754.2(2) | 100 |
| 2057.9(4) | | 366.9(1) | $2^+$ | 1691.0(4) | 100 |
| 2061.2(5) | | 1089.0(2) | $(3)^+$ | 972.2(5) | 100 |
| 2063.7(2) | (6) | 1413.3(1) | $(5^+)$ | 650.3(1) | 100 |
| 2064.2(3) | | 654.0(1) | $4^+$ | 1410.2(3) | 100 |
| 2066.9(2) | | 654.0(1) | $4^+$ | 1412.9(2) | 100(23)* |
| | | 994.2(1) | $6^+$ | 1072.9(4) | 89(38)* |
| 2071.8(1) | | 534.8(1) | $2^+$ | 1536.9(1) | 100 |
| 2072.4(2) | | 1300.2(1) | $4^+$ | 772.1(2) | 100(19)* |
| | | 1413.3(1) | $(5^+)$ | 659.0(2) | 75(21)* |
| | | 1549.6(2) | $6^+$ | 523.3(3) | 52(22)* |
| 2080.1(2) | | 366.9(1) | $2^+$ | 1713.2(2) | 100 |
| 2083.0(1) | | 534.8(1) | $2^+$ | 1548.1(1) | 100(6) |
| | | 1178.8(2) | $2^+$ | 904.4(5) | 25(11)* |
| 2093.0(2) | | 0.0 | $0^+$ | 2093.1(2)[7] | 100(14) |
| | | 375.4(1) | $0^+$ | 1717.6(1) | 59(10) |
| 2096.6(3) | | 375.4(1) | $0^+$ | 1721.2(3) | 100 |
| 2106.5(2) | | 654.0(1) | $4^+$ | 1452.5(2) | 100 |
| 2121.3(2) | 7 | 1412.7(1) | $8^+$ | 708.5(2) | 100(22)* |
| | | 1549.6(2) | $6^+$ | 571.8(2) | 40(13)* |
| | | 1817.3(2) | $(5,6^+)$ | 304.2(1) | 51(12) |
| 2143.7(3) | | 366.9(1) | $2^+$ | 1776.8(3) | 100 |
| 2145.2(2) | | 1086.6(1) | $4^+$ | 1058.5(1) | 100 |
| 2149.6(1) | | 654.0(1) | $4^+$ | 1495.6(1) | 100 |

*Continued Table III*

| $E_i$ (keV) | $J_i^\pi$ | $E_f$ (keV) | $J_f^\pi$ | $E_\gamma$ (keV) | $Br_\gamma$ |
|---|---|---|---|---|---|
| 2156.8(2) | | 534.8(1) | $2^+$ | 1621.9(1) | 100(11) |
| | | 1300.2(1) | $4^+$ | 857.1(4) | 45(20)* |
| 2180.8(3) | | 366.9(1) | $2^+$ | 1813.9(3) | 100 |
| 2192.4(2) | | 366.9(1) | $2^+$ | 1825.5(2) | 100 |
| 2193.4(3) | | 1086.6(1) | $4^+$ | 1106.7(3) | 100 |
| 2195.8(3) | | 994.2(1) | $6^+$ | 1201.6(3) | 100 |
| 2216.3(4) | | 1549.6(2) | $6^+$ | 666.7(4) | 100 |
| 2239.3(2) | | 366.9(1) | $2^+$ | 1872.1(3) | 41(12) |
| | | 375.4(1) | $0^+$ | 1864.0(2) | 100(10) |
| 2242.4(1) | | 654.0(1) | $4^+$ | 1588.4(1) | 100 |
| 2248.8(2) | | 1413.3(1) | $(5^+)$ | 835.3(2) | 66(8) |
| | | 1549.6(2) | $6^+$ | 699.4(1) | 100(7) |
| 2257.1(3) | $(9^+)$ | 1412.7(1) | $8^+$ | 844.3(4) | 100(38)* |
| | | 1803.3(1) | $(7^+)$ | 453.9(3) | 51(29)* |
| 2267.2(2) | | 994.2(1) | $6^+$ | 1273.0(2) | 100 |
| 2270.1(3) | | 1817.3(2) | $(5,6^+)$ | 452.8(2) | 100 |
| 2271.7(2) | | 654.0(1) | $4^+$ | 1617.8(1) | 100(8) |
| | | 994.2(1) | $6^+$ | 1276.9(3) | 70(19)* |
| 2291.6(2) | | 994.2(1) | $6^+$ | 1297.0(3) | 27(9)* |
| | | 1412.7(1) | $8^+$ | 879.0(1) | 100(7) |
| | | 2072.4(2) | | 219.1(2) | 64(19)* |
| 2309.3(2) | | 0.0 | $0^+$ | 2309.3(2)[7] | 100(10) |
| | | 366.9(1) | $2^+$ | 1942.4(1) | 99(15) |
| | | 375.4(1) | $0^+$ | 1934.2(3) | 10.0(36)* |
| 2328.8(2) | | 994.2(1) | $6^+$ | 1334.5(1) | 97(28) |
| | | 1412.7(1) | $8^+$ | 916.3(2) | 100(28)* |
| 2330.1(1) | | 983.5(1) | $2^+$ | 1346.6(1) | 100 |
| 2344.1(4) | | 534.8(1) | $2^+$ | 1809.0(4) | 100(37)* |
| | | 654.0(1) | $4^+$ | 1690.8(7) | 61(35)* |
| 2349.8(5) | | 1413.3(1) | $(5^+)$ | 936.5(5) | 100 |
| 2357.9(3) | | 375.4(1) | $0^+$ | 1982.5(3) | 100 |
| 2373.7(8) | | 983.5(1) | $2^+$ | 1390.2(8) | 100 |
| 2374.7(4) | (8) | 1412.7(1) | $8^+$ | 961.6(4) | 47(22)* |
| | | 1803.3(1) | $(7^+)$ | 571.3(2) | 100(21)* |
| | | 2063.7(2) | (6) | 311.6(3) | 51(17)* |
| 2380.5(1) | | 366.9(1) | $2^+$ | 2013.6(1) | 100 |
| 2383.3(3) | | 994.2(1) | $6^+$ | 1389.1(3) | 100 |
| 2387.2(2) | | 1412.7(1) | $8^+$ | 974.5(2) | 100 |
| 2404.3(2) | | 1412.7(1) | $8^+$ | 991.6(2) | 100 |
| 2417.1(1) | | 534.8(1) | $2^+$ | 1882.3(1) | 100 |
| 2429.5(1) | | 1412.7(1) | $8^+$ | 1016.8(1) | 100 |
| 2449.1(6) | | 366.9(1) | $2^+$ | 2082.2(6) | 100 |
| 2494.7(3) | | 1412.7(1) | $8^+$ | 1082.0(3) | 100 |
| 2502.2(3) | | 994.2(1) | $6^+$ | 1508.0(3) | 100 |
| 2509.6(2) | | 994.2(1) | $6^+$ | 1515.3(2) | 100 |
| 2543.5(1) | | 654.0(1) | $4^+$ | 1889.5(1) | 100 |
| 2548.3(2) | | 1412.7(1) | $8^+$ | 1135.6(2) | 100 |
| 2563.4(1) | | 1412.7(1) | $8^+$ | 1150.7(1) | 100 |
| 2569.0(4) | | 366.9(1) | $2^+$ | 2202.1(4) | 100 |
| 2627.7(2) | | 375.4(1) | $0^+$ | 2252.3(2) | 100 |
| 2642.5(4) | | 654.0(1) | $4^+$ | 1988.5(4) | 100 |
| 2664.6(3) | | 994.2(1) | $6^+$ | 1670.3(3) | 100 |
| 2673.4(1) | | 1412.7(1) | $8^+$ | 1260.7(1) | 100 |
| 2703.5(3) | | 1412.7(1) | $8^+$ | 1290.8(3) | 100 |
| 2735.8(3) | | 983.5(1) | $2^+$ | 1752.2(3) | 100 |
| 2817.6(4) | | 375.4(1) | $0^+$ | 2442.2(4) | 100 |
| 2832.8(4) | | 375.4(1) | $0^+$ | 2457.4(4) | 100 |
| 3015.7(1) | | 1412.7(1) | $8^+$ | 1603.0(1) | 100 |

*Continued Table III*

| $E_i$ (keV) | $J_i^\pi$ | $E_f$ (keV) | $J_f^\pi$ | $E_\gamma$ (keV) | $Br_\gamma$ |
|---|---|---|---|---|---|

[1] Total transition intensity relative to the total intensity of the 375-keV $E0$ transition, see text for details.
[2] Observed only as conversion electrons, $\gamma$-branching ratio limits given with 95% credible interval.
[3] Intensity obtained from singles after subtracting the contribution from daughter activities, see text for details.
[4] $\gamma$ ray not observed, upper limit, given within 95% credible interval, obtained from the $\gamma$-$\gamma$ coincidence data.
[5] Total electron intensity relative to the 589 keV $\gamma$-ray transition intensity, see text for details.
[6] Intensity determined as a difference between singles and gated spectrum, see text for details.
[7] Not included in the level energy determination.

TABLE IV: The relative $\gamma$-ray intensities in $^{184}$Hg, normalized to the strongest $2_1^+ \rightarrow 0_1^+$ 367 keV transition. The intensities of transitions marked with * were determined from coincidences.

| $E_\gamma$ (keV) | $I_\gamma$ | $E_i$ (keV) | $E_f$ (keV) |
|---|---|---|---|
| 8.5(2)[1] | $2.4(9) \times 10^{-6}$ | 375.4(1) | 366.9(1) |
| 119.2(2) | < 0.22[2] | 654.0(1) | 534.8(1) |
| 159.4(1) | 0.48(5)* | 534.8(1) | 375.4(1) |
| 168.0(1) | 1.20(17)* | 534.8(1) | 366.9(1) |
| 213.6(2) | <0.17[2] | 1300.2(1) | 1086.6(1) |
| 219.1(2) | 0.39(11)* | 2291.6(2) | 2072.4(2) |
| 287.1(1) | 39(3) | 654.0(1) | 366.9(1) |
| 304.2(1) | 0.30(4) | 2121.3(2) | 1817.3(2) |
| 311.6(3) | 0.10(3)* | 2374.7(4) | 2063.7(2) |
| 316.6(3) | 0.19(7)* | 1300.2(1) | 983.5(1) |
| 324.4(1) | 0.94(7) | 1413.3(1) | 1089.0(2) |
| 340.3(1) | 19.8(14) | 994.2(1) | 654.0(1) |
| 366.9(1) | 100 | 366.9(1) | 0.0 |
| 375.4(1) | 10.1(7)[3] | 375.4(1) | 0.0 |
| 389.9(1) | 0.90(15)* | 1803.3(1) | 1413.3(1) |
| 390.3(3) | 0.38(10)* | 1803.3(1) | 1412.7(1) |
| 418.5(1) | 7.8(7)* | 1412.7(1) | 994.2(1) |
| 419.5(1) | 0.84(12)* | 1969.1(2) | 1549.6(2) |
| 432.8(2) | 1.23(13)* | 1086.6(1) | 654.0(1) |
| 435.1(2) | 1.27(13)* | 1089.0(2) | 654.0(1) |
| 440.5(4) | 0.09(4)* | 1854.3(2) | 1413.3(1) |
| 448.7(1) | <0.19[2] | 983.5(1) | 534.8(1) |
| 452.8(2) | 0.37(14)* | 2270.1(3) | 1817.3(2) |
| 453.9(3) | 0.08(3)* | 2257.1(3) | 1803.3(1) |
| 462.9(1) | 2.4(2) | 1549.6(2) | 1086.6(1) |
| 489.0(1) | 0.38(3) | 1901.7(1) | 1412.7(1) |
| 516.6(3) | 0.35(9)* | 1817.3(2) | 1300.2(1) |
| 523.3(3) | 0.13(5)* | 2072.4(2) | 1549.6(2) |
| 527.3(3) | 0.40(10)* | 1705.8(2) | 1178.8(2) |
| 534.8(1) | 15.0(11) | 534.8(1) | 0.0 |
| 547.6(2) | 0.32(6)* | 1847.7(1) | 1300.2(1) |
| 551.9(1) | 6.1(4) | 1086.6(1) | 534.8(1) |
| 554.4(1) | 7.4(5) | 1089.0(2) | 534.8(1) |
| 555.5(1) | 2.4(2)* | 1549.6(2) | 994.2(1) |
| 569.6(3) | 0.44(10)* | 1658.4(1) | 1089.0(2) |
| 571.3(2) | 0.20(4)* | 2374.7(4) | 1803.3(1) |
| 571.8(2) | 0.24(6)* | 2121.3(2) | 1549.6(2) |
| 573.9(3) | 0.30(8)* | 1557.4(1) | 983.5(1) |
| 589.1(2) | 1.03(16)* | 1123.9(2) | 534.8(1) |
| 608.2(1) | 4.8(3) | 983.5(1) | 375.4(1) |
| 616.6(1) | 5.3(4) | 983.5(1) | 366.9(1) |
| 643.9(1) | 2.3(2) | 1178.8(2) | 534.8(1) |
| 646.3(1) | 2.09(15) | 1300.2(1) | 654.0(1) |
| 650.3(1) | 0.59(9) | 2063.7(2) | 1413.3(1) |
| 653.8(4) | 0.18(7)* | 1832.6(1) | 1178.8(2) |
| 659.0(2) | 0.19(4)* | 2072.4(2) | 1413.3(1) |
| 666.7(4) | 0.20(6)* | 2216.3(4) | 1549.6(2) |
| 674.8(1) | 0.76(6) | 1658.4(1) | 983.5(1) |
| 692.2(3) | 0.10(3)* | 1992.4(3) | 1300.2(1) |
| 699.4(1) | 0.30(3) | 2248.8(2) | 1549.6(2) |
| 708.5(2) | 0.59(13)* | 2121.3(2) | 1412.7(1) |
| 719.6(1) | 4.2(3) | 1086.6(1) | 366.9(1) |
| 722.0(1) | 3.1(2) | 1089.0(2) | 366.9(1) |
| 730.7(1) | 0.92(12)* | 1817.3(2) | 1086.6(1) |
| 735.9(1) | 1.09(16)* | 1824.9(2) | 1089.0(2) |
| 748.5(2) | 0.038(10)[3] | 1123.9(2) | 375.4(1) |
| 754.1(2) | 0.65(10)* | 1737.7(2) | 983.5(1) |
| 754.2(2) | 0.23(5)* | 2054.4(3) | 1300.2(1) |
| 759.3(1) | 4.1(3)* | 1413.3(1) | 654.0(1) |
| 760.8(3) | 0.40(9)* | 1847.7(1) | 1086.6(1) |
| 765.3(1) | 3.1(3)* | 1300.2(1) | 534.8(1) |
| 765.4(1) | 0.89(14)* | 1854.3(2) | 1089.0(2) |
| 772.1(2) | 0.25(5)* | 2072.4(2) | 1300.2(1) |
| 803.3(1) | 0.68(5) | 1178.8(2) | 375.4(1) |
| 809.1(1) | 1.49(11) | 1803.3(1) | 994.2(1) |
| 812.2(2) | 0.43(8)* | 1178.8(2) | 366.9(1) |
| 821.0(2) | 0.28(7)* | 1804.6(1) | 983.5(1) |
| 823.2(3) | 0.18(7)* | 1910.0(3) | 1086.6(1) |
| 823.2(2) | 0.26(6)* | 1817.3(2) | 994.2(1) |
| 835.3(2) | 0.20(2) | 2248.8(2) | 1413.3(1) |
| 843.9(2) | 0.77(12)* | 1930.6(2) | 1086.6(1) |
| 844.3(4) | 0.15(6)* | 2257.1(3) | 1412.7(1) |
| 851.5(3) | 0.36(9)* | 1938.1(3) | 1086.6(1) |
| 857.1(4) | 0.09(4)* | 2156.8(2) | 1300.2(1) |
| 877.4(1) | 0.72(6) | 1871.7(1) | 994.2(1) |
| 879.0(1) | 0.61(5) | 2291.6(2) | 1412.7(1) |
| 895.4(1) | 0.69(5) | 1549.6(2) | 654.0(1) |
| 904.4(5) | 0.14(6)* | 2083.0(1) | 1178.8(2) |
| 904.8(1) | 0.83(11)* | 1991.5(2) | 1086.6(1) |
| 914.8(1) | 1.75(17)* | 1449.6(1) | 534.8(1) |
| 916.3(2) | 0.22(6)* | 2328.8(2) | 1412.7(1) |
| 926.8(4) | 0.17(5)* | 1910.0(3) | 983.5(1) |
| 933.3(2) | < 0.32[2] | 1300.2(1) | 366.9(1) |
| 936.5(5) | 0.09(4)* | 2349.8(5) | 1413.3(1) |
| 945.4(3) | 0.24(6)* | 1929.1(2) | 983.5(1) |
| 961.6(4) | 0.09(4)* | 2374.7(4) | 1412.7(1) |
| 964.3(2) | 0.33(7)* | 2050.9(2) | 1086.6(1) |
| 964.8(5) | 0.13(5)* | 1948.5(4) | 983.5(1) |
| 972.2(5) | 0.07(4)* | 2061.2(5) | 1089.0(2) |
| 974.5(2) | 0.15(5)* | 2387.2(2) | 1412.7(1) |
| 979.0(1) | 0.28(2) | 1513.8(1) | 534.8(1) |
| 983.5(1) | < 0.62[2] | 983.5(1) | 0.0 |
| 991.6(2) | 0.40(9)* | 2404.3(2) | 1412.7(1) |
| 1016.8(1) | 0.142(14) | 2429.5(1) | 1412.7(1) |
| 1022.4(3) | 0.63(15)* | 1557.4(1) | 534.8(1) |
| 1058.5(1) | 0.30(2) | 2145.2(2) | 1086.6(1) |
| 1068.1(1) | 0.33(3) | 1603.0(1) | 534.8(1) |
| 1072.9(4) | 0.18(7)* | 2066.9(2) | 994.2(1) |
| 1078.1(1) | 0.37(3) | 1445.0(1) | 366.9(1) |
| 1082.0(3) | 0.23(7)* | 2494.7(3) | 1412.7(1) |
| 1082.7(2) | 0.42(8)* | 1449.6(1) | 366.9(1) |
| 1088.6(2) | 0.11(3) | 1463.8(4) | 375.4(1) |
| 1096.2(5) | 0.16(7)* | 1463.8(4) | 366.9(1) |
| 1106.7(3) | 0.28(7)* | 2193.4(3) | 1086.6(1) |

| $E_\gamma$ (keV) | $I_\gamma$ | $E_i$ (keV) | $E_f$ (keV) |
|---|---|---|---|
| 1135.6(2) | 0.15(2) | 2548.3(2) | 1412.7(1) |
| 1140.0(2) | 0.47(8)* | 1794.0(3) | 654.0(1) |
| 1150.7(1) | 0.20(2) | 2563.4(1) | 1412.7(1) |
| 1163.2(4) | 0.21(6)* | 1817.3(2) | 654.0(1) |
| 1170.7(2) | 0.54(9)* | 1705.8(2) | 534.8(1) |
| 1178.7(6) | 0.25(14)* | 1832.6(1) | 654.0(1) |
| 1179.2(5) | 1.34(17)* | 1178.8(2) | 0.0 |
| 1190.5(1) | 1.52(11) | 1557.4(1) | 366.9(1) |
| 1193.7(1) | 0.38(3) | 1847.7(1) | 654.0(1) |
| 1201.6(3) | 0.21(6)* | 2195.8(3) | 994.2(1) |
| 1203.0(5) | 0.24(8)* | 1737.7(2) | 534.8(1) |
| 1227.7(1) | 0.24(3)* | 1603.0(1) | 375.4(1) |
| 1236.1(1) | 0.63(6) | 1603.0(1) | 366.9(1) |
| 1260.7(1) | 0.29(2) | 2673.4(1) | 1412.7(1) |
| 1269.7(1) | 0.54(4) | 1804.6(1) | 534.8(1) |
| 1273.0(2) | 0.38(6)* | 2267.2(2) | 994.2(1) |
| 1276.9(3) | 0.21(6)* | 2271.7(2) | 994.2(1) |
| 1290.8(3) | 0.10(4)* | 2703.5(3) | 1412.7(1) |
| 1294.7(6) | 0.17(6)* | 1948.5(4) | 654.0(1) |
| 1297.0(3) | 0.16(6)* | 2291.6(2) | 994.2(1) |
| 1298.4(2) | 0.59(8)* | 1665.3(2) | 366.9(1) |
| 1327.6(1) | 0.27(2) | 1862.4(1) | 534.8(1) |
| 1334.5(1) | 0.21(2) | 2328.8(2) | 994.2(1) |
| 1338.9(1) | 0.51(4) | 1705.8(2) | 366.9(1) |
| 1346.6(1) | 0.18(2) | 2330.1(1) | 983.5(1) |
| 1354.6(5) | 0.07(4)* | 2008.6(5) | 654.0(1) |
| 1370.9(5) | 0.45(11)* | 1737.7(2) | 366.9(1) |
| 1389.1(3) | 0.16(5) * | 2383.3(3) | 994.2(1) |
| 1390.2(8) | 0.20(10)* | 2373.7(8) | 983.5(1) |
| 1410.2(3) | 0.17(4)* | 2064.2(3) | 654.0(1) |
| 1412.9(2) | 0.21(5)* | 2066.9(2) | 654.0(1) |
| 1414.7(3) | 0.07(2)* | 1790.2(3) | 375.4(1) |
| 1425.8(2) | 0.21(5)* | 1792.7(2) | 366.9(1) |
| 1437.7(1) | 0.24(2) | 1804.6(1) | 366.9(1) |
| 1449.7(1) | 0.26(3) | 1449.6(1) | 0.0 |
| 1452.5(2) | 0.122(13) | 2106.5(2) | 654.0(1) |
| 1465.6(1) | 0.83(6) | 1832.6(1) | 366.9(1) |
| 1495.6(1) | 0.58(4) | 2149.6(1) | 654.0(1) |
| 1508.0(3) | 0.18(5)* | 2502.2(3) | 994.2(1) |
| 1515.3(2) | 0.13(3) | 2509.6(2) | 994.2(1) |
| 1536.9(1) | 0.42(3) | 2071.8(1) | 534.8(1) |
| 1548.1(1) | 0.56(4) | 2083.0(1) | 534.8(1) |
| 1562.2(1) | 0.38(3) | 1929.1(2) | 366.9(1) |
| 1588.4(1) | 0.44(4) | 2242.4(1) | 654.0(1) |
| 1603.0(1) | 0.38(3) | 3015.7(1) | 1412.7(1) |
| 1617.8(1) | 0.30(3) | 2271.7(2) | 654.0(1) |
| 1621.9(1) | 0.19(2) | 2156.8(2) | 534.8(1) |
| 1660.3(2) | 0.130(14) | 2035.7(2) | 375.4(1) |
| 1670.3(3) | 0.14(5)* | 2664.6(3) | 994.2(1) |
| 1690.8(7) | 0.15(7)* | 2344.1(4) | 654.0(1) |
| 1691.0(4) | 0.30(9)* | 2057.9(4) | 366.9(1) |
| 1713.2(2) | 0.15(4)* | 2080.1(2) | 366.9(1) |
| 1717.6(1) | 0.138(13) | 2093.0(2) | 375.4(1) |
| 1721.2(3) | 0.07(2)* | 2096.6(3) | 375.4(1) |
| 1752.2(3) | 0.10(4)* | 2735.8(3) | 983.5(1) |
| 1776.8(3) | 0.13(2) | 2143.7(3) | 366.9(1) |
| 1809.0(4) | 0.24(9)* | 2344.1(4) | 534.8(1) |
| 1813.9(3) | 0.23(5)* | 2180.8(3) | 366.9(1) |
| 1825.5(2) | 0.19(2) | 2192.4(2) | 366.9(1) |
| 1864.0(2) | 0.16(2) | 2239.3(2) | 375.4(1) |
| 1872.1(3) | 0.07(2) | 2239.3(2) | 366.9(1) |
| 1882.3(1) | 0.30(3) | 2417.1(1) | 534.8(1) |
| 1889.5(1) | 0.18(3) | 2543.5(1) | 654.0(1) |
| 1934.2(3) | 0.036(13)* | 2309.3(2) | 375.4(1) |
| 1942.4(1) | 0.36(4) | 2309.3(2) | 366.9(1) |
| 1982.5(3) | 0.09(2)* | 2357.9(3) | 375.4(1) |
| 1988.5(4) | 0.10(5)* | 2642.5(4) | 654.0(1) |
| 2013.6(1) | 0.25(3) | 2380.5(1) | 366.9(1) |
| 2035.6(1) | 0.44(4) | 2035.7(2) | 0.0 |
| 2082.2(6) | 0.25(10)* | 2449.1(6) | 366.9(1) |
| 2093.1(2) | 0.23(4) | 2093.0(2) | 0.0 |
| 2202.1(4) | 0.25(6) | 2569.0(4) | 366.9(1) |
| 2252.3(2) | 0.16(2) | 2627.7(2) | 375.4(1) |
| 2309.3(2) | 0.36(4) | 2309.3(2) | 0.0 |
| 2442.2(4) | 0.047(14)* | 2817.6(4) | 375.4(1) |
| 2457.4(4) | 0.044(13)* | 2832.8(4) | 375.4(1) |

[1] Not observed directly.

[2] Limit given in 95% credible interval.

[3] $E0$ transition. The intensity of K electrons was multiplied by a factor 1.2 to account for other shells.

TABLE V: Transition properties obtained in the present work for $^{186}$Hg. Level energies, spins and parities of the initial ($E_i$, $J_i^\pi$) and final ($E_f$, $J_f^\pi$) states, transition energies ($E_t$) and $\gamma$-branching ratios ($Br_\gamma$) have been listed. Pure $E0$ transitions are written in italics. The spins and parities are taken from this work and Ref. [4].

| $E_i$ (keV) | $J_i^\pi$ | $E_f$ (keV) | $J_f^\pi$ | $E_\gamma$ (keV) | $Br_\gamma$ |
|---|---|---|---|---|---|
| 405.5(1) | $2^+$ | 0.0 | $0^+$ | 405.5(1) | 100 |
| 523.7(2) | $0^+$ | 0.0 | $0^+$ | *523.7(2)* | *100* |
| 621.4(1) | $2^+$ | 0.0 | $0^+$ | 621.4(1) | 18.4(14) |
| | | 405.5(1) | $2^+$ | 216.0(1) | 100(5) |
| | | 523.7(2) | $0^+$ | 97.3(5) | 3.8(18)* |
| 808.4(1) | $4^+$ | 405.5(1) | $2^+$ | 402.8(1) | 100(5) |
| | | 621.4(1) | $2^+$ | 187.0(1) | 4.1(3) |
| 1080.8(1) | $4^+$ | 405.5(1) | $2^+$ | 675.2(1) | 100(5) |
| | | 621.4(1) | $2^+$ | 459.3(1) | 20.0(14) |
| | | 808.4(1) | $4^+$ | 272.5(1) | 2.4(3) |
| 1096.9(1) | $2^+$ | 0.0 | $0^+$ | 1096.9(1) | < 11[1] |
| | | 405.5(1) | $2^+$ | 691.4(1) | 100(5) |
| | | 523.7(2) | $0^+$ | 573.2(1) | 46(3) |
| 1165.4(1) | $6^+$ | 808.4(1) | $4^+$ | 357.0(1) | 100 |
| 1228.8(1) | $4^+$ | 621.4(1) | $2^+$ | 607.4(1) | 100 |
| 1248.0(1) | | 0.0 | $0^+$ | 1247.9(1) | 100(5) |
| | | 405.5(1) | $2^+$ | 842.5(1) | 33(3) |
| 1434.2(1) | $4^+$ | 405.5(1) | $2^+$ | 1028.7(2) | < 16.8[1] |
| | | 621.4(1) | $2^+$ | 812.6(1) | 47(5)* |
| | | 808.4(1) | $4^+$ | 625.9(1) | 100(5) |
| | | 1080.8(1) | $4^+$ | 353.4(2) | < 2.5 [2] |
| | | 1096.9(1) | $2^+$ | 337.2(1) | 15.0(17) |
| 1536.1(2) | | 523.7(2) | $0^+$ | 1012.4(1) | 100 |
| 1578.4(1) | $6^+$ | 808.4(1) | $4^+$ | 769.9(1) | 100(5) |
| | | 1080.8(1) | $4^+$ | 497.7(1) | 18.6(14) |
| | | 1165.4(1) | $6^+$ | 413.0(1) | 14.0(10) |
| | | 1228.8(1) | $4^+$ | 349.5(2) | 44(12)* |
| 1589.7(2) | $8^+$ | 1165.4(1) | $6^+$ | 424.4(1) | 100 |
| 1615.2(1) | | 405.5(1) | $2^+$ | 1209.7(1) | 100 |
| 1660.0(2) | | 808.4(1) | $4^+$ | 851.3(1) | 33(3) |
| | | 1080.8(1) | $4^+$ | 579.4(1) | 95(7) |
| | | 1096.9(1) | $2^+$ | 563.1(1) | 100(5) |
| 1678.2(1) | $6^+$ | 808.4(1) | $4^+$ | 869.7(1) | 25.2(18) |
| | | 1080.8(1) | $4^+$ | 597.4(1) | 100(5) |
| 1719.3(1) | | 405.5(1) | $2^+$ | 1313.8(1) | 100 |
| 1762.3(1) | | 1080.8(1) | $4^+$ | 681.2(3) | 41(14)* |

*Continued Table V*

| $E_i$ (keV) | $J_i^\pi$ | $E_f$ (keV) | $J_f^\pi$ | $E_\gamma$ (keV) | $Br_\gamma$ |
|---|---|---|---|---|---|
| | | 1096.9(1) | $2^+$ | 665.4(1) | 42(5) |
| | | 1228.8(1) | $4^+$ | 533.5(1) | 100(6) |
| 1845.1(4) | | 523.7(2) | $0^+$ | 1321.3(4) | 100 |
| 1868.9(1) | | 1080.8(1) | $4^+$ | 788.0(1) | 100(5) |
| | | 1165.4(1) | $6^+$ | 703.5(1) | $29(4)^*$ |
| | | 1434.2(1) | $4^+$ | 435.0(1) | 21.6(16) |
| 1905.7(1) | | 405.5(1) | $2^+$ | 1500.2(1) | 100 |
| 1907.0(1) | (5) | 808.4(1) | $4^+$ | 1098.6(2) | $47(6)^*$ |
| | | 1080.8(1) | $4^+$ | 826.4(1) | 100(5) |
| | | 1434.2(1) | $4^+$ | 472.7(1) | 16.0(14) |
| 1922.4(2) | | 405.5(1) | $2^+$ | 1516.9(1) | 100 |
| 1954.9(2) | | 1228.8(1) | $4^+$ | 726.0(1) | 100 |
| 1976.3(1) | $8^+$ | 1165.4(1) | $6^+$ | 811.0(1) | $96(8)^*$ |
| | | 1578.4(1) | $6^+$ | 397.9(1) | 100(5) |
| | | 1589.7(2) | $8^+$ | 386.7(1) | 13.1(11) |
| 1982.1(2) | | 405.5(1) | $2^+$ | 1576.6(1) | 100 |
| 1983.8(5) | | 1080.8(1) | $4^+$ | 903.1(5) | 100 |
| 1995.1(3) | | 1096.9(1) | $2^+$ | 898.2(3) | 100 |
| 1995.8(1) | | 621.4(1) | $2^+$ | 1374.3(1) | 100 |
| 2002.7(2) | | 1228.8(1) | $4^+$ | 773.7(1) | 95(7) |
| | | 1434.2(1) | $4^+$ | 568.8(1) | 100(5) |
| 2008.4(1) | | 1096.9(1) | $2^+$ | 911.5(2) | 100 |
| 2009.2(2) | | 621.4(1) | $2^+$ | 1387.7(2) | 100 |
| 2078.7(2) | $10^+$ | 1589.7(2) | $8^+$ | 488.9(1) | 100 |
| 2081.2(1) | | 808.4(1) | $4^+$ | 1272.8(1) | 100(5) |
| | | 1165.4(1) | $6^+$ | 915.7(2) | $37(7)^*$ |
| | | 1434.2(1) | $4^+$ | 647.1(1) | 27(2) |
| 2083.8(2) | | 1719.3(1) | | 364.5(1) | 100 |
| 2093.4(2) | | 808.4(1) | $4^+$ | 1285.0(2) | 100 |
| 2131.1(1) | | 1080.8(1) | $4^+$ | 1050.4(1) | 100(6) |
| | | 1434.2(1) | $4^+$ | 696.9(1) | 38(3) |
| 2138.2(2) | | 808.4(1) | $4^+$ | 1329.8(1) | 100 |
| 2138.8(1) | | 1080.8(1) | $4^+$ | 1058.0(1) | 100(6) |
| | | 1660.0(2) | | 478.8(5) | $35(12)^*$ |
| 2140.4(2) | | 405.5(1) | $2^+$ | 1735.0(1) | 100(6) |
| | | 523.7(2) | $0^+$ | 1616.3(1) | 50(5) |
| 2155.6(3) | | 621.4(1) | $2^+$ | 1534.1(3) | 100 |
| 2155.9(1) | $(8^+)$ | 1165.4(1) | $6^+$ | 990.4(1) | 16(3) |
| | | 1589.7(2) | $8^+$ | 566.2(1) | 39(8) |
| | | 1678.2(1) | $6^+$ | 477.8(1) | $100(19)^*$ |
| 2170.5(2) | | 405.5(1) | $2^+$ | 1765.0(1) | 100 |
| 2185.7(3) | | 1907.0(1) | (5) | 278.7(3) | 100 |
| 2186.6(2) | $(6^-)$ | 1578.4(1) | $6^+$ | 608.2(2) | 100 |
| 2199.7(3) | | 1719.3(1) | | 480.4(2) | 100 |
| 2211.6(1) | | 1080.8(1) | $4^+$ | 1130.8(1) | 100(6) |
| | | 1434.2(1) | $4^+$ | 777.5(1) | 41(4) |
| 2214.1(2) | | 808.4(1) | $4^+$ | 1405.7(2) | 100 |
| 2214.7(2) | | 621.4(1) | $2^+$ | 1593.3(1) | 100 |
| 2218.4(1) | $(8^-)$ | 1589.7(2) | $8^+$ | 628.4(1) | 37(3) |
| | | 1976.3(1) | $8^+$ | 242.1(1) | 100(5) |
| 2231.5(2) | | 523.7(2) | $0^+$ | 1707.8(1) | 100 |
| 2234.5(4) | | 621.4(1) | $2^+$ | 1613.1(4) | 100 |
| 2254.3(2) | | 1080.8(1) | $4^+$ | 1173.7(2) | 74(9) |
| | | 1165.4(1) | $6^+$ | 1088.8(1) | 100(9) |
| 2264.5(2) | | 523.7(2) | $0^+$ | 1740.8(2) | 100 |
| 2267.7(1) | (7) | 1165.4(1) | $6^+$ | 1102.4(1) | 32(3) |
| | | 1589.7(2) | $8^+$ | 678.5(4) | $9(3)^*$ |
| | | 1868.9(1) | | 398.8(1) | $99(41)^*$ |
| | | 1907.0(1) | (5) | 360.6(1) | 100(6) |
| 2280.1(1) | | 808.4(1) | $4^+$ | 1471.7(1) | 100 |

*Continued Table V*

| $E_i$ (keV) | $J_i^\pi$ | $E_f$ (keV) | $J_f^\pi$ | $E_\gamma$ (keV) | $Br_\gamma$ |
|---|---|---|---|---|---|
| 2324.4(2) | | 1165.4(1) | $6^+$ | 1159.1(1) | 100 |
| 2342.0(2) | | 621.4(1) | $2^+$ | 1720.6(1) | 100 |
| 2342.5(2) | | 1165.4(1) | $6^+$ | 1177.2(2) | 100 |
| 2350.3(2) | $(6^+,7)$ | 1165.4(1) | $6^+$ | 1185.0(1) | 29(13) |
| | | 1589.7(2) | $8^+$ | 760.2(1) | 51(22) |
| | | 1868.9(1) | | 481.4(2) | $100(42)^*$ |
| | | 1907.0(1) | (5) | 443.2(2) | $55(25)^*$ |
| 2356.0(3) | | 1907.0(1) | (5) | 449.0(3) | 100 |
| 2380.7(1) | | 808.4(1) | $4^+$ | 1572.4(1) | 100(7) |
| | | 1165.4(1) | $6^+$ | 1215.1(2) | $83(40)^*$ |
| 2384.9(2) | | 405.5(1) | $2^+$ | 1979.4(1) | 100 |
| 2388.4(2) | | 1165.4(1) | $6^+$ | 1223.0(1) | 100 |
| 2393.0(2) | | 808.4(1) | $4^+$ | 1584.6(2) | 100 |
| 2403.2(2) | | 1589.7(2) | $8^+$ | 813.3(2) | $31(9)^*$ |
| | | 1678.2(1) | $6^+$ | 725.1(2) | $100(21)^*$ |
| 2405.3(2) | | 1868.9(1) | | 536.4(1) | 100 |
| 2422.0(5) | | 621.4(1) | $2^+$ | 1800.6(5) | 100 |
| 2428.2(1) | $10^+$ | 1589.7(2) | $8^+$ | 838.4(1) | 89(27) |
| | | 1976.3(1) | $8^+$ | 451.9(2) | $100(29)^*$ |
| 2428.4(1) | | 1678.2(1) | $6^+$ | 750.2(1) | 77(8) |
| | | 1868.9(1) | | 559.7(1) | 100(5) |
| 2467.1(3) | $(8^-)$ | 2186.6(2) | $(6^-)$ | 280.5(2) | 100 |
| 2469.2(3) | | 1589.7(2) | $8^+$ | 879.3(4) | $40(19)^*$ |
| | | 1678.2(1) | $6^+$ | 791.4(5) | $100(34)^*$ |
| 2474.0(2) | | 1165.4(1) | $6^+$ | 1308.6(1) | 100 |
| 2475.9(2) | | 1589.7(2) | $8^+$ | 886.1(1) | 100 |
| 2489.5(3) | | 621.4(1) | $2^+$ | 1868.2(4) | $31(15)^*$ |
| | | 1080.8(1) | $4^+$ | 1408.3(5) | 100(24) |
| 2509.1(6) | | 621.4(1) | $2^+$ | 1887.7(6) | 100 |
| 2516.1(2) | | 1165.4(1) | $6^+$ | 1350.7(1) | 100(6) |
| | | 1589.7(2) | $8^+$ | 926.3(5) | $35(15)^*$ |
| 2564.5(2) | | 1165.4(1) | $6^+$ | 1399.2(3) | $100(23)^*$ |
| | | 1589.7(2) | $8^+$ | 974.8(3) | $92(30)^*$ |
| 2574.0(2) | (9) | 2267.7(1) | (7) | 306.3(1) | 100 |
| 2577.1(2) | | 1589.7(2) | $8^+$ | 987.2(1) | 77(7) |
| | | 1976.3(1) | $8^+$ | 600.9(1) | 100(6) |
| 2590.6(1) | | 1165.4(1) | $6^+$ | 1425.3(1) | 89(11) |
| | | 1589.7(2) | $8^+$ | 1000.8(1) | 100(10) |
| 2608.9(2) | | 1165.4(1) | $6^+$ | 1443.7(3) | $58(13)^*$ |
| | | 1589.7(2) | $8^+$ | 1019.1(1) | 100(7) |
| 2620.7(2) | $12^+$ | 2078.7(2) | $10^+$ | 542.1(1) | 100 |
| 2628.6(2) | | 1589.7(2) | $8^+$ | 1038.9(1) | 100 |
| 2633.6(1) | | 1976.3(1) | $8^+$ | 657.3(1) | 100 |
| 2637.3(2) | $(10^+)$ | 2078.7(2) | $10^+$ | 558.4(4) | $83(35)^*$ |
| | | 2155.9(1) | $(8^+)$ | 481.5(2) | $100(26)^*$ |
| 2649.7(2) | | 1589.7(2) | $8^+$ | 1060.0(1) | 100 |
| 2685.0(2) | | 1165.4(1) | $6^+$ | 1519.7(1) | 100 |
| 2693.8(2) | | 1165.4(1) | $6^+$ | 1528.4(1) | 100 |
| 2706.7(2) | | 1589.7(2) | $8^+$ | 1116.9(1) | 100 |
| 2715.7(3) | | 2078.7(2) | $10^+$ | 637.0(3) | 100 |
| 2758.2(3) | | 1678.2(1) | $6^+$ | 1080.0(3) | 100 |
| 2772.6(2) | | 808.4(1) | $4^+$ | 1964.2(1) | 100 |
| 2791.2(5) | | 1165.4(1) | $6^+$ | 1625.9(5) | 100 |
| 2833.7(2) | $10^+$ | 1589.7(2) | $8^+$ | 1243.8(5) | $95(33)^*$ |
| | | 2078.7(2) | $10^+$ | 755.0(2) | 100(16) |
| 2890.0(2) | | 1589.7(2) | $8^+$ | 1300.3(1) | 100 |
| 2908.7(2) | | 1589.7(2) | $8^+$ | 1318.9(1) | 77(9) |
| | | 2078.7(2) | $10^+$ | 829.9(1) | 100(6) |
| 2912.1(3) | | 523.7(2) | $0^+$ | 2388.4(3) | 100 |
| 3003.2(2) | | 1165.4(1) | $6^+$ | 1837.8(2) | 100 |

*Continued Table V*

| $E_i$ (keV) | $J_i^\pi$ | $E_f$ (keV) | $J_f^\pi$ | $E_\gamma$ (keV) | $Br_\gamma$ |
|---|---|---|---|---|---|
| 3011.9(3) | | 2078.7(2) | $10^+$ | 933.2(3) | 100 |
| 3024.9(3) | | 1165.4(1) | $6^+$ | 1859.6(3) | 100 |

[1] $\gamma$ ray not observed, upper limit, given within 95% credible interval, obtained from the $\gamma$-$\gamma$ coincidence data.
[2] Observed only as conversion electrons, $\gamma$-branching ratio limits given with 95% credible interval.

TABLE VI: The relative $\gamma$-ray intensities in $^{186}$Hg, normalized to the strongest $2_1^+ \rightarrow 0_1^+$ 406 keV transition. The intensities of transitions marked with * were determined from coincidences.

| $E_\gamma$ (keV) | $I_\gamma$ | $E_i$ (keV) | $E_f$ (keV) |
|---|---|---|---|
| 97.3(5) | 0.141(66)* | 621.4(1) | 523.7(2) |
| 187.0(1) | 2.11(15) | 808.4(1) | 621.4(1) |
| 216.0(1) | 3.7(3) | 621.4(1) | 405.5(1) |
| 242.1(1) | 1.71(13) | 2218.4(1) | 1976.3(1) |
| 272.5(1) | 0.36(4) | 1080.8(1) | 808.4(1) |
| 278.7(3) | 0.55(16)* | 2185.7(3) | 1907.0(1) |
| 280.5(2) | 0.38(8)* | 2467.1(3) | 2186.6(2) |
| 306.3(1) | 0.78(6) | 2574.0(2) | 2267.7(1) |
| 337.2(1) | 0.46(5) | 1434.2(1) | 1096.9(1) |
| 349.5(2) | 2.2(6)* | 1578.4(1) | 1228.8(1) |
| 353.4(2) | $< 0.076$[1] | 1434.2(1) | 1080.8(1) |
| 357.0(1) | 31(2) | 1165.4(1) | 808.4(1) |
| 360.6(1) | 1.56(12) | 2267.7(1) | 1907.0(1) |
| 364.5(1) | 0.35(3) | 2083.8(2) | 1719.3(1) |
| 386.7(1) | 0.41(3) | 1976.3(1) | 1589.7(2) |
| 397.9(1) | 3.1(2) | 1976.3(1) | 1578.4(1) |
| 398.8(1) | 1.5(6)* | 2267.7(1) | 1868.9(1) |
| 402.8(1) | 51(4) | 808.4(1) | 405.5(1) |
| 405.5(1) | 100 | 405.5(1) | 0.0 |
| 413.0(1) | 0.70(5) | 1578.4(1) | 1165.4(1) |
| 424.4(1) | 14.1(10) | 1589.7(2) | 1165.4(1) |
| 435.0(1) | 0.60(5) | 1868.9(1) | 1434.2(1) |
| 443.2(2) | 0.56(12)* | 2350.3(2) | 1907.0(1) |
| 449.0(3) | 0.38(11)* | 2356.0(3) | 1907.0(1) |
| 451.9(2) | 0.8(2)* | 2428.2(1) | 1976.3(1) |
| 459.3(1) | 3.0(2) | 1080.8(1) | 621.4(1) |
| 472.7(1) | 0.45(4) | 1907.0(1) | 1434.2(1) |
| 477.8(1) | 2.1(4)* | 2155.9(1) | 1678.2(1) |
| 478.8(5) | 0.27(9)* | 2138.8(1) | 1660.0(2) |
| 480.4(2) | 0.25(8)* | 2199.7(3) | 1719.3(1) |
| 481.4(2) | 1.0(4)* | 2350.3(2) | 1868.9(1) |
| 481.5(2) | 0.17(5)* | 2637.3(2) | 2155.9(1) |
| 488.9(1) | 2.8(2) | 2078.7(2) | 1589.7(2) |
| 497.7(1) | 0.93(7) | 1578.4(1) | 1080.8(1) |
| 523.7(2) | 3.6(3)[2] | 523.7(2) | 0.0 |
| 533.5(1) | 0.52(4) | 1762.3(1) | 1228.8(1) |
| 536.4(1) | 0.17(2) | 2405.3(2) | 1868.9(1) |
| 542.1(1) | 0.32(3) | 2620.7(2) | 2078.7(2) |
| 558.4(4) | 0.15(5))* | 2637.3(2) | 2078.7(2 |
| 559.7(1) | 0.61(5) | 2428.4(1) | 1868.9(1) |
| 563.1(1) | 0.66(5) | 1660.0(2) | 1096.9(1) |
| 566.2(1) | 0.80(6) | 2155.9(1) | 1589.7(2) |
| 568.8(1) | 0.56(4) | 2002.7(2) | 1434.2(1) |
| 573.2(1) | 1.55(11) | 1096.9(1) | 523.7(2) |
| 579.4(1) | 0.63(5) | 1660.0(2) | 1080.8(1) |
| 597.4(1) | 4.4(3) | 1678.2(1) | 1080.8(1) |
| 600.9(1) | 0.49(4) | 2577.1(2) | 1976.3(1) |
| 607.4(1) | 7.3(6)* | 1228.8(1) | 621.4(1) |
| 608.2(2) | 1.38(19)* | 2186.6(2) | 1578.4(1) |
| 621.4(1) | 0.67(5) | 621.4(1) | 0.0 |
| 625.9(1) | 3.1(2) | 1434.2(1) | 808.4(1) |
| 628.4(1) | 0.64(5) | 2218.4(1) | 1589.7(2) |
| 637.0(3) | 0.18(6)* | 2715.7(3) | 2078.7(2) |
| 647.1(1) | 0.43(4) | 2081.2(1) | 1434.2(1) |
| 657.3(1) | 0.38(4) | 2633.6(1) | 1976.3(1) |
| 665.4(1) | 0.22(3) | 1762.3(1) | 1096.9(1) |
| 675.2(1) | 14.8(11) | 1080.8(1) | 405.5(1) |
| 678.5(4) | 0.14(5)* | 2267.7(1) | 1589.7(2) |
| 681.2(3) | 0.21(7)* | 1762.3(1) | 1080.8(1) |
| 691.4(1) | 3.4(2) | 1096.9(1) | 405.5(1) |
| 696.9(1) | 0.209(18) | 2131.1(1) | 1434.2(1) |
| 703.5(1) | 0.82(10)* | 1868.9(1) | 1165.4(1) |
| 725.1(2) | 0.96(20)* | 2403.2(2) | 1678.2(1) |
| 726.0(1) | 0.86(14)* | 1954.9(2) | 1228.8(1) |
| 750.2(1) | 0.47(5) | 2428.4(1) | 1678.2(1) |
| 755.0(2) | 0.21(4) | 2833.7(2) | 2078.7(2) |
| 760.2(1) | 0.52(4) | 2350.3(2) | 1589.7(2) |
| 769.9(1) | 5.0(4) | 1578.4(1) | 808.4(1) |
| 773.7(1) | 0.53(4) | 2002.7(2) | 1228.8(1) |
| 777.5(1) | 0.29(2) | 2211.6(1) | 1434.2(1) |
| 788.0(1) | 2.8(2) | 1868.9(1) | 1080.8(1) |
| 791.4(5) | 0.25(9)* | 2469.2(3) | 1678.2(1) |
| 811.0(1) | 3.0(2)* | 1976.3(1) | 1165.4(1) |
| 812.6(1) | 1.43(15)* | 1434.2(1) | 621.4(1) |
| 813.3(2) | 0.29(6)* | 2403.2(2) | 1589.7(2) |
| 826.4(1) | 2.8(2) | 1907.0(1) | 1080.8(1) |
| 829.9(1) | 0.26(2) | 2908.7(2) | 2078.7(2) |
| 838.4(1) | 0.72(5) | 2428.2(1) | 1589.7(2) |
| 842.5(1) | 0.55(4) | 1248.0(1) | 405.5(1) |
| 851.3(1) | 0.219(18) | 1660.0(2) | 808.4(1) |
| 869.7(1) | 1.10(8) | 1678.2(1) | 808.4(1) |
| 879.3(4) | 0.10(4)* | 2469.2(3) | 1589.7(2) |
| 886.1(1) | 0.66(5) | 2475.9(2) | 1589.7(2) |
| 898.2(3) | 0.28(8)* | 1995.1(3) | 1096.9(1) |
| 903.1(5) | 0.20(7)* | 1983.8(5) | 1080.8(1) |
| 911.5(2) | 0.48(10)* | 2008.4(1) | 1096.9(1) |
| 915.7(2) | 0.58(11)* | 2081.2(1) | 1165.4(1) |
| 926.3(5) | 0.19(8)* | 2516.1(2) | 1589.7(2) |
| 933.2(3) | 0.10(4)* | 3011.9(3) | 2078.7(2) |
| 974.8(3) | 0.22(5)* | 2564.5(2) | 1589.7(2) |
| 987.2(1) | 0.38(3) | 2577.1(2) | 1589.7(2) |
| 990.4(1) | 0.34(3) | 2155.9(1) | 1165.4(1) |
| 1000.8(1) | 0.26(3) | 2590.6(1) | 1589.7(2) |
| 1012.4(1) | 0.176(17) | 1536.1(2) | 523.7(2) |
| 1019.1(1) | 0.41(4) | 2608.9(2) | 1589.7(2) |
| 1028.7(2) | $< 0.52$[1] | 1434.2(1) | 405.5(1) |
| 1038.9(1) | 0.37(5) | 2628.6(2) | 1589.7(2) |
| 1050.4(1) | 0.55(4) | 2131.1(1) | 1080.8(1) |
| 1058.0(1) | 0.77(6) | 2138.8(1) | 1080.8(1) |
| 1060.0(1) | 0.45(4) | 2649.7(2) | 1589.7(2) |
| 1080.0(3) | 0.27(9)* | 2758.2(3) | 1678.2(1) |
| 1088.8(1) | 0.24(2) | 2254.3(2) | 1165.4(1) |
| 1096.9(1) | $< 0.37$[1] | 1096.9(1) | 0.0 |
| 1098.6(2) | 1.30(17)* | 1907.0(1) | 808.4(1) |
| 1102.4(1) | 0.50(4) | 2267.7(1) | 1165.4(1) |
| 1116.9(1) | 0.41(3) | 2706.7(2) | 1589.7(2) |
| 1130.8(1) | 0.70(5) | 2211.6(1) | 1080.8(1) |
| 1159.1(1) | 0.148(18) | 2324.4(2) | 1165.4(1) |
| 1173.7(2) | 0.175(17) | 2254.3(2) | 1080.8(1) |
| 1177.2(2) | 0.49(8)* | 2342.5(2) | 1165.4(1) |
| 1185.0(1) | 0.30(3) | 2350.3(2) | 1165.4(1) |
| 1209.7(1) | 1.31(9) | 1615.2(1) | 405.5(1) |

| $E_\gamma$ (keV) | $I_\gamma$ | $E_i$ (keV) | $E_f$ (keV) |
|---|---|---|---|
| 1215.1(2) | 0.16(8)* | 2380.7(1) | 1165.4(1) |
| 1223.0(1) | 0.40(3) | 2388.4(2) | 1165.4(1) |
| 1243.8(5) | 0.20(6)* | 2833.7(2) | 1589.7(2) |
| 1247.9(1) | 1.65(12) | 1248.0(1) | 0.0 |
| 1272.8(1) | 1.59(11) | 2081.2(1) | 808.4(1) |
| 1285.0(2) | 0.086(13) | 2093.4(2) | 808.4(1) |
| 1300.3(1) | 0.24(2) | 2890.0(2) | 1589.7(2) |
| 1308.6(1) | 0.57(4) | 2474.0(2) | 1165.4(1) |
| 1313.8(1) | 1.13(8) | 1719.3(1) | 405.5(1) |
| 1318.9(1) | 0.20(2) | 2908.7(2) | 1589.7(2) |
| 1321.3(4) | 0.050(18)* | 1845.1(4) | 523.7(2) |
| 1329.8(1) | 0.21(2) | 2138.2(2) | 808.4(1) |
| 1350.7(1) | 0.55(4) | 2516.1(2) | 1165.4(1) |
| 1374.3(1) | 0.74(6) | 1995.8(1) | 621.4(1) |
| 1387.7(2) | 0.20(2) | 2009.2(2) | 621.4(1) |
| 1399.2(3) | 0.24(6)* | 2564.5(2) | 1165.4(1) |
| 1405.7(2) | 0.35(6) | 2214.1(2) | 808.4(1) |
| 1408.3(5) | 0.28(7) | 2489.5(3) | 1080.8(1) |
| 1425.3(1) | 0.23(2) | 2590.6(1) | 1165.4(1) |
| 1443.7(3) | 0.24(5)* | 2608.9(2) | 1165.4(1) |
| 1471.7(1) | 0.94(7) | 2280.1(1) | 808.4(1) |
| 1500.2(1) | 0.49(4) | 1905.7(1) | 405.5(1) |
| 1516.9(1) | 0.41(4) | 1922.4(2) | 405.5(1) |
| 1519.7(1) | 0.30(3) | 2685.0(2) | 1165.4(1) |
| 1528.4(1) | 0.184(18) | 2693.8(2) | 1165.4(1) |
| 1534.1(3) | 0.12(3)* | 2155.6(3) | 621.4(1) |
| 1572.4(1) | 0.189(17) | 2380.7(1) | 808.4(1) |
| 1576.6(1) | 0.27(2) | 1982.1(2) | 405.5(1) |
| 1584.6(2) | 0.092(14) | 2393.0(2) | 808.4(1) |
| 1593.3(1) | 0.22(2) | 2214.7(2) | 621.4(1) |
| 1613.1(4) | 0.18(7)* | 2234.5(4) | 621.4(1) |
| 1616.3(1) | 0.129(13) | 2140.4(2) | 523.7(2) |
| 1625.9(5) | 0.21(7)* | 2791.2(5) | 1165.4(1) |
| 1707.8(1) | 0.22(2) | 2231.5(2) | 523.7(2) |
| 1720.6(1) | 0.133(16) | 2342.0(2) | 621.4(1) |
| 1735.0(1) | 0.26(2) | 2140.4(2) | 405.5(1) |
| 1740.8(2) | 0.161(19) | 2264.5(2) | 523.7(2) |
| 1765.0(1) | 0.41(4) | 2170.5(2) | 405.5(1) |
| 1800.6(5) | 0.27(7)* | 2422.0(5) | 621.4(1) |
| 1837.8(2) | 0.19(3) | 3003.2(2) | 1165.4(1) |
| 1859.6(3) | 0.11(3)* | 3024.9(3) | 1165.4(1) |
| 1868.2(4) | 0.09(4)* | 2489.5(3) | 621.4(1) |
| 1887.7(6) | 0.18(7)* | 2509.1(6) | 621.4(1) |
| 1964.2(1) | 0.22(2) | 2772.6(2) | 808.4(1) |
| 1979.4(1) | 0.22(2) | 2384.9(2) | 405.5(1) |
| 2388.4(3) | 0.09(2) | 2912.1(3) | 523.7(2) |

[1] Limit given in 95% credible interval.
[2] $E0$ transition. The intensity of K electrons was multiplied by a factor 1.2 to account for other shells.


[1] B. Singh, Nuclear Data Sheets **130**, 21 (2015), URL https://www.sciencedirect.com/science/article/pii/S0090375215000563.

[2] C. M. Baglin, Nuclear Data Sheets **111**, 275 (2010), URL https://www.sciencedirect.com/science/article/pii/S0090375210000189.

[3] E. Rapisarda, A. N. Andreyev, S. Antalic, A. Barzakh, T. E. Cocolios, I. G. Darby, R. De Groote, H. De Witte, J. Diriken, J. Elseviers, et al., Journal of Physics G: Nuclear and Particle Physics **44**, 074001 (2017), URL https://iopscience.iop.org/article/10.1088/1361-6471/aa6bb6.

[4] J. Batchelder, A. Hurst, and M. Basunia, Nuclear Data Sheets **183**, 1 (2022), URL https://www.sciencedirect.com/science/article/pii/S009037522200031X.

[5] T. Grahn, A. Petts, M. Scheck, P. A. Butler, A. Dewald, M. B. Gómez Hornillos, P. T. Greenlees, A. Görgen, K. Helariutta, J. Jolie, et al., Physical Review C **80**, 014324 (2009), URL https://link.aps.org/doi/10.1103/PhysRevC.80.014324.

[6] L. P. Gaffney, M. Hackstein, R. D. Page, T. Grahn, M. Scheck, P. A. Butler, P. F. Bertone, N. Bree, R. J. Carroll, M. P. Carpenter, et al., Physical Review C **89**, 024307 (2014), 1401.5030, URL https://link.aps.org/doi/10.1103/PhysRevC.89.024307.

[7] K. Wrzosek-Lipska, K. Rezynkina, N. Bree, M. Zielińska, L. P. Gaffney, A. Petts, A. Andreyev, B. Bastin, M. Bender, A. Blazhev, et al., The European Physical Journal A **55**, 130 (2019), URL http://link.springer.com/10.1140/epja/i2019-12815-2.

TABLE VII. Comparison of the experimental $B(E2)$ transition strengths taken from Ref. [5–7] with the SCCM theoretical model. Values are given in units of $e^2b^2$.

| Nucleus | Value | Experiment | SCCM |
|---|---|---|---|
| $^{182}$Hg | $B(E2; 2_1^+ \to 0_1^+)$ | 0.33(2) | 0.071 |
| | $B(E2; 2_2^+ \to 0_1^+)$ | 0.072(24) | 0.36 |
| | $B(E2; 4_1^+ \to 2_1^+)$ | 1.52(5) | 2.80 |
| | $B(E2; 6_1^+ \to 4_1^+)$ | 2.27(18) | 3.15 |
| | $B(E2; 8_1^+ \to 6_1^+)$ | 2.33(25) | 3.38 |
| $^{184}$Hg | $B(E2; 2_1^+ \to 0_1^+)$ | 0.320(15) | 0.40 |
| | $B(E2; 2_2^+ \to 0_1^+)$ | 0.024(4) | 0.00072 |
| | $B(E2; 4_1^+ \to 2_1^+)$ | 1.22(4) | 0.074 |
| | $B(E2; 6_1^+ \to 4_1^+)$ | 1.91(9) | 2.74 |
| | $B(E2; 8_1^+ \to 6_1^+)$ | 1.92(8) | 2.94 |
| $^{186}$Hg | $B(E2; 2_1^+ \to 0_1^+)$ | $0.31^{+0.05}_{-0.04}$ | 0.40 |
| | $B(E2; 2_2^+ \to 0_1^+)$ | 0.0005(2) | 0.0012 |
| | $B(E2; 4_1^+ \to 2_1^+)$ | 1.28(15) | 0.011 |
| | $B(E2; 6_1^+ \to 4_1^+)$ | 1.46(6) | 2.34 |
| | $B(E2; 8_1^+ \to 6_1^+)$ | 1.27(9) | 2.50 |
