# Supplementary material for: Simultaneous $\gamma$-ray and electron spectroscopy of $^{182,184,186}$Hg isotopes
Source: arXiv:2305.16442 ancillary file (2023-06-06)

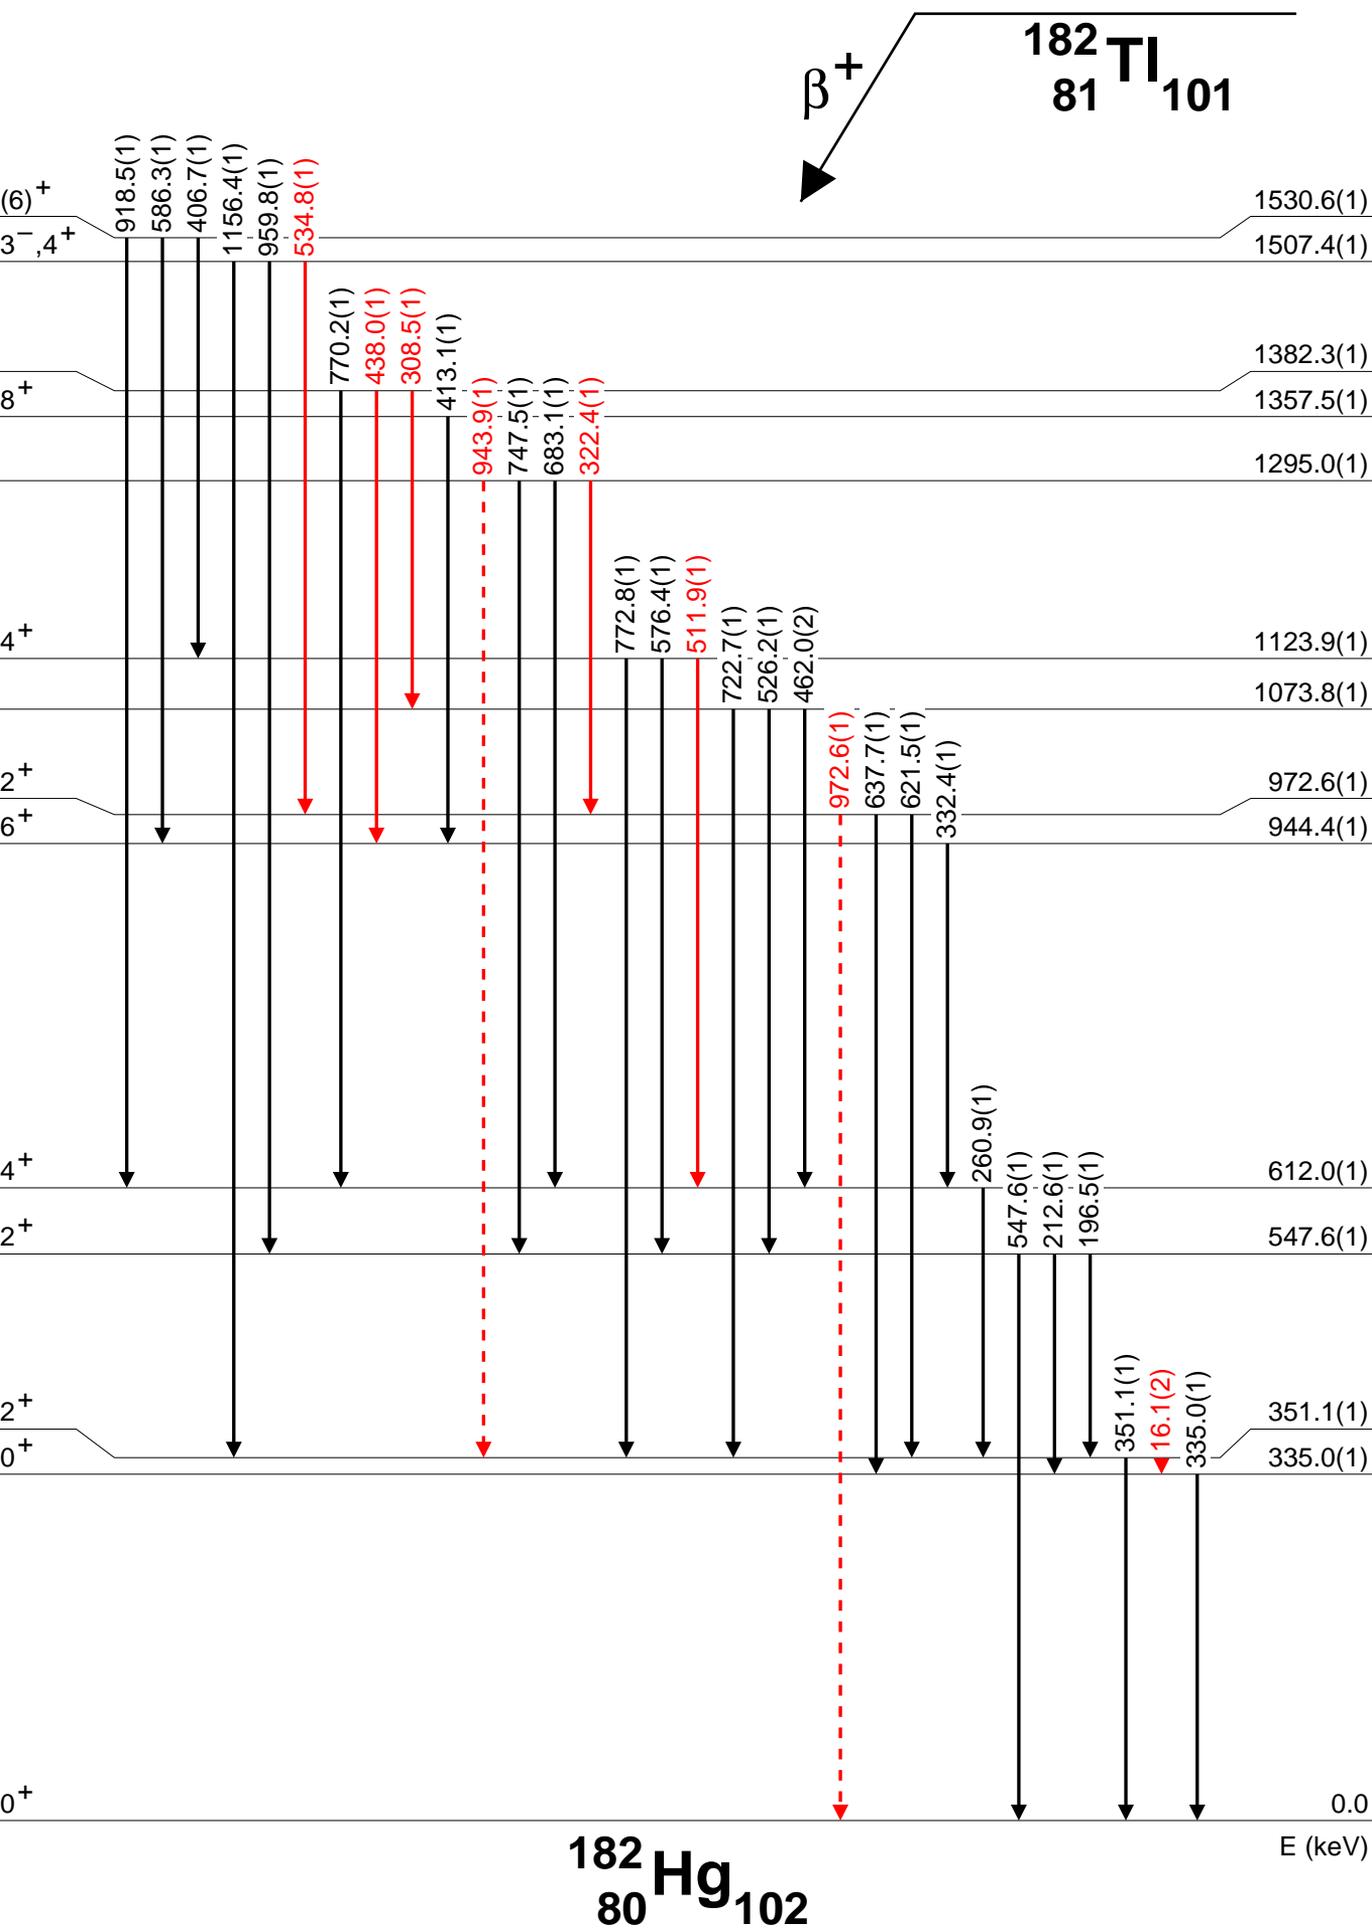

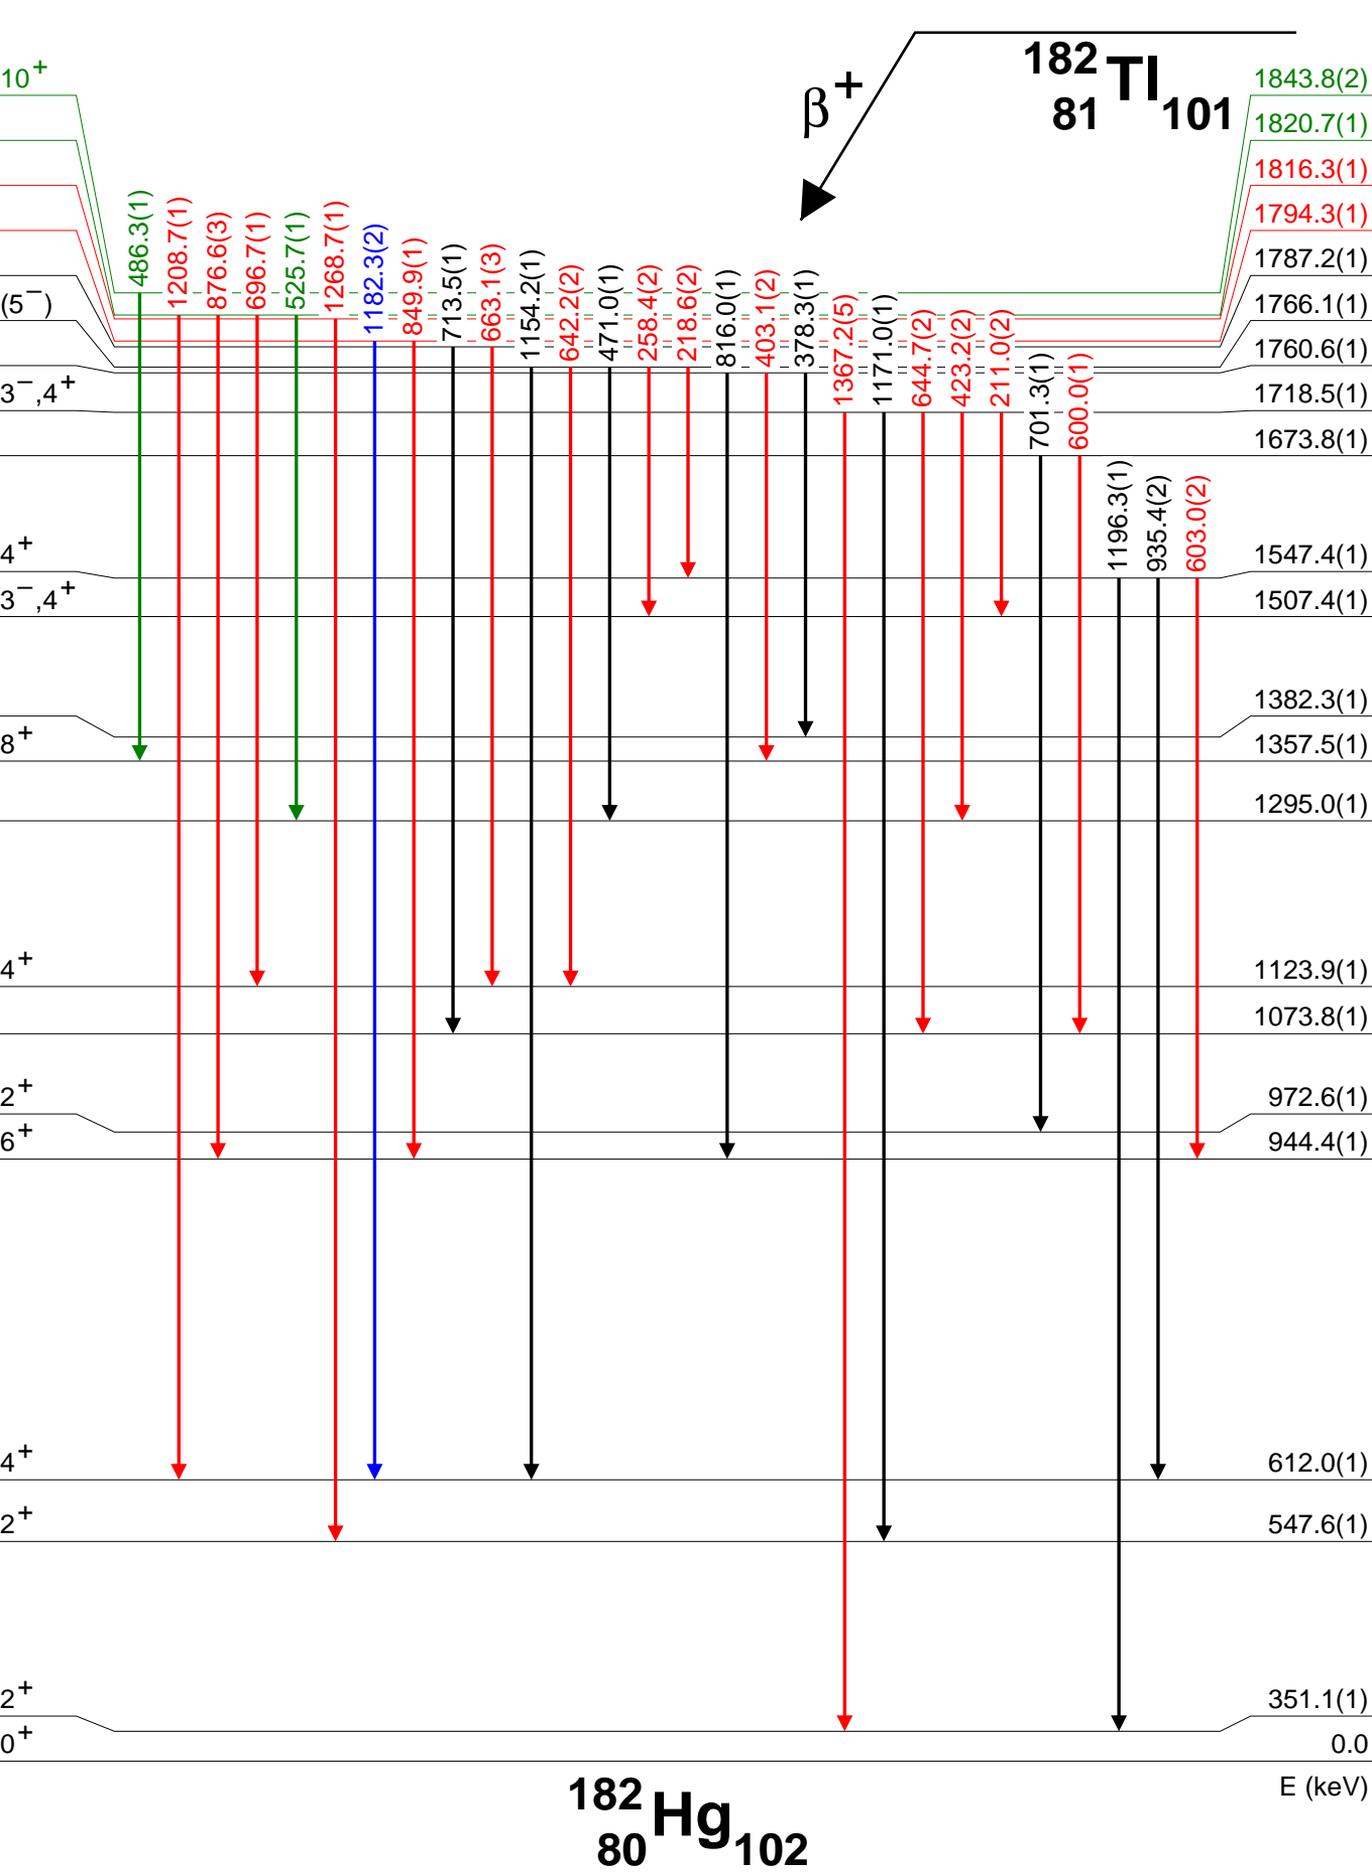

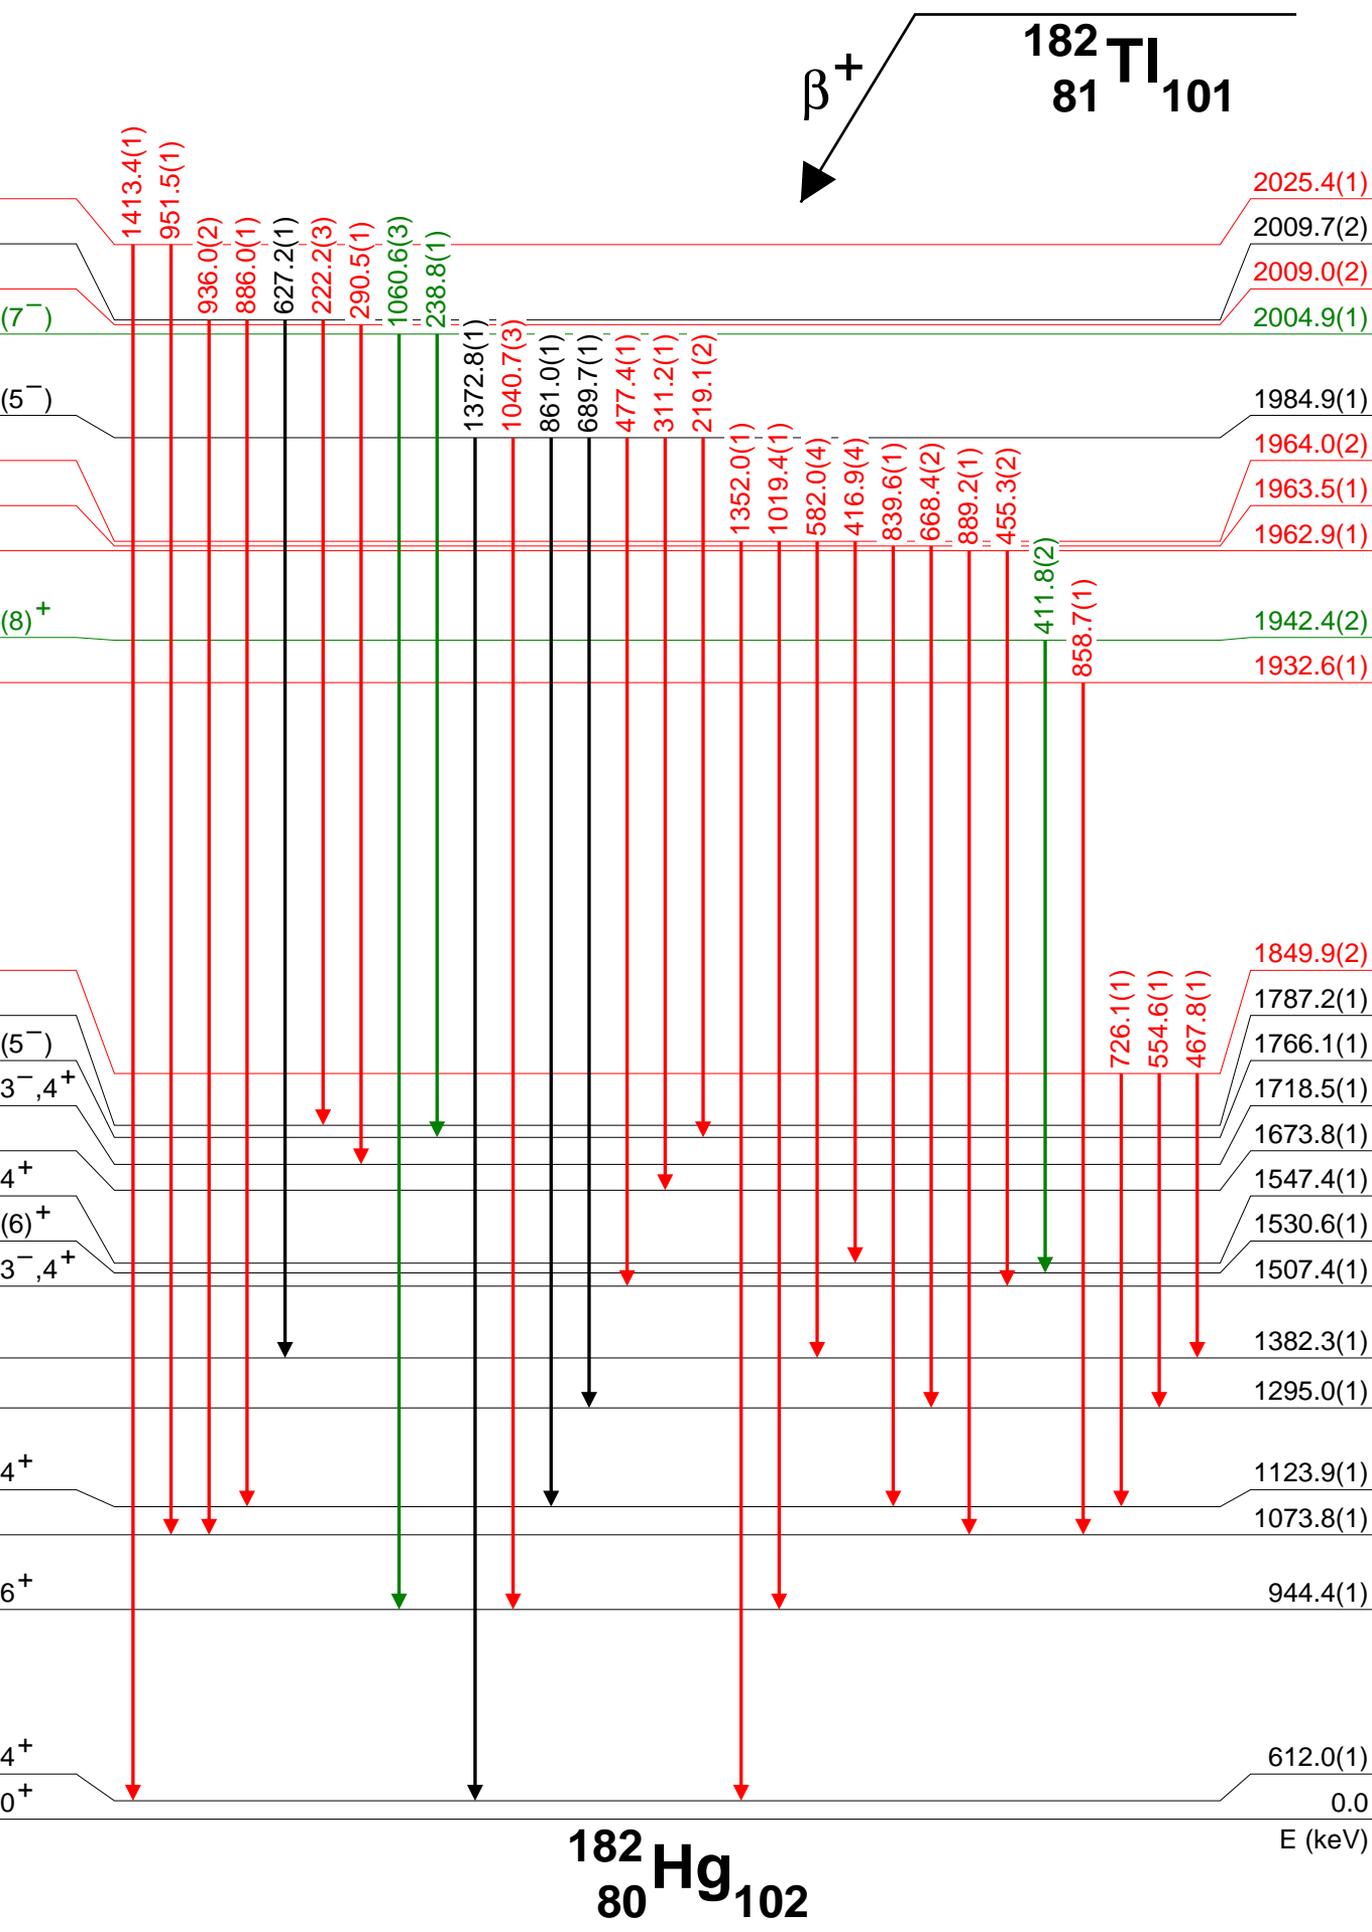

$\beta^+$   $^{182}\text{Tl}_{101}$

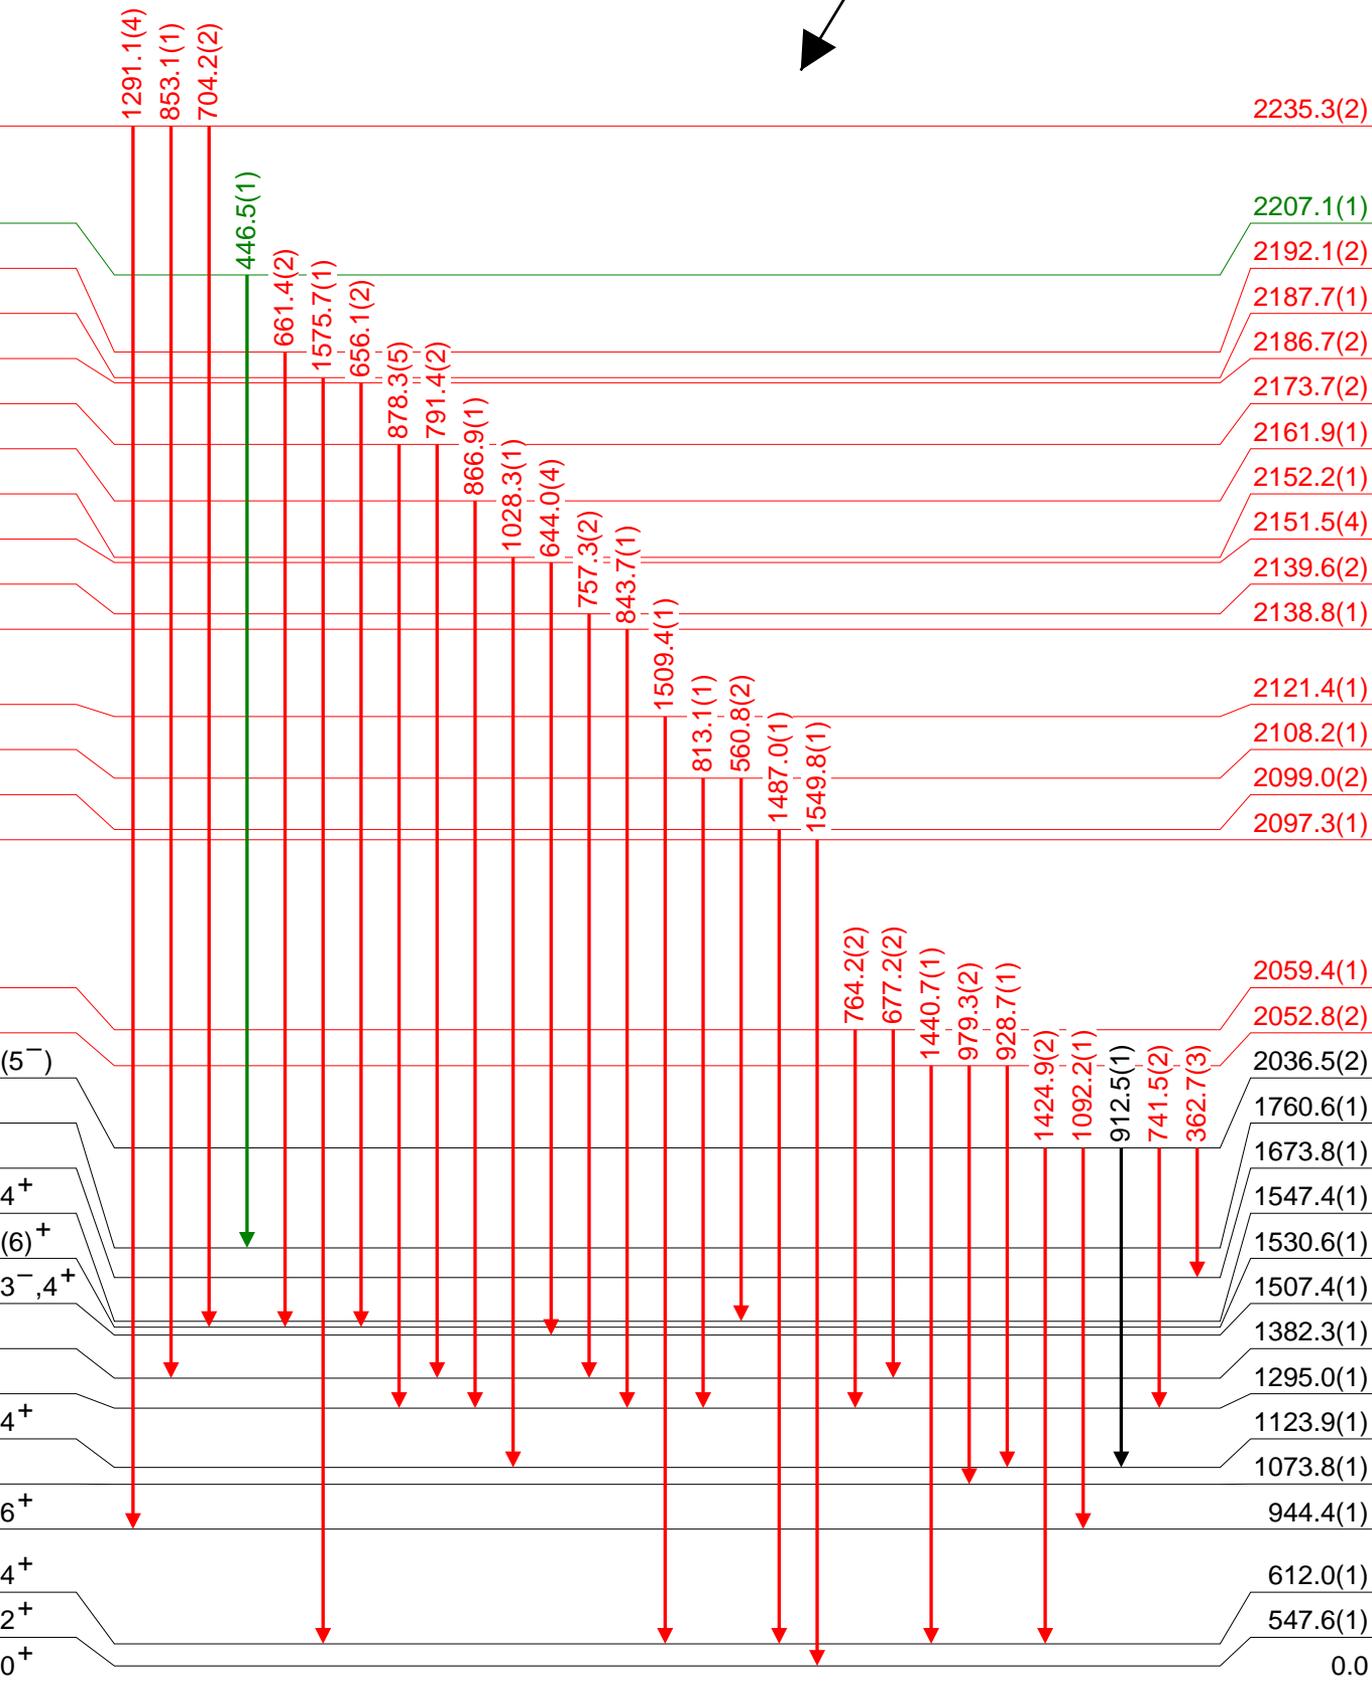

$^{182}\text{Hg}_{102}$

E (keV)

$\beta^+$   $^{182}_{81}\text{Tl}_{101}$

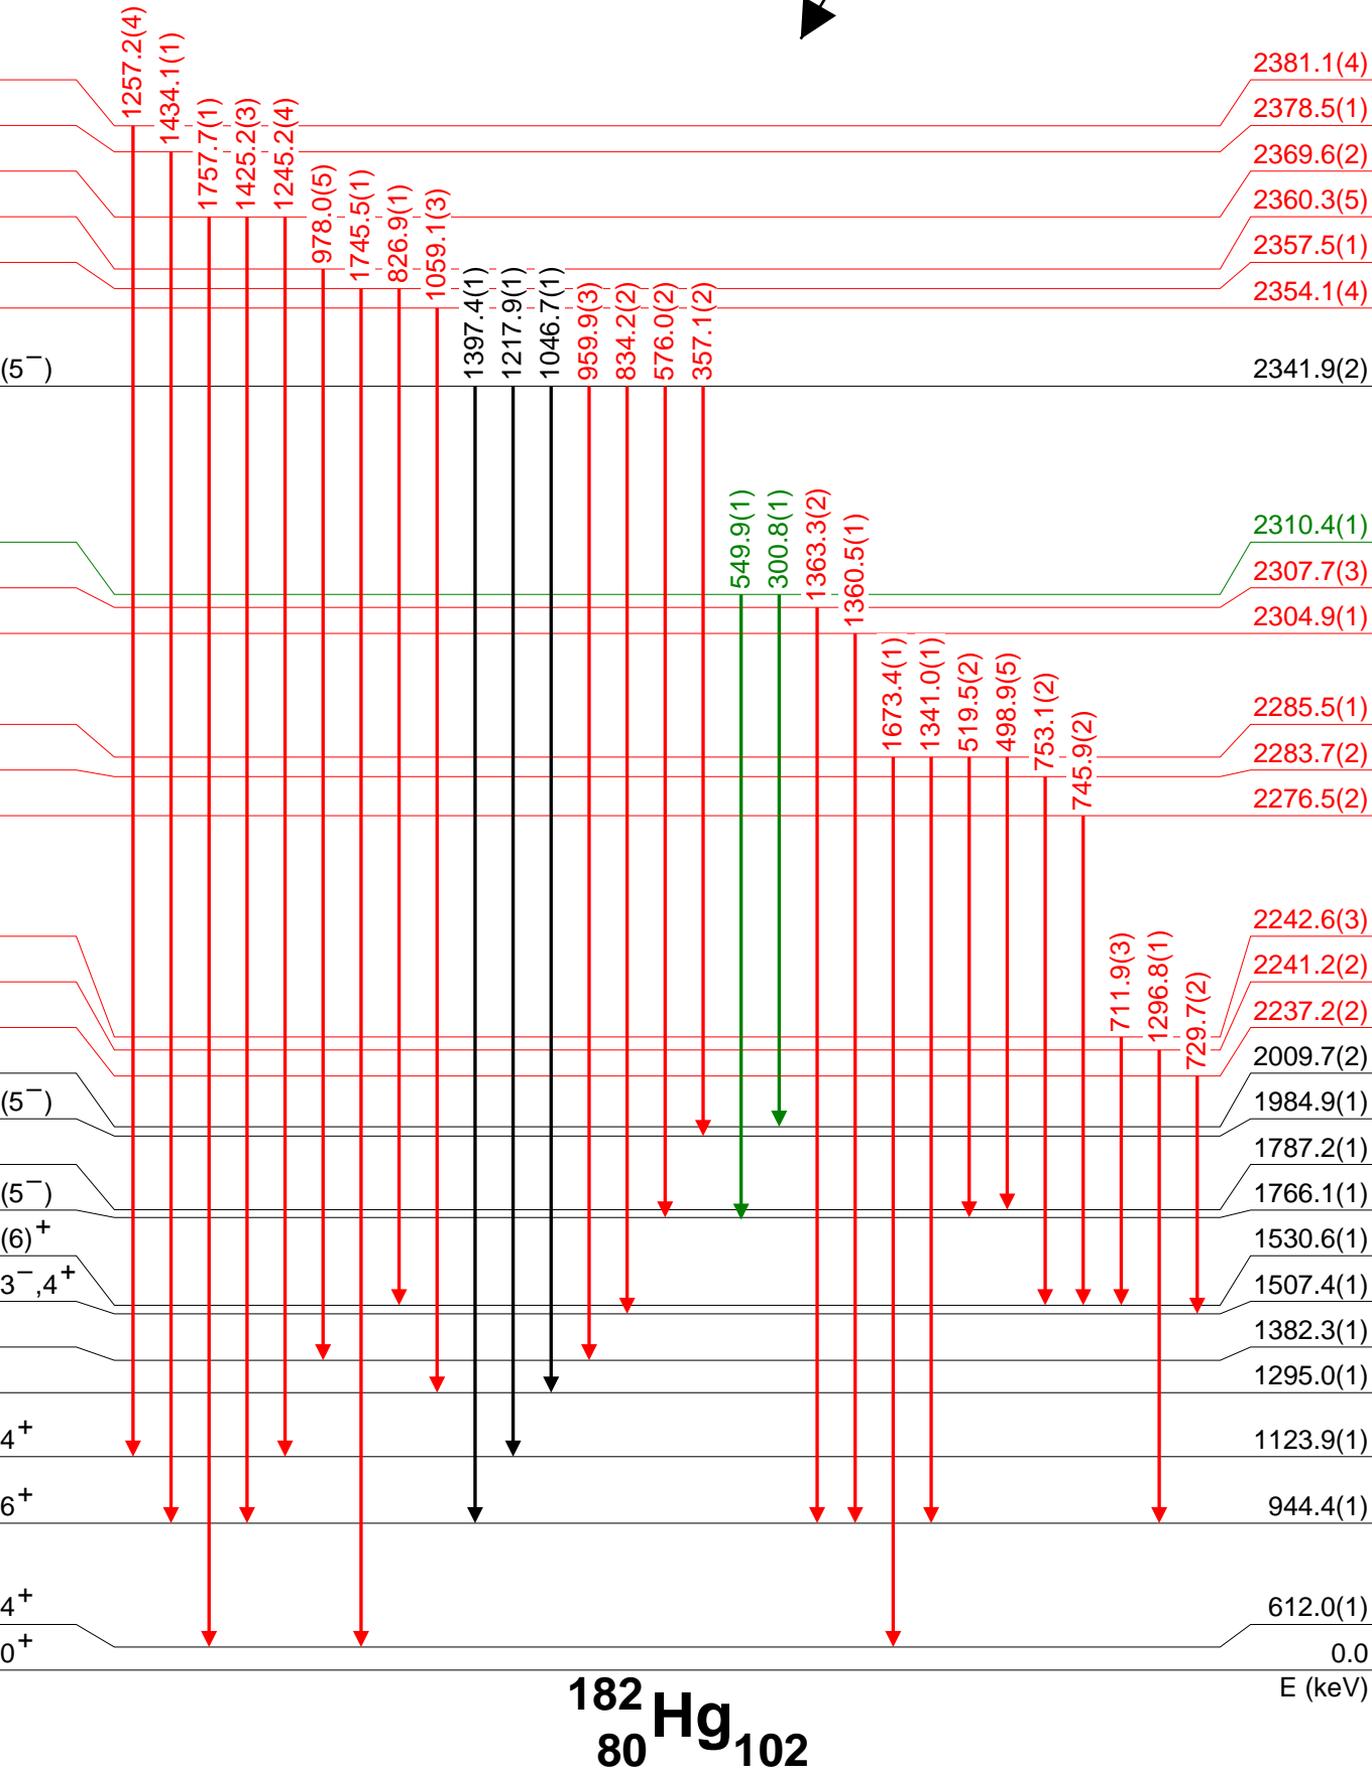

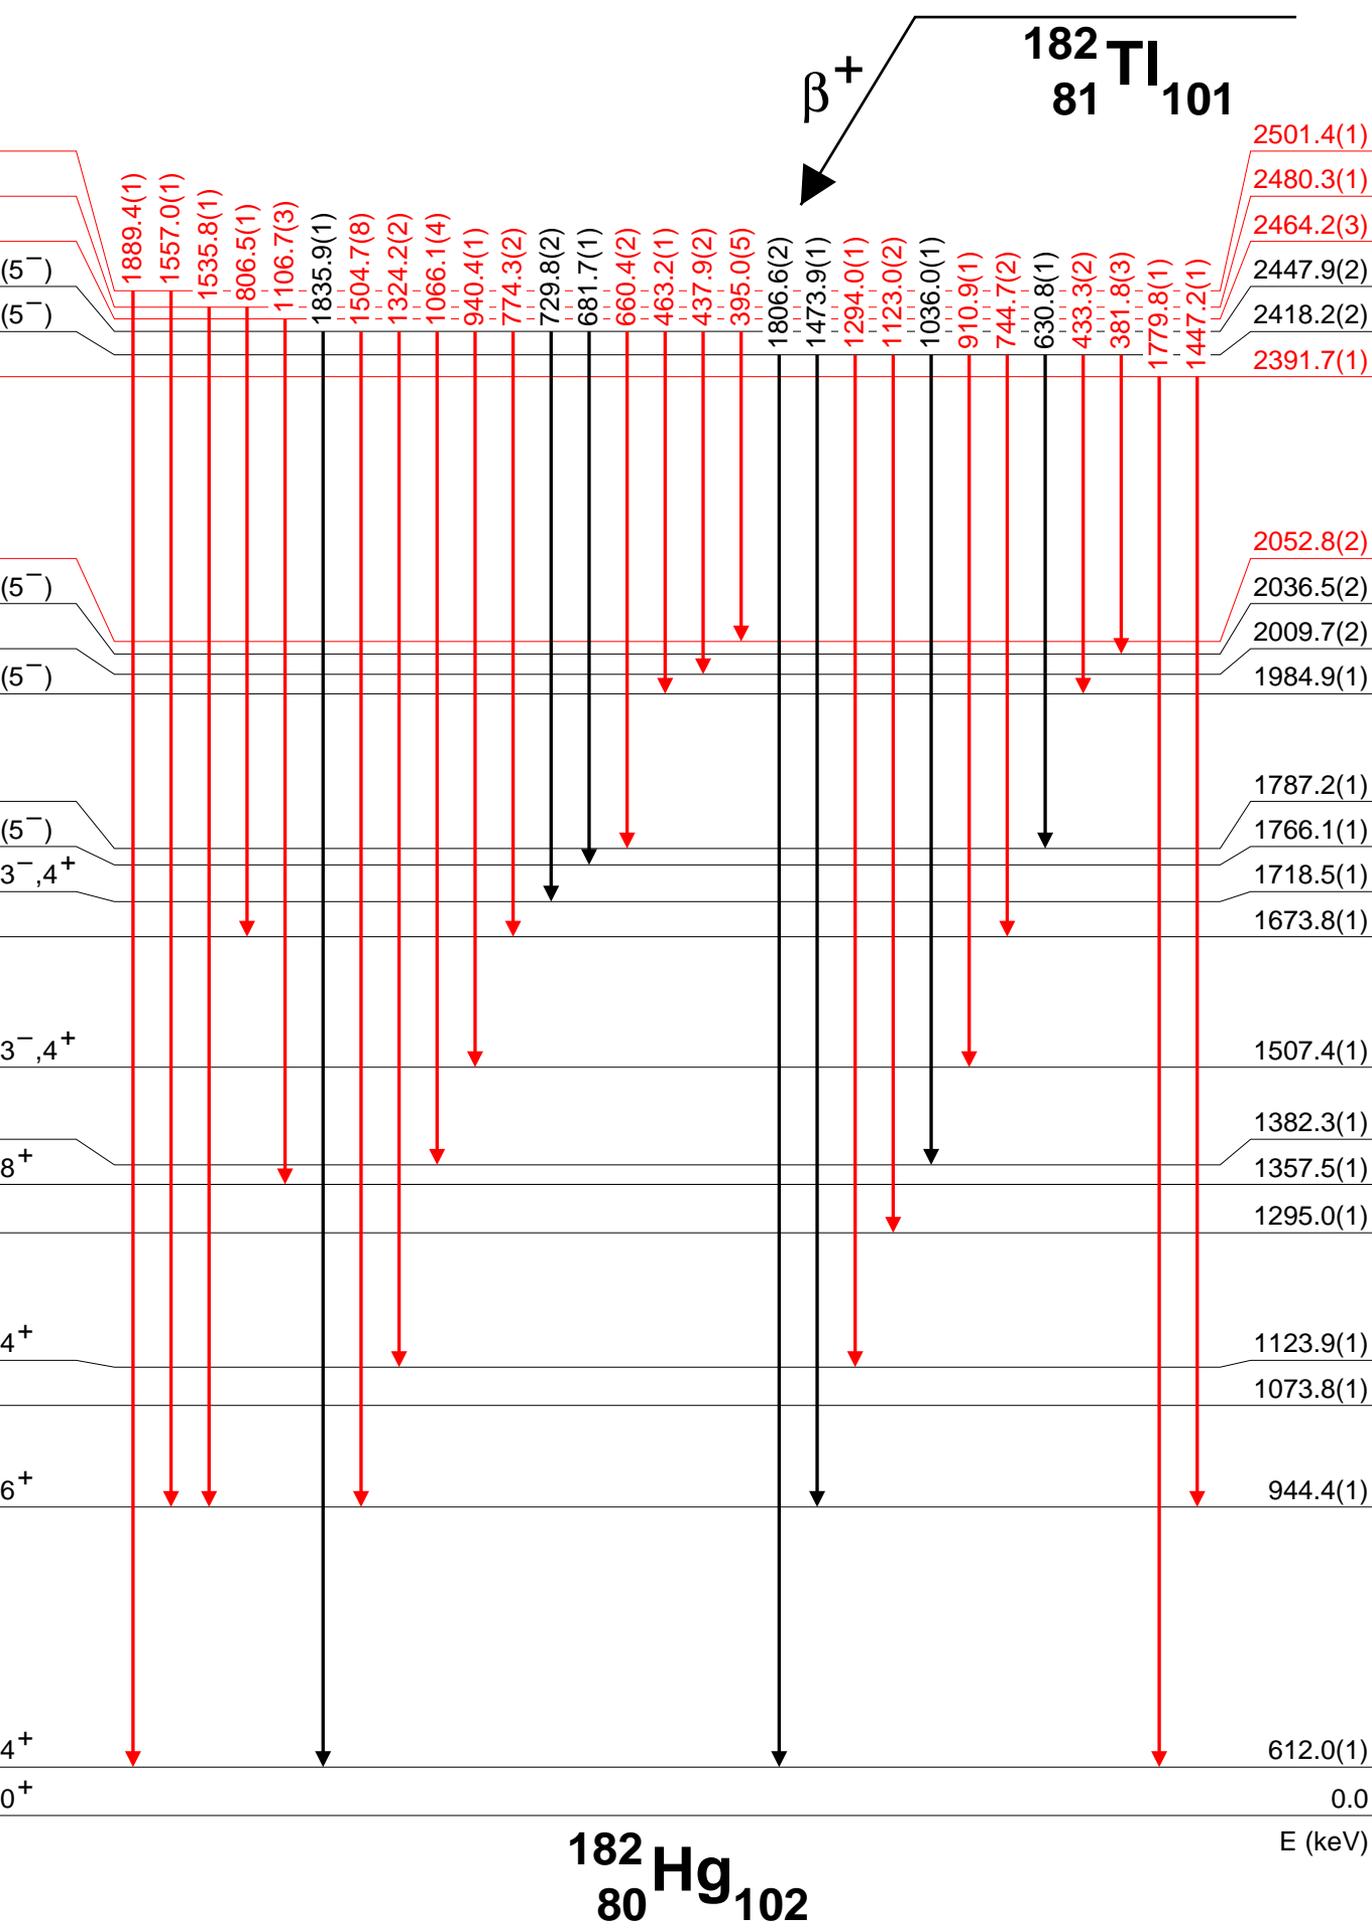

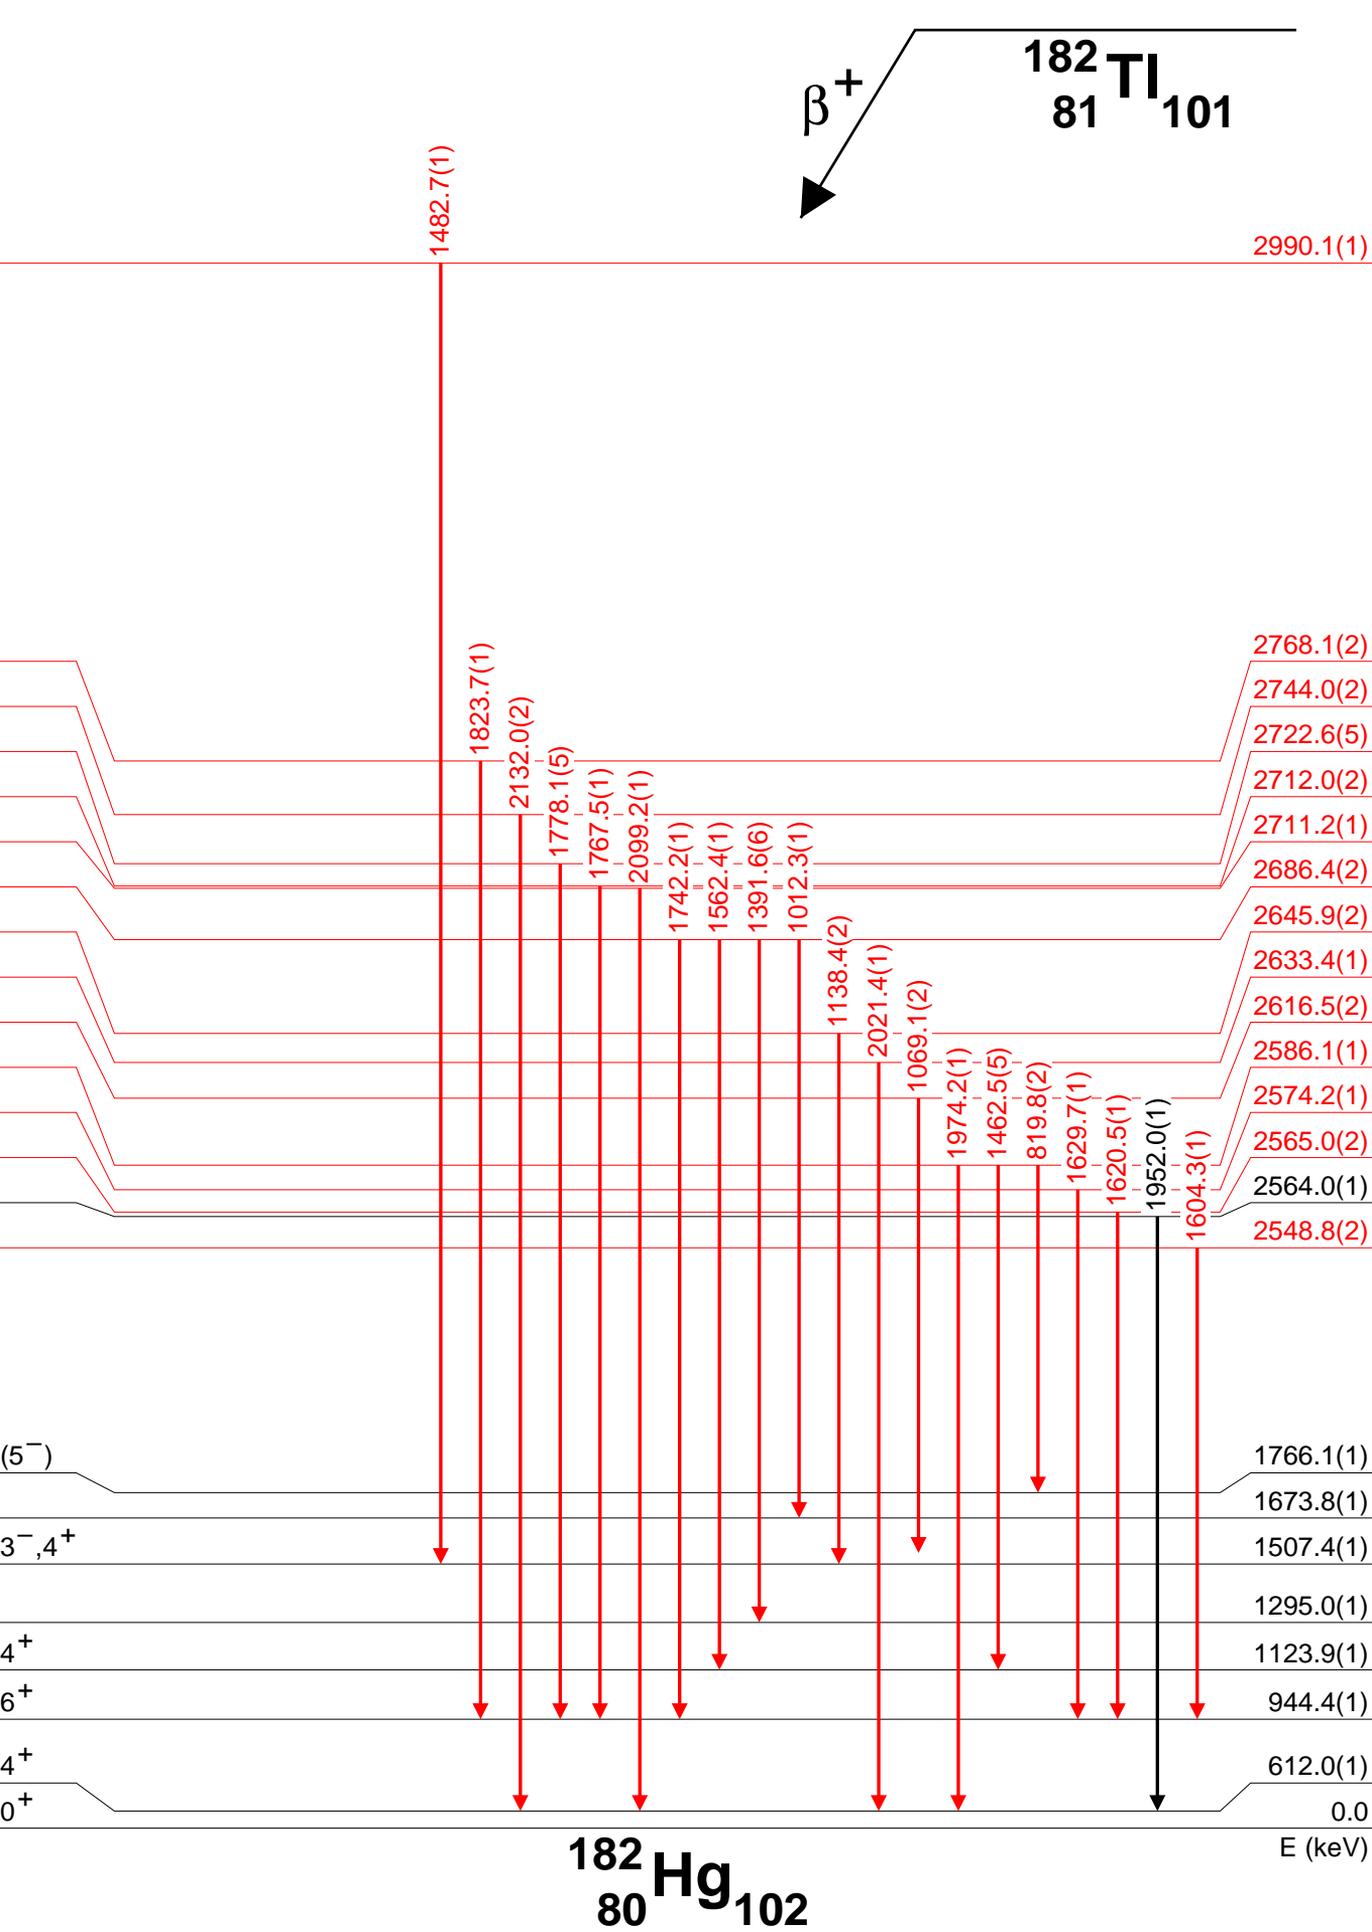

Supplement: Supplementary file 2 [file 20230308_182Hg_decayscheme.pdf]
