# Supplementary material for: Simultaneous $\gamma$-ray and electron spectroscopy of $^{182,184,186}$Hg isotopes
Source: arXiv:2305.16442 ancillary file (2023-06-06)

$\beta^+$   $^{184}_{81}\text{Tl}_{103}$

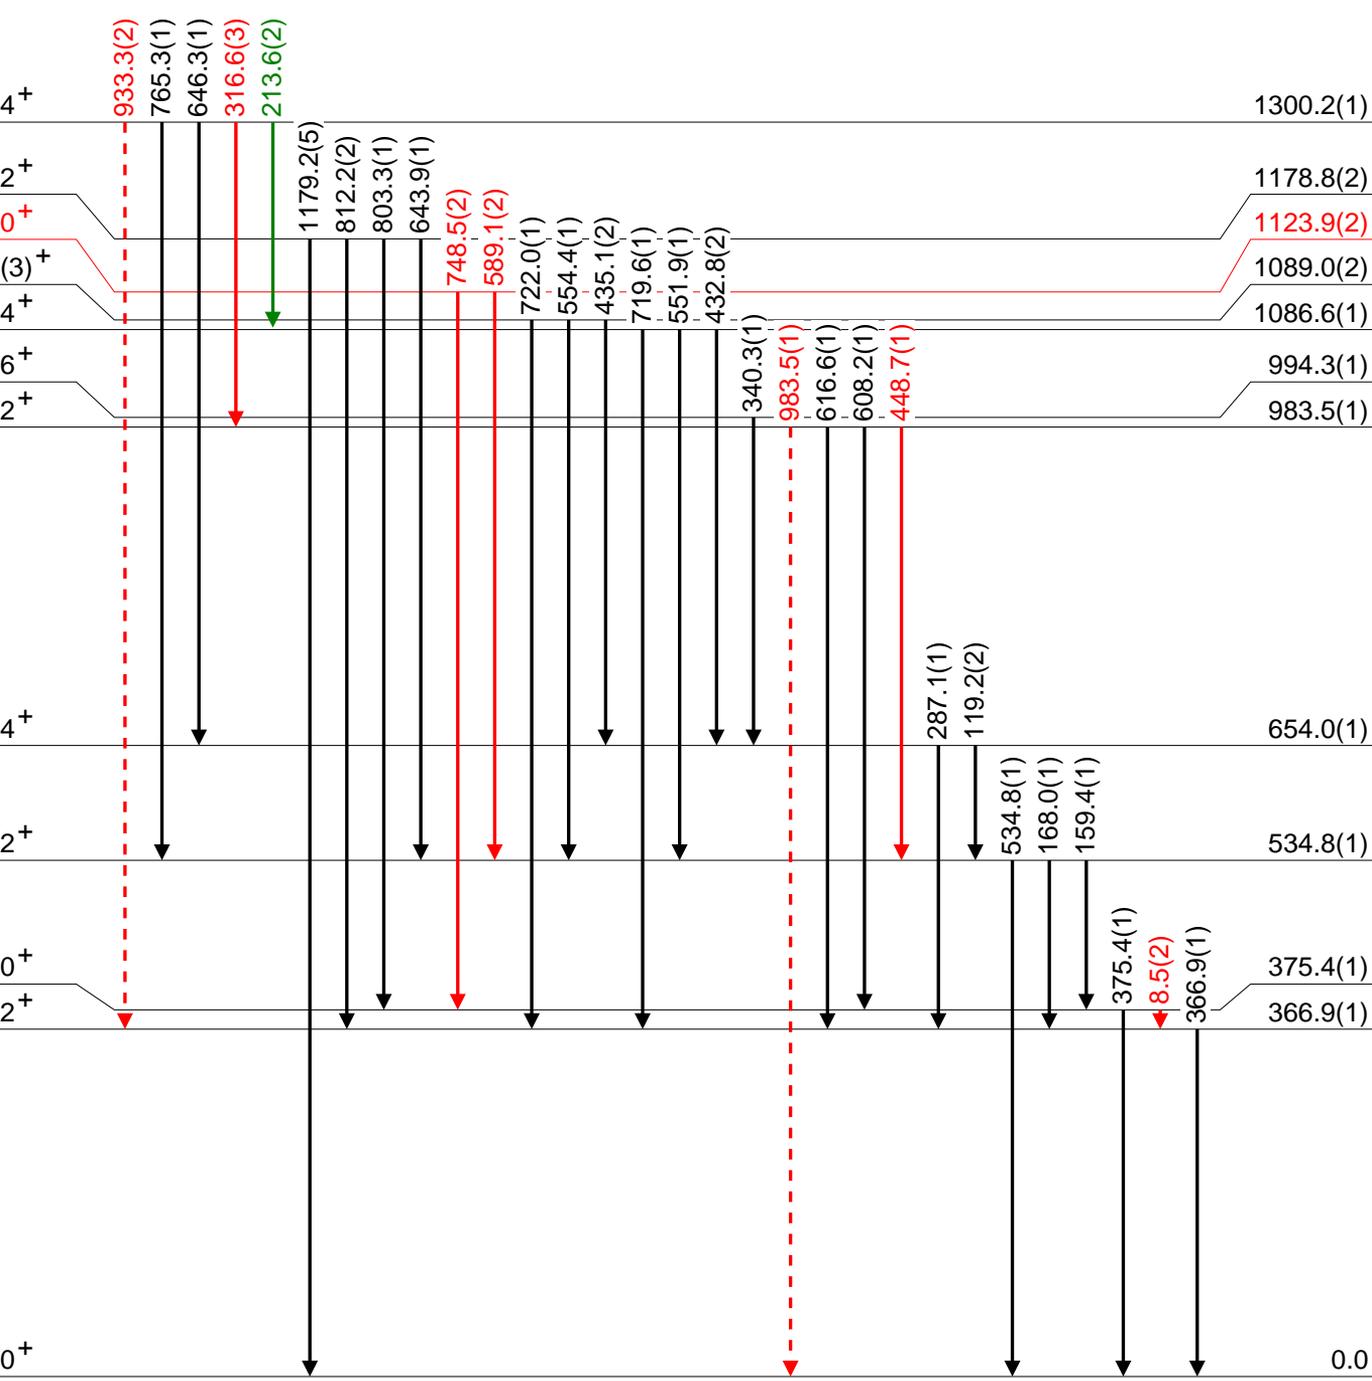

$^{184}_{80}\text{Hg}_{104}$

E (keV)

$\beta^+$   $^{184}_{81}\text{Tl}_{103}$

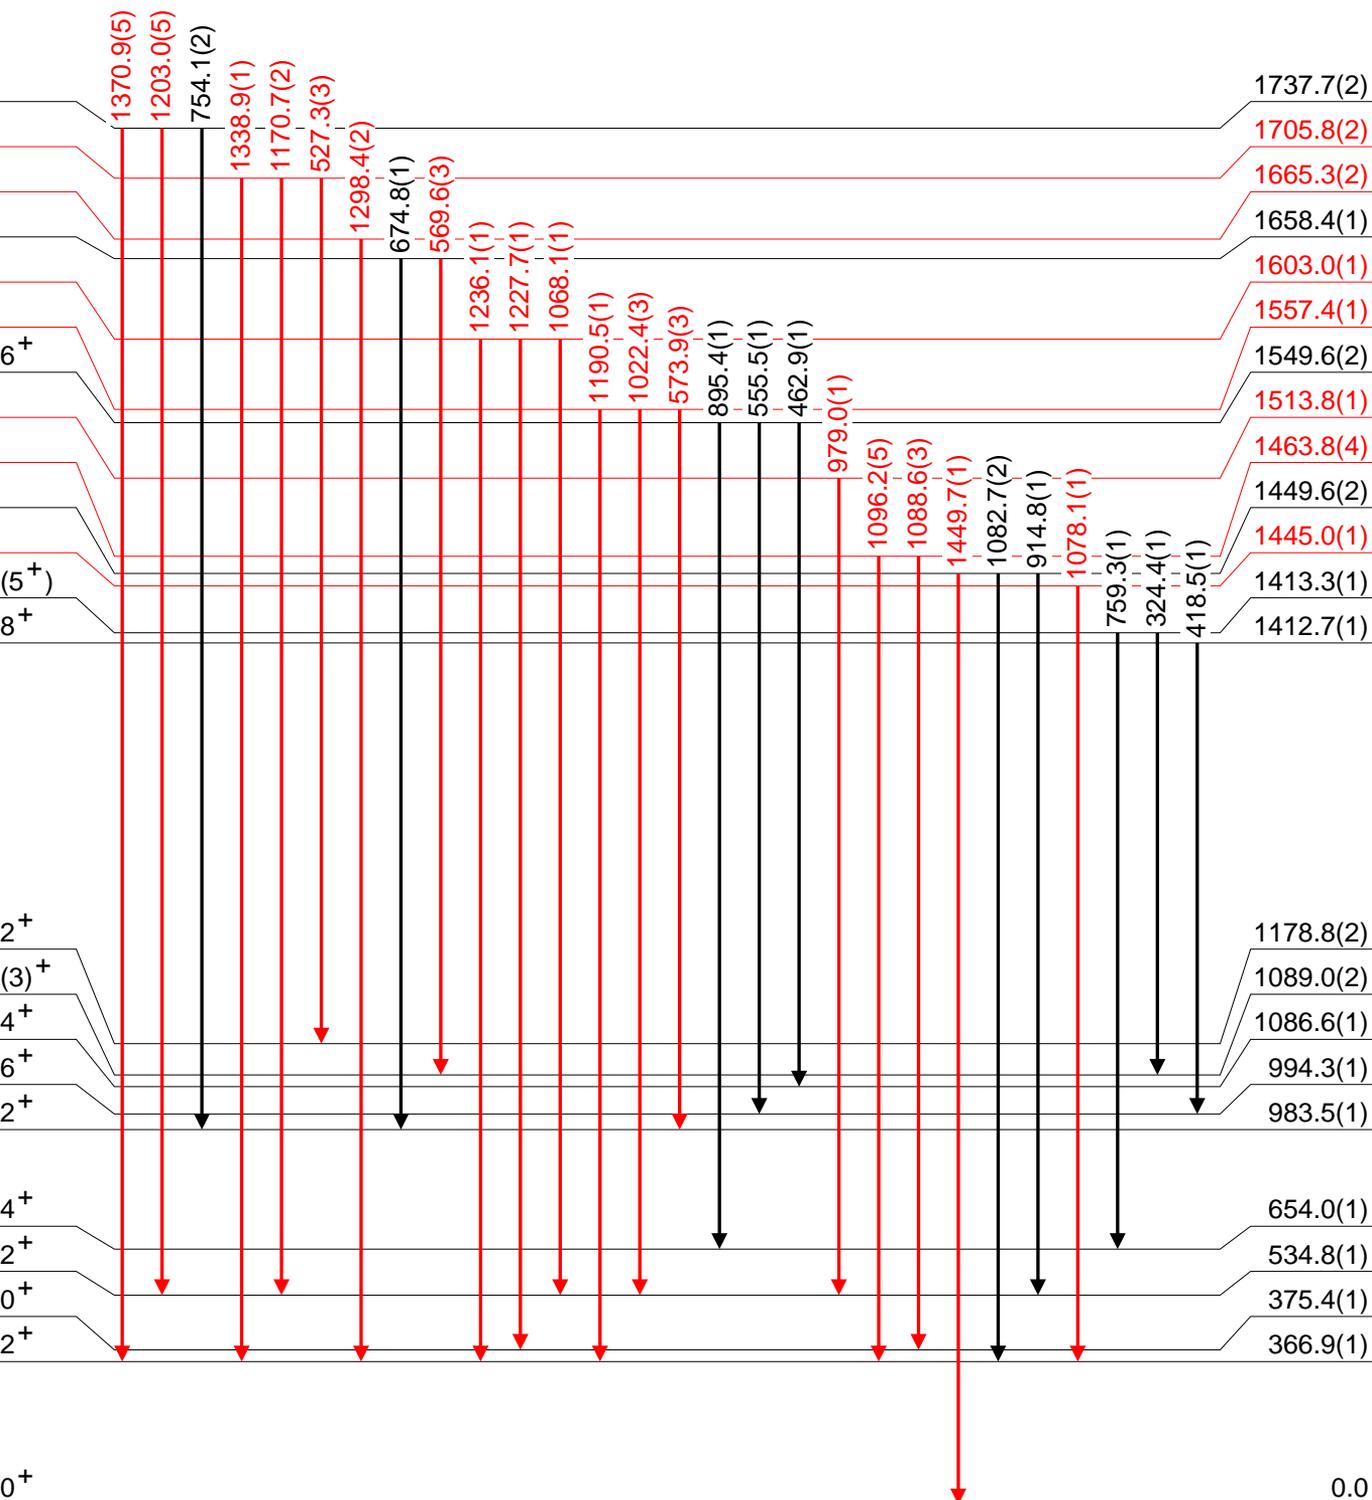

$^{184}_{80}\text{Hg}_{104}$

E (keV)

$\beta^+$   $^{184}_{81}\text{Tl}_{103}$

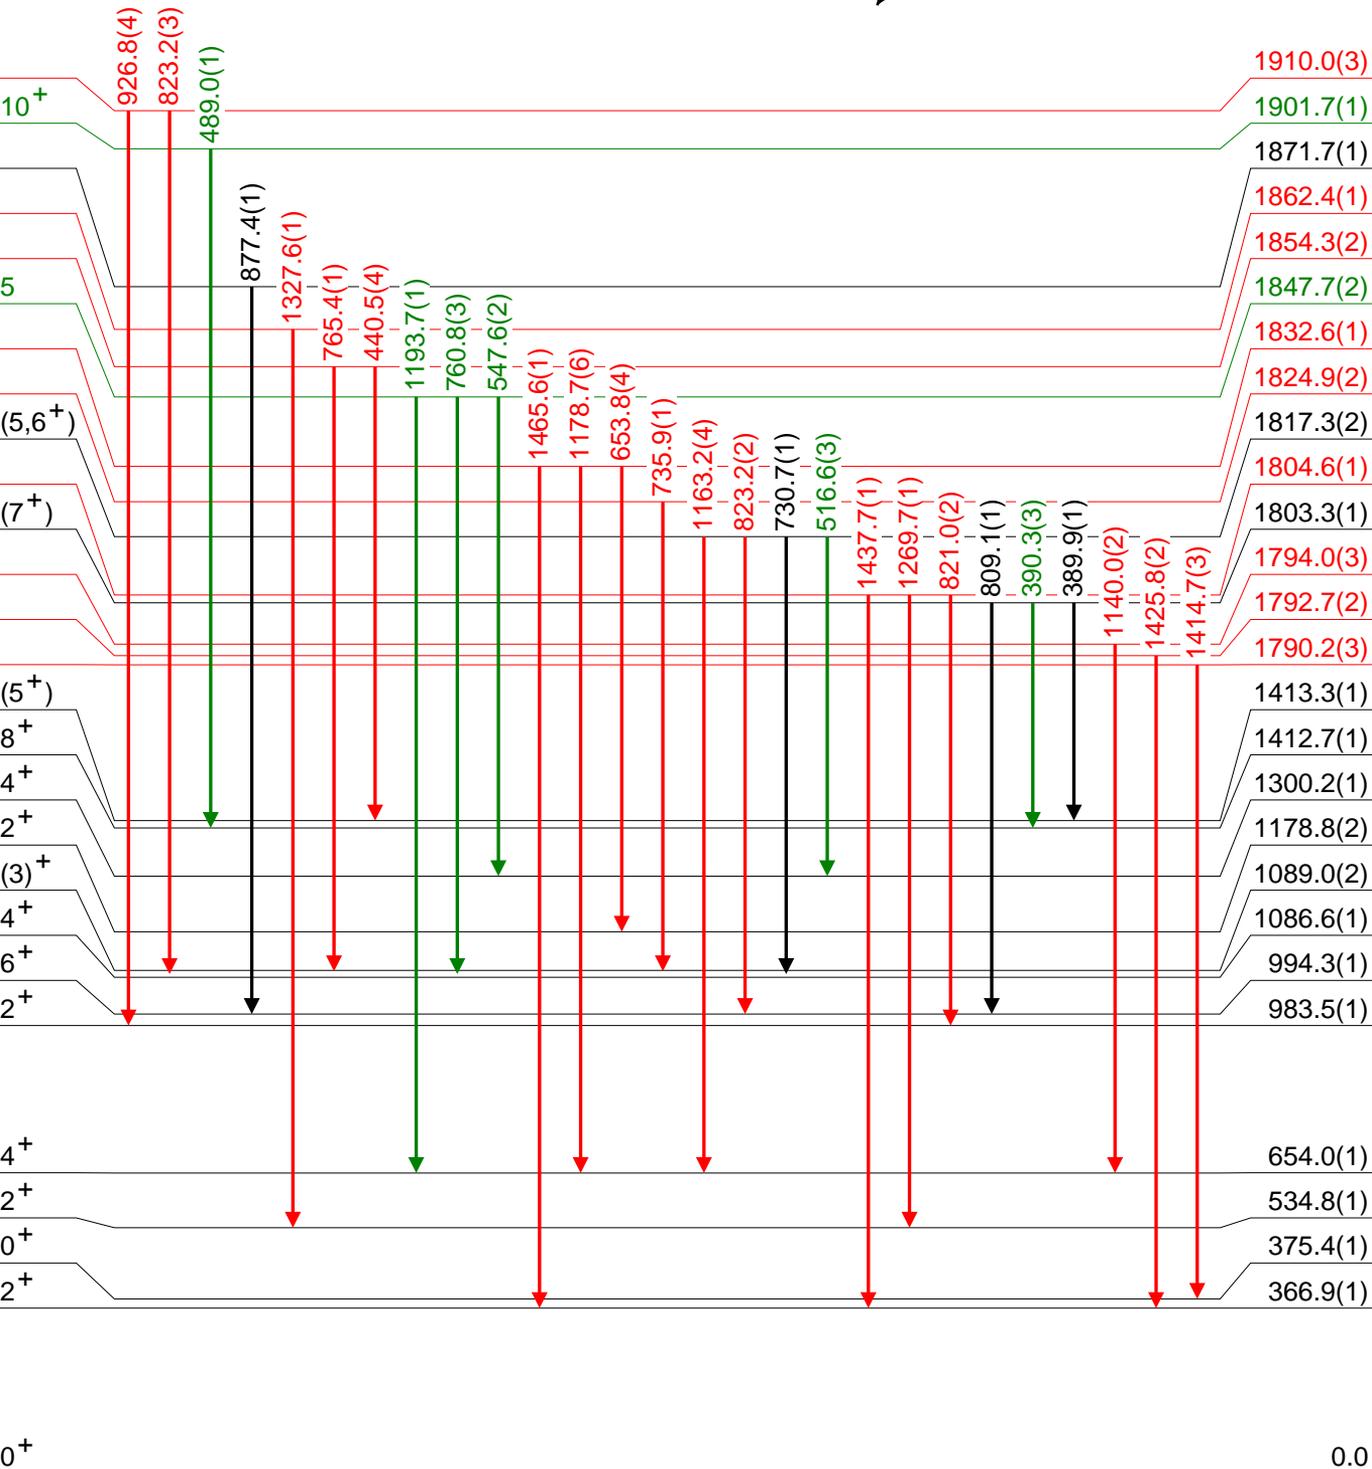

$^{184}_{80}\text{Hg}_{104}$

0.0  
E (keV)

$\beta^+$   
 $^{184}_{81}\text{Tl}_{103}$

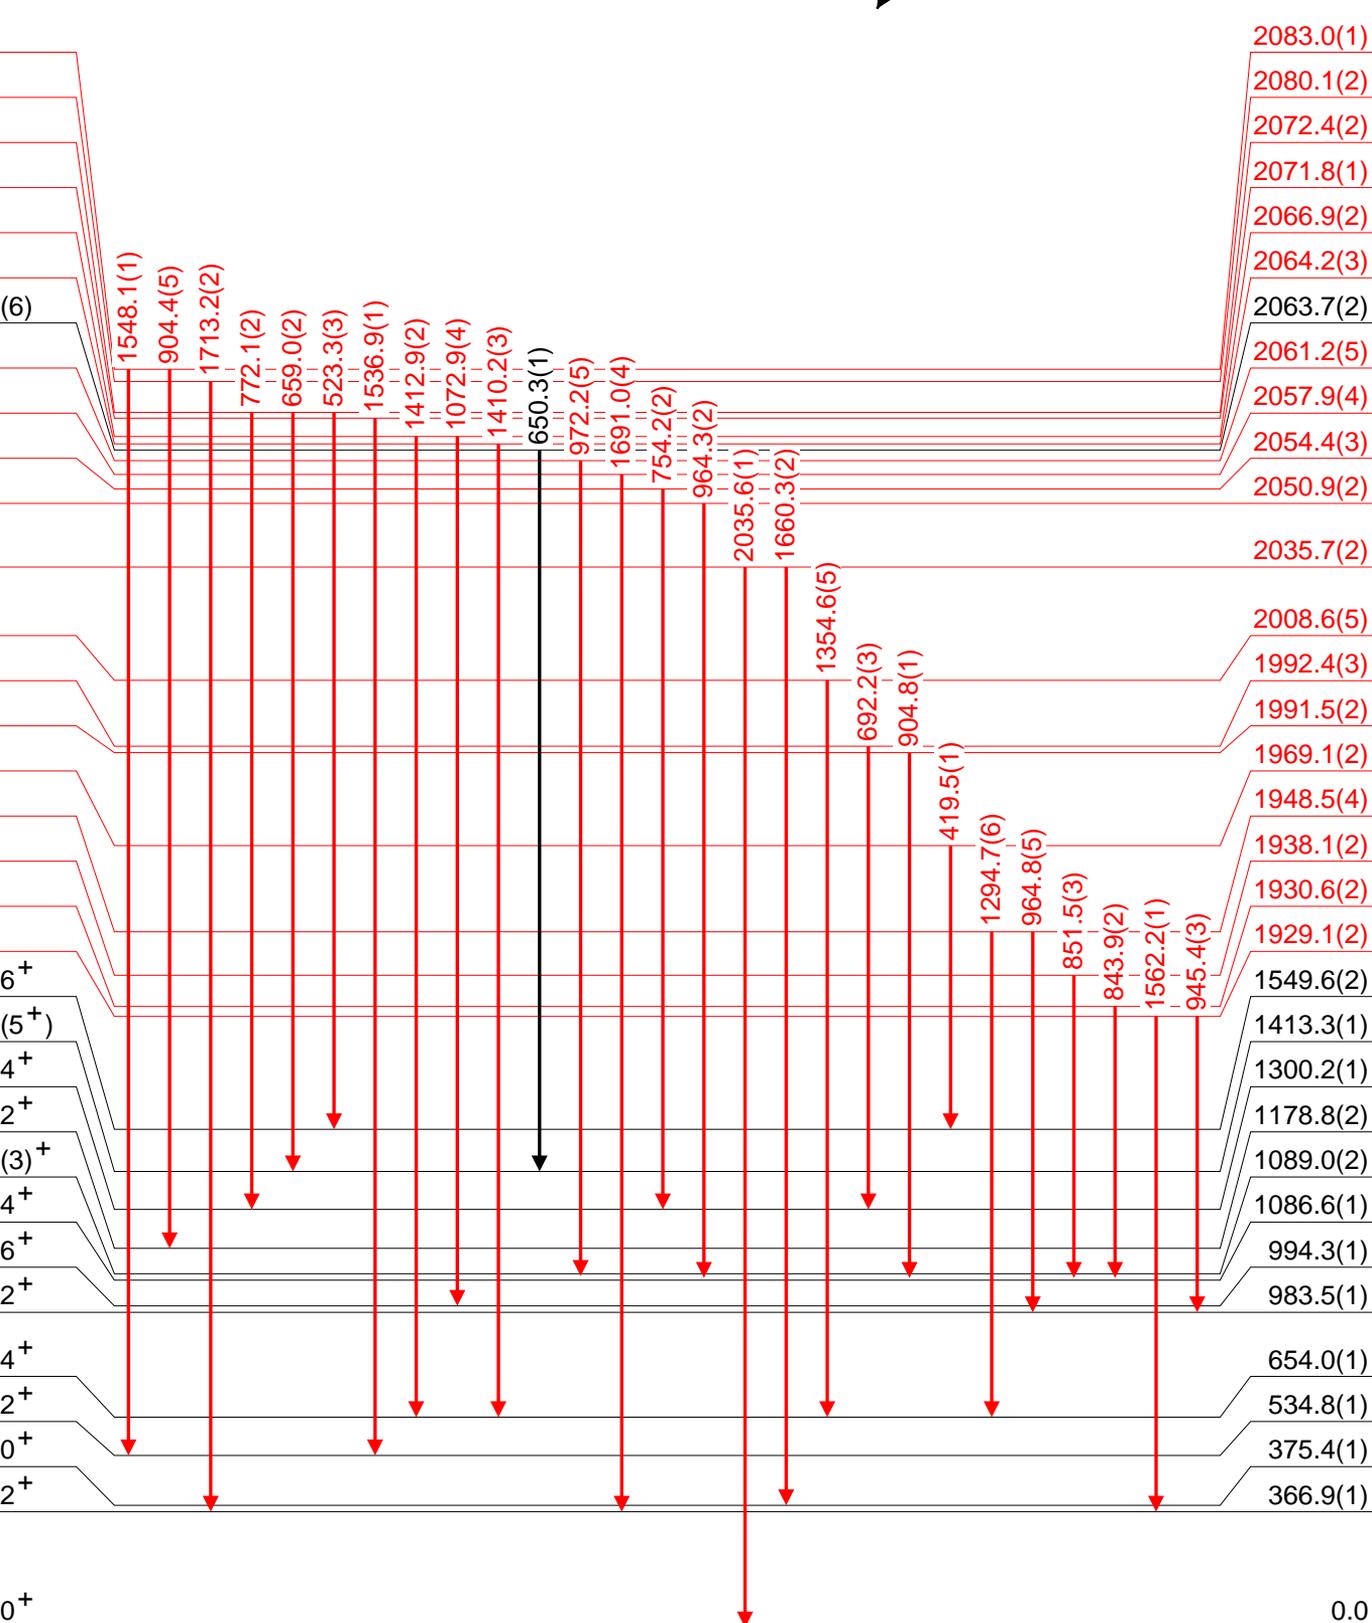

$^{184}_{80}\text{Hg}_{104}$

0.0  
 E (keV)

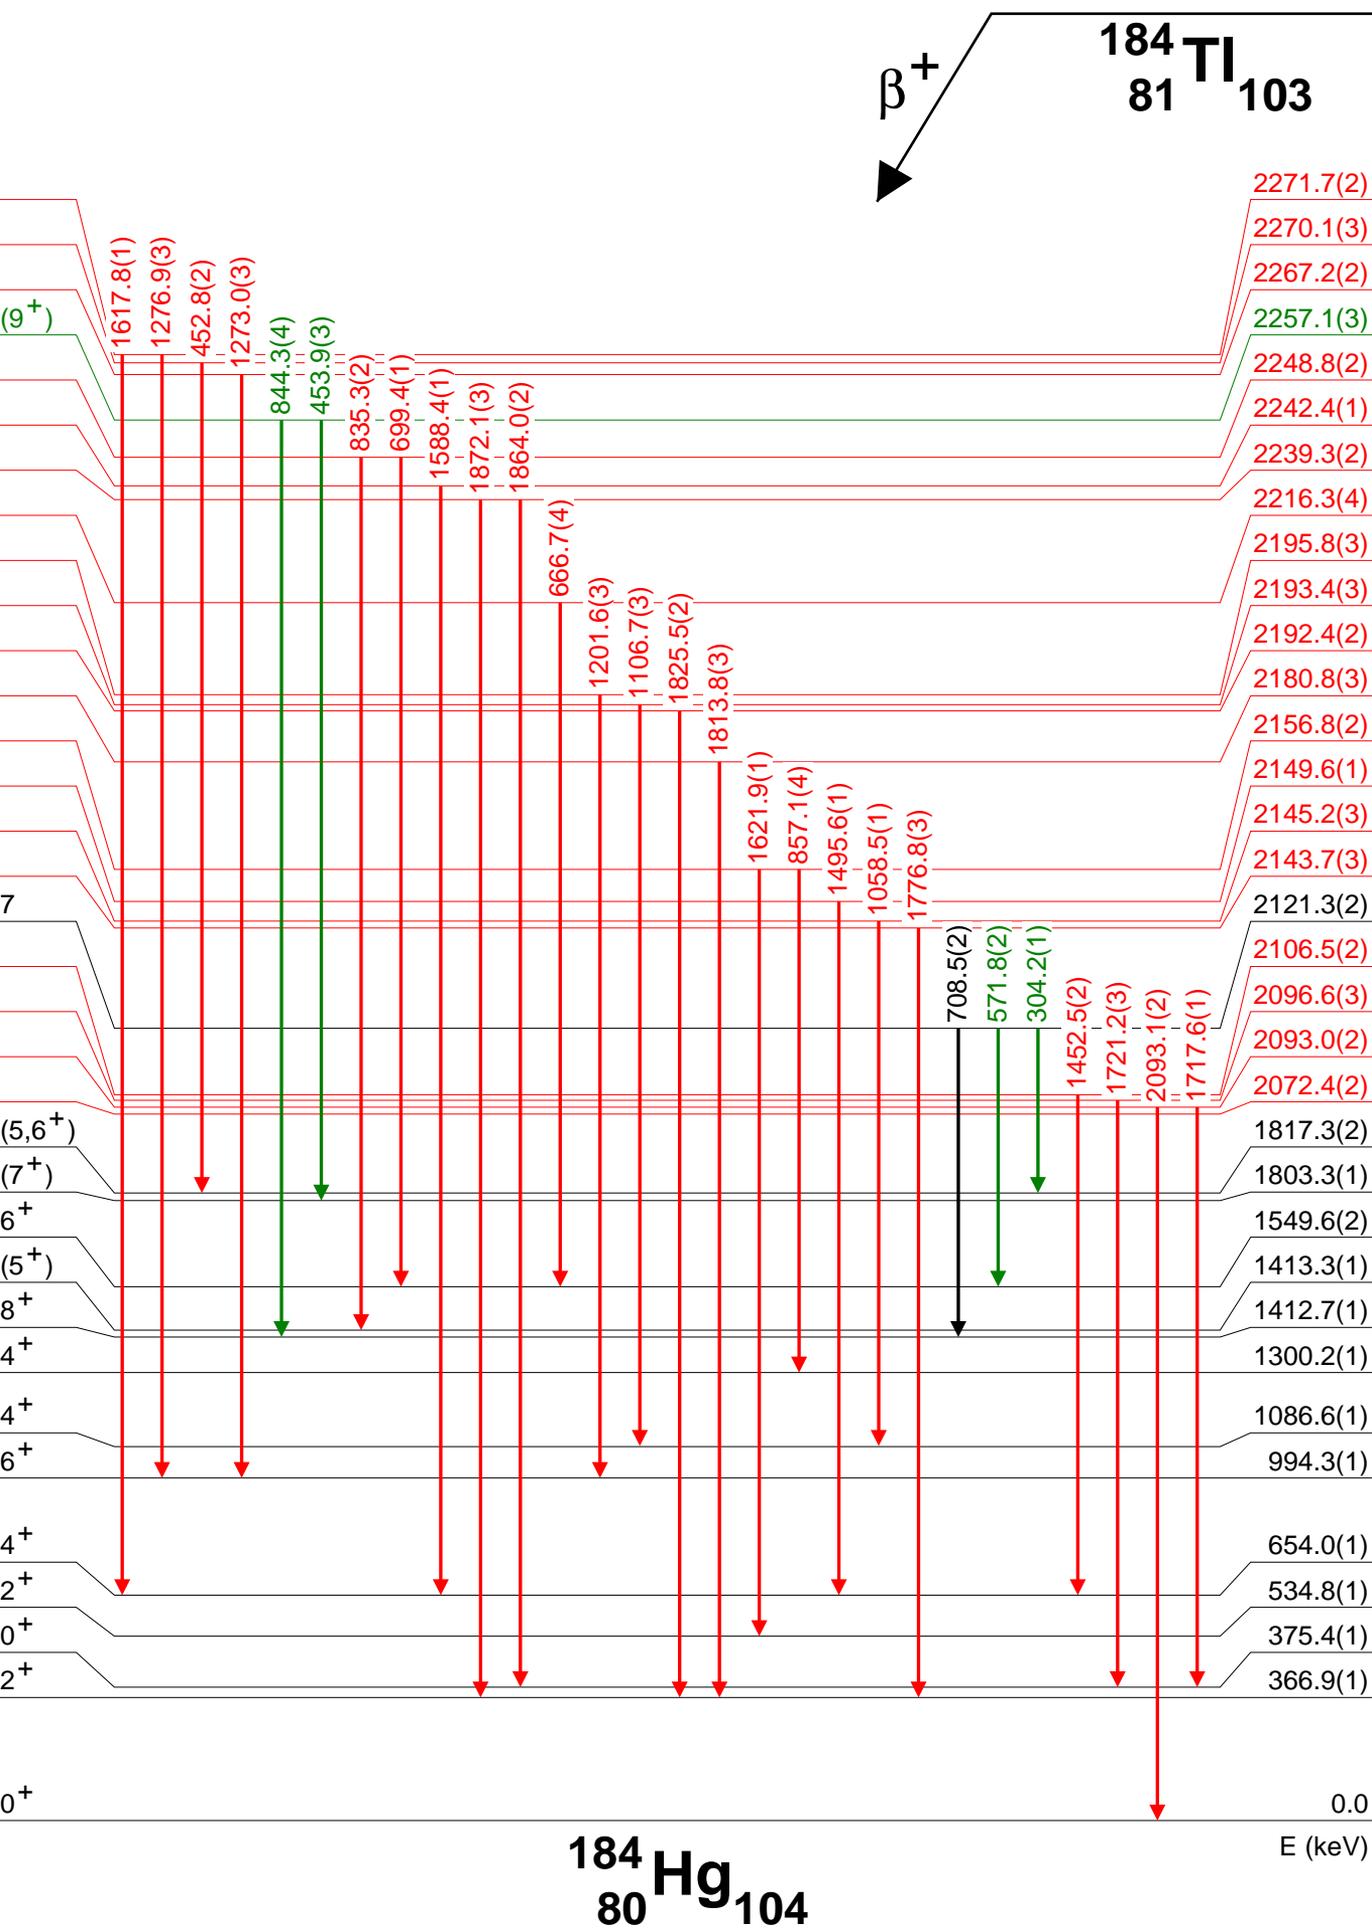

$\beta^+$  $^{184}_{81}\text{Tl}_{103}$ 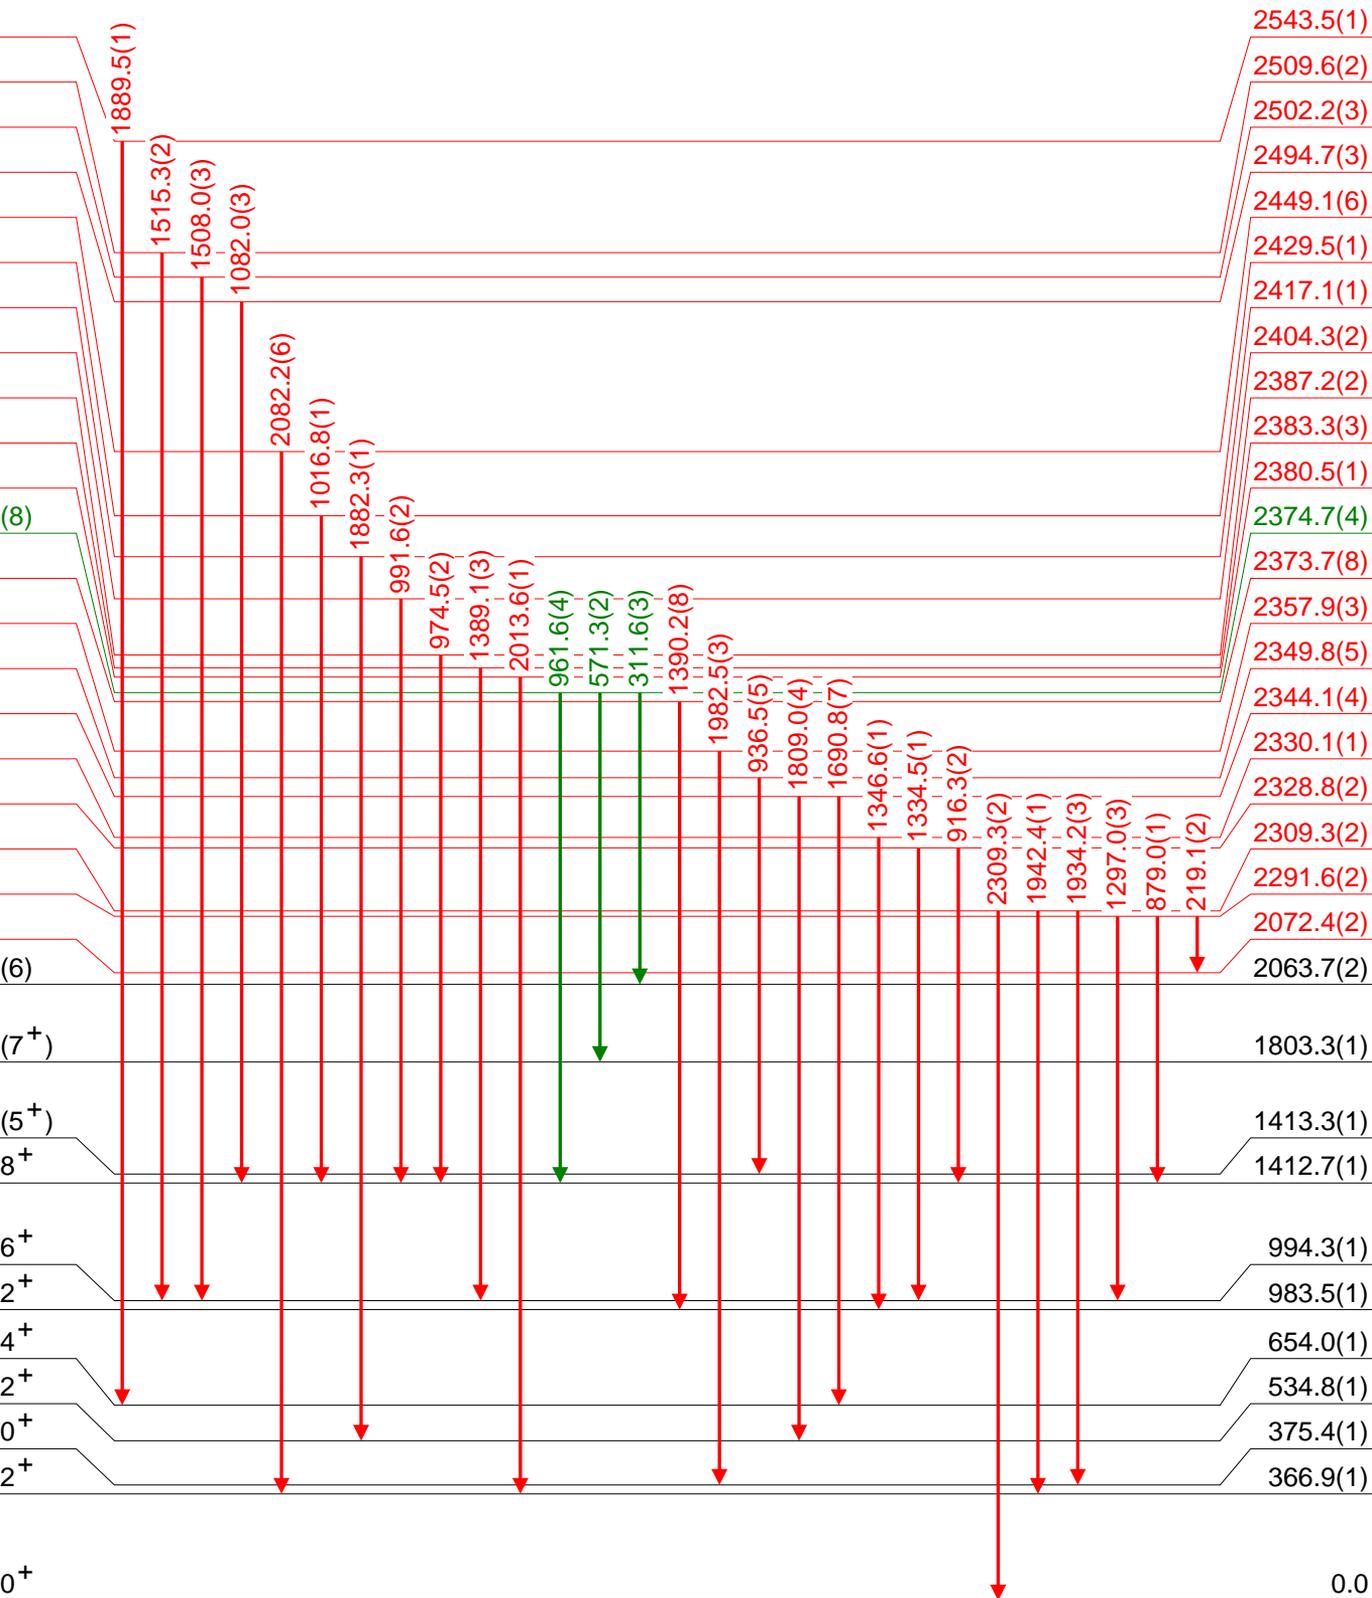 $^{184}_{80}\text{Hg}_{104}$ 

E (keV)

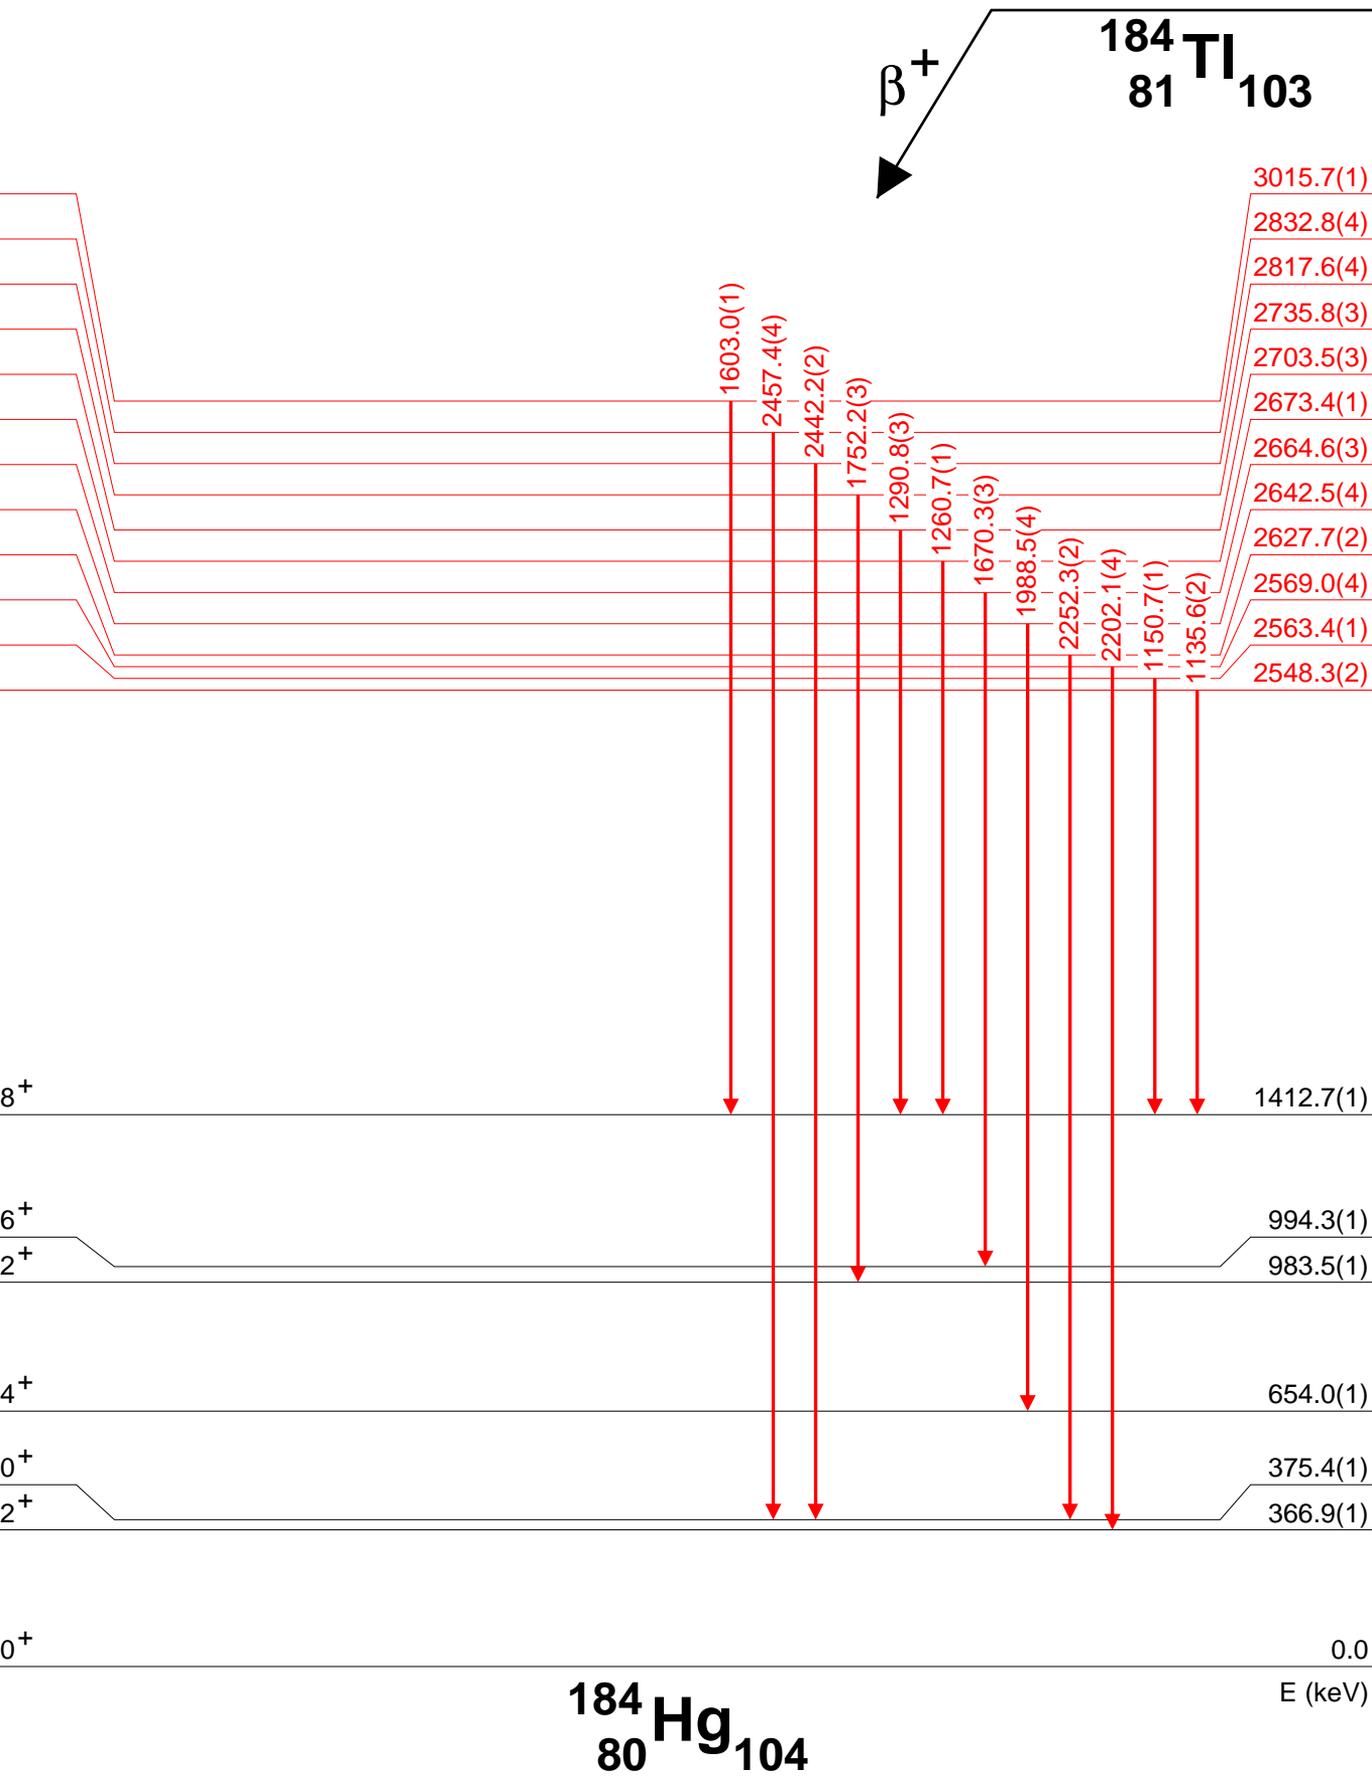

Supplement: Supplementary file 3 [file 20230308_184Hg_decayscheme.pdf]
