# Supplementary material for: Simultaneous $\gamma$-ray and electron spectroscopy of $^{182,184,186}$Hg isotopes
Source: arXiv:2305.16442 ancillary file (2023-06-06)

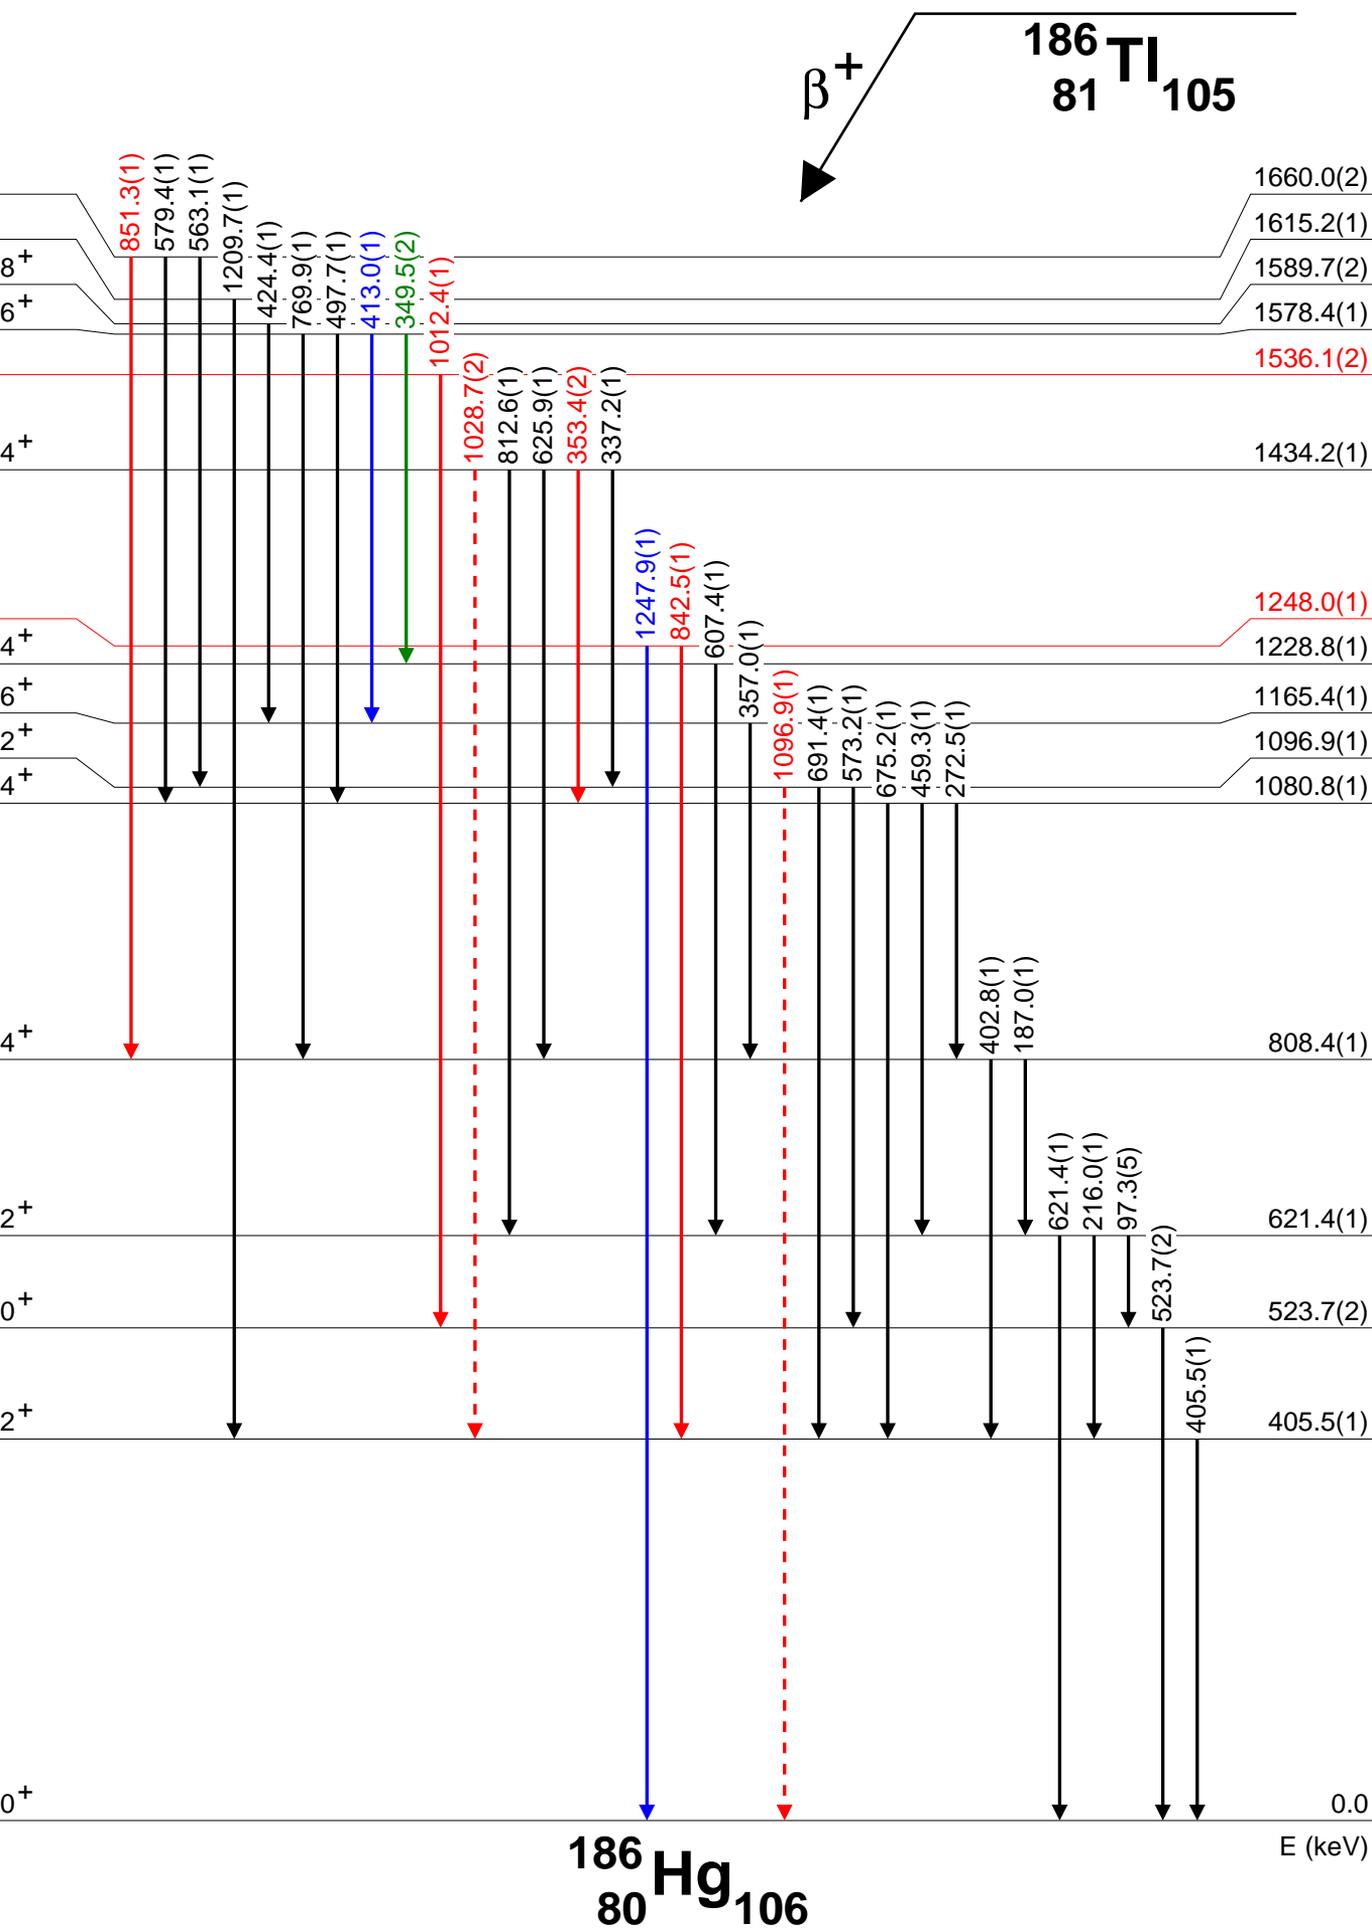

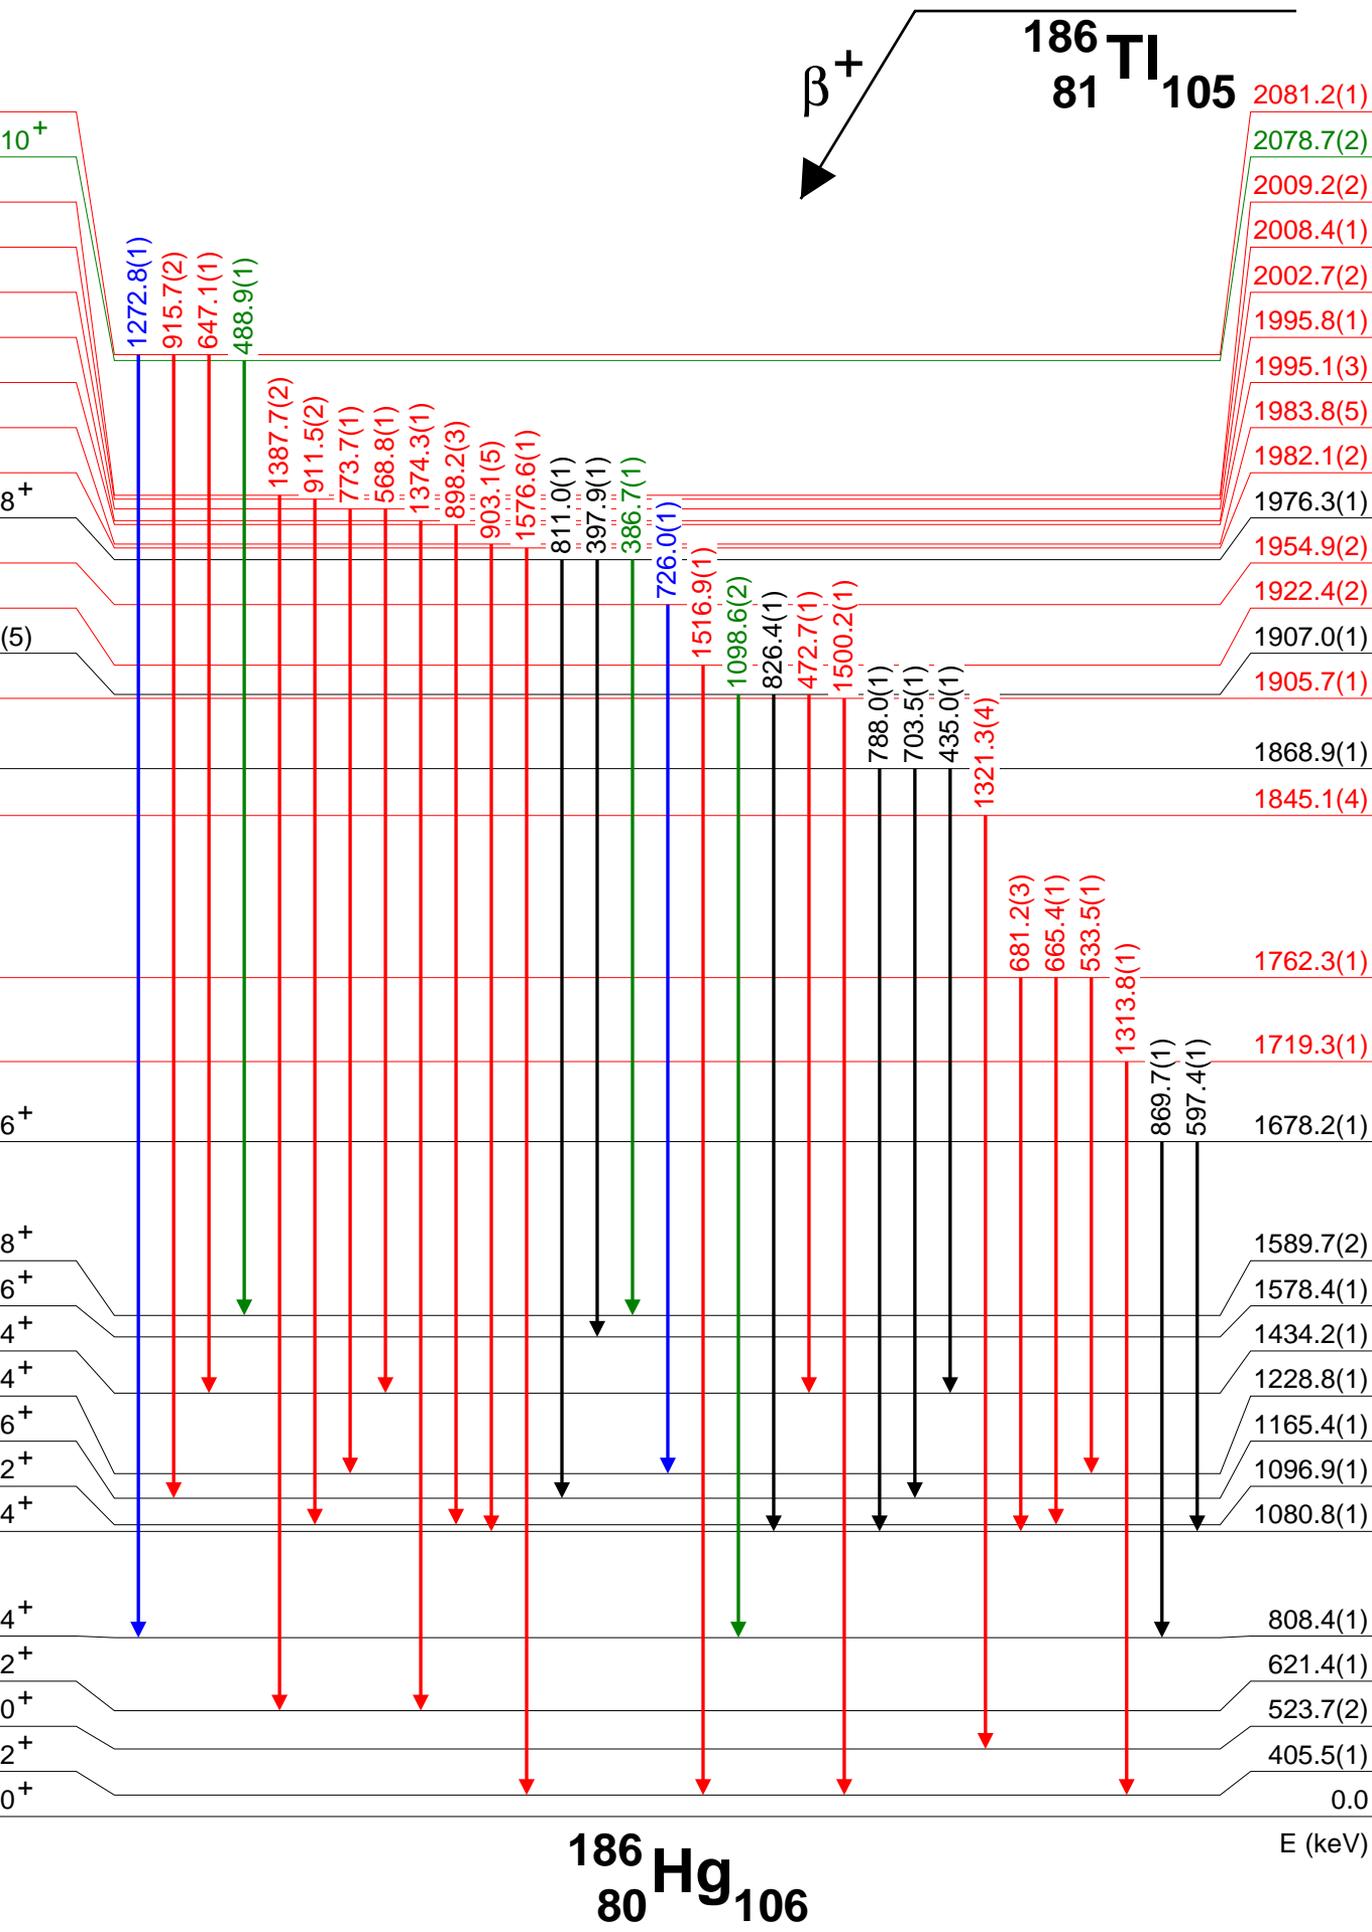

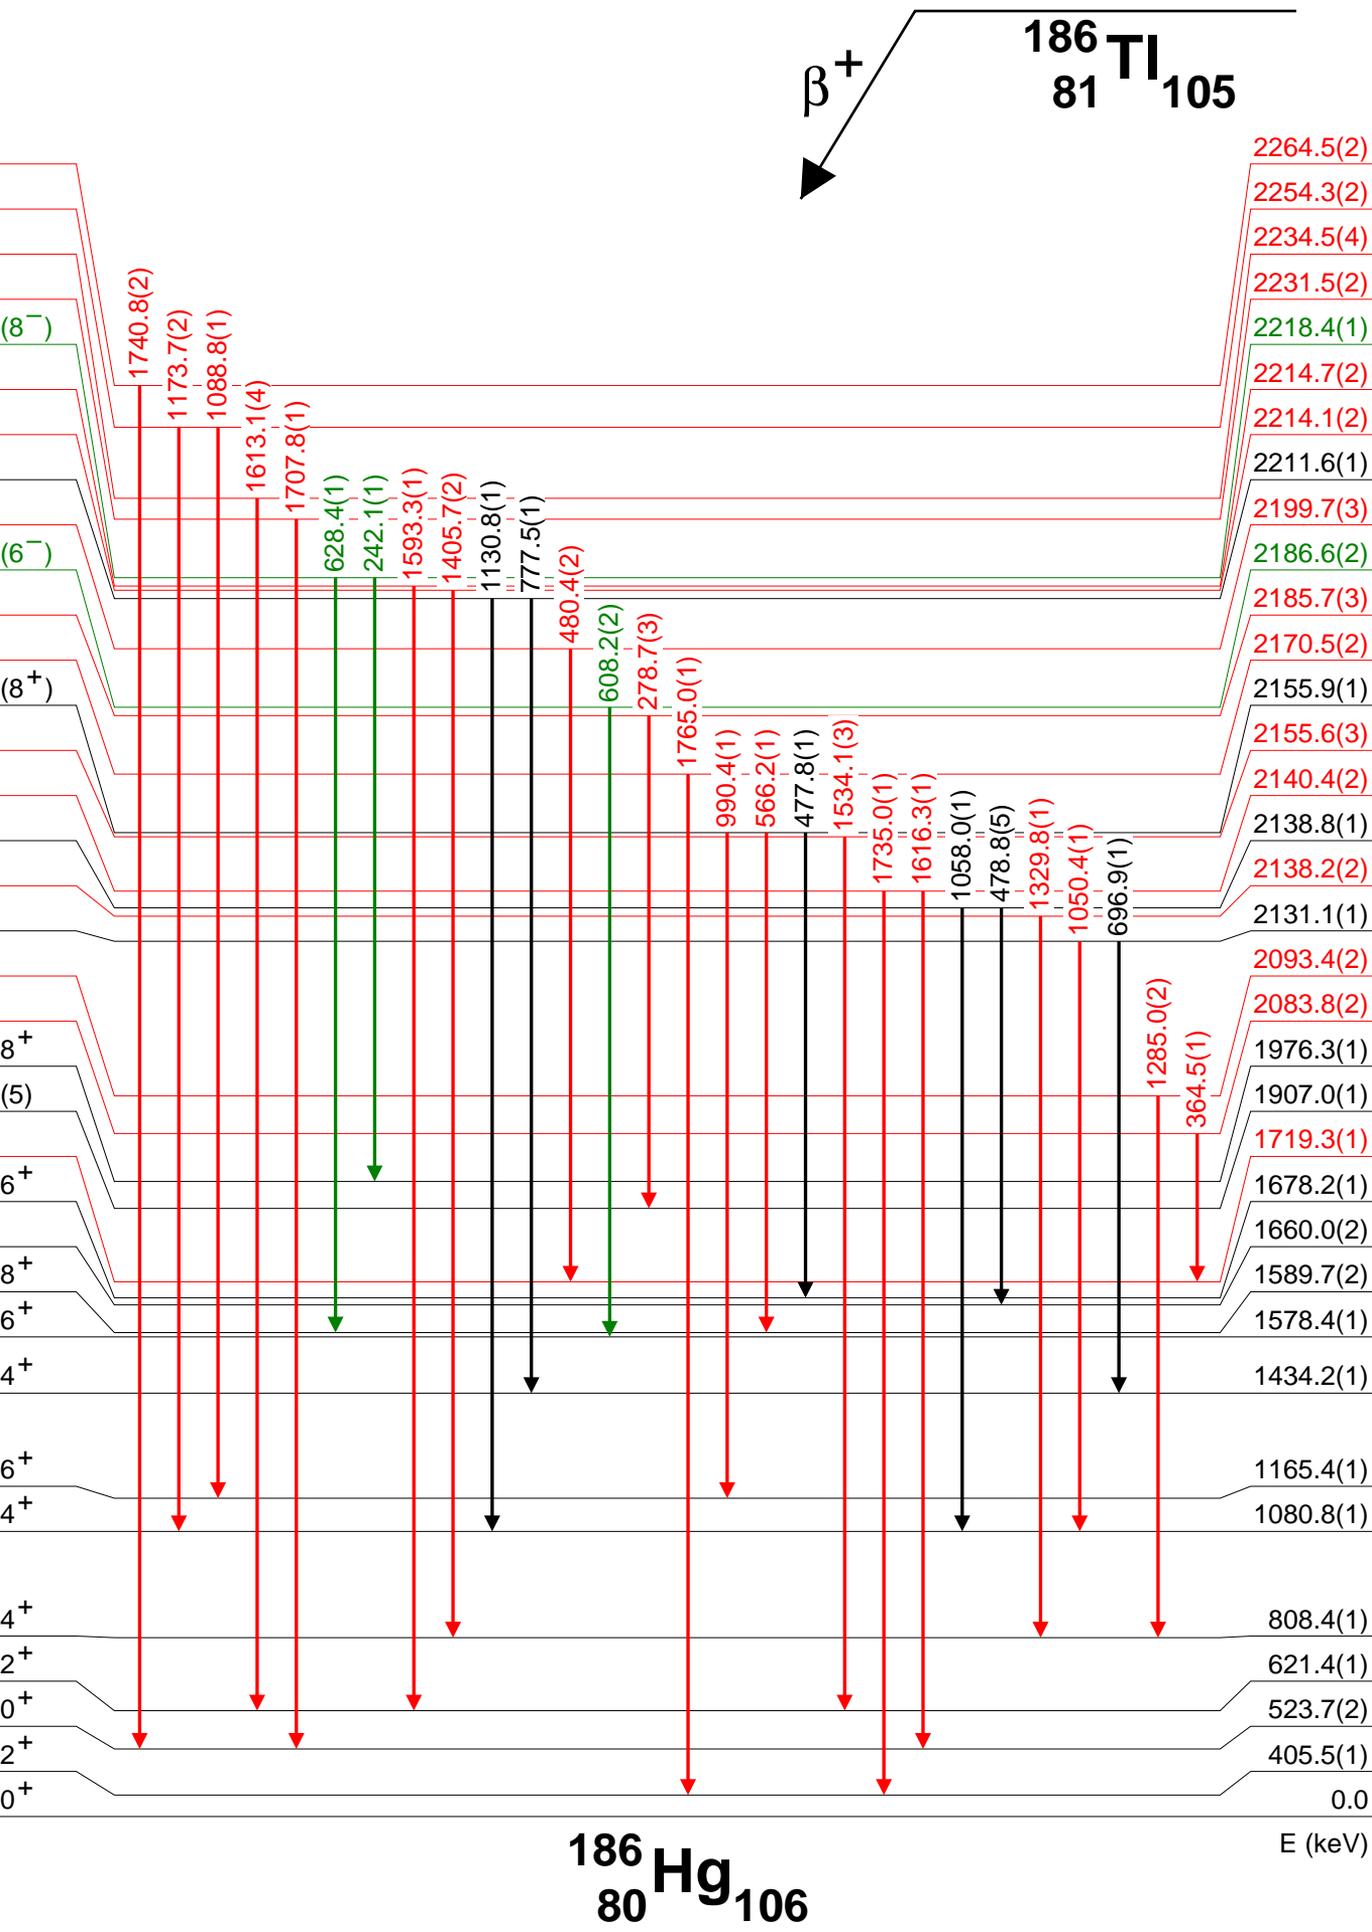



$\beta^+$   $^{186}_{81}\text{Tl}_{105}$

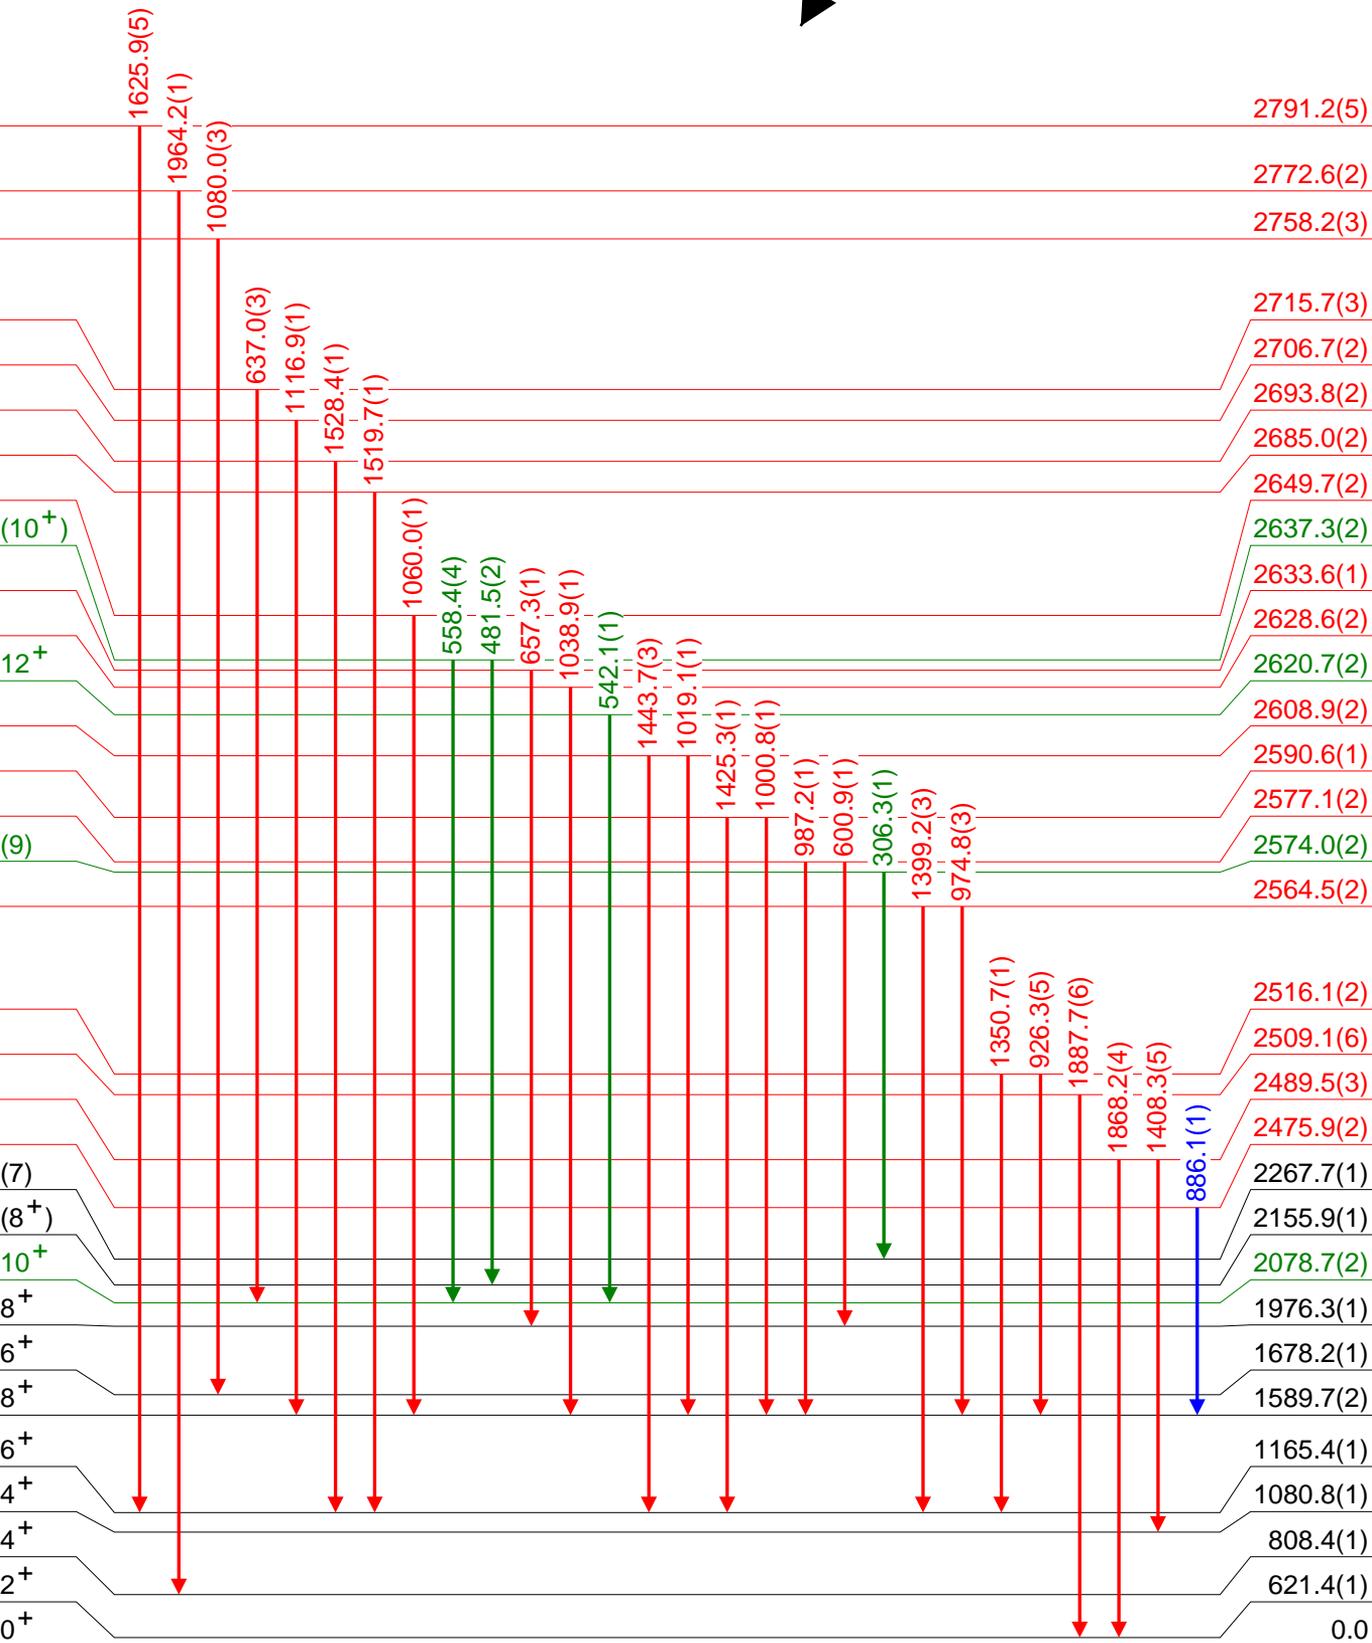

$^{186}_{80}\text{Hg}_{106}$

E (keV)

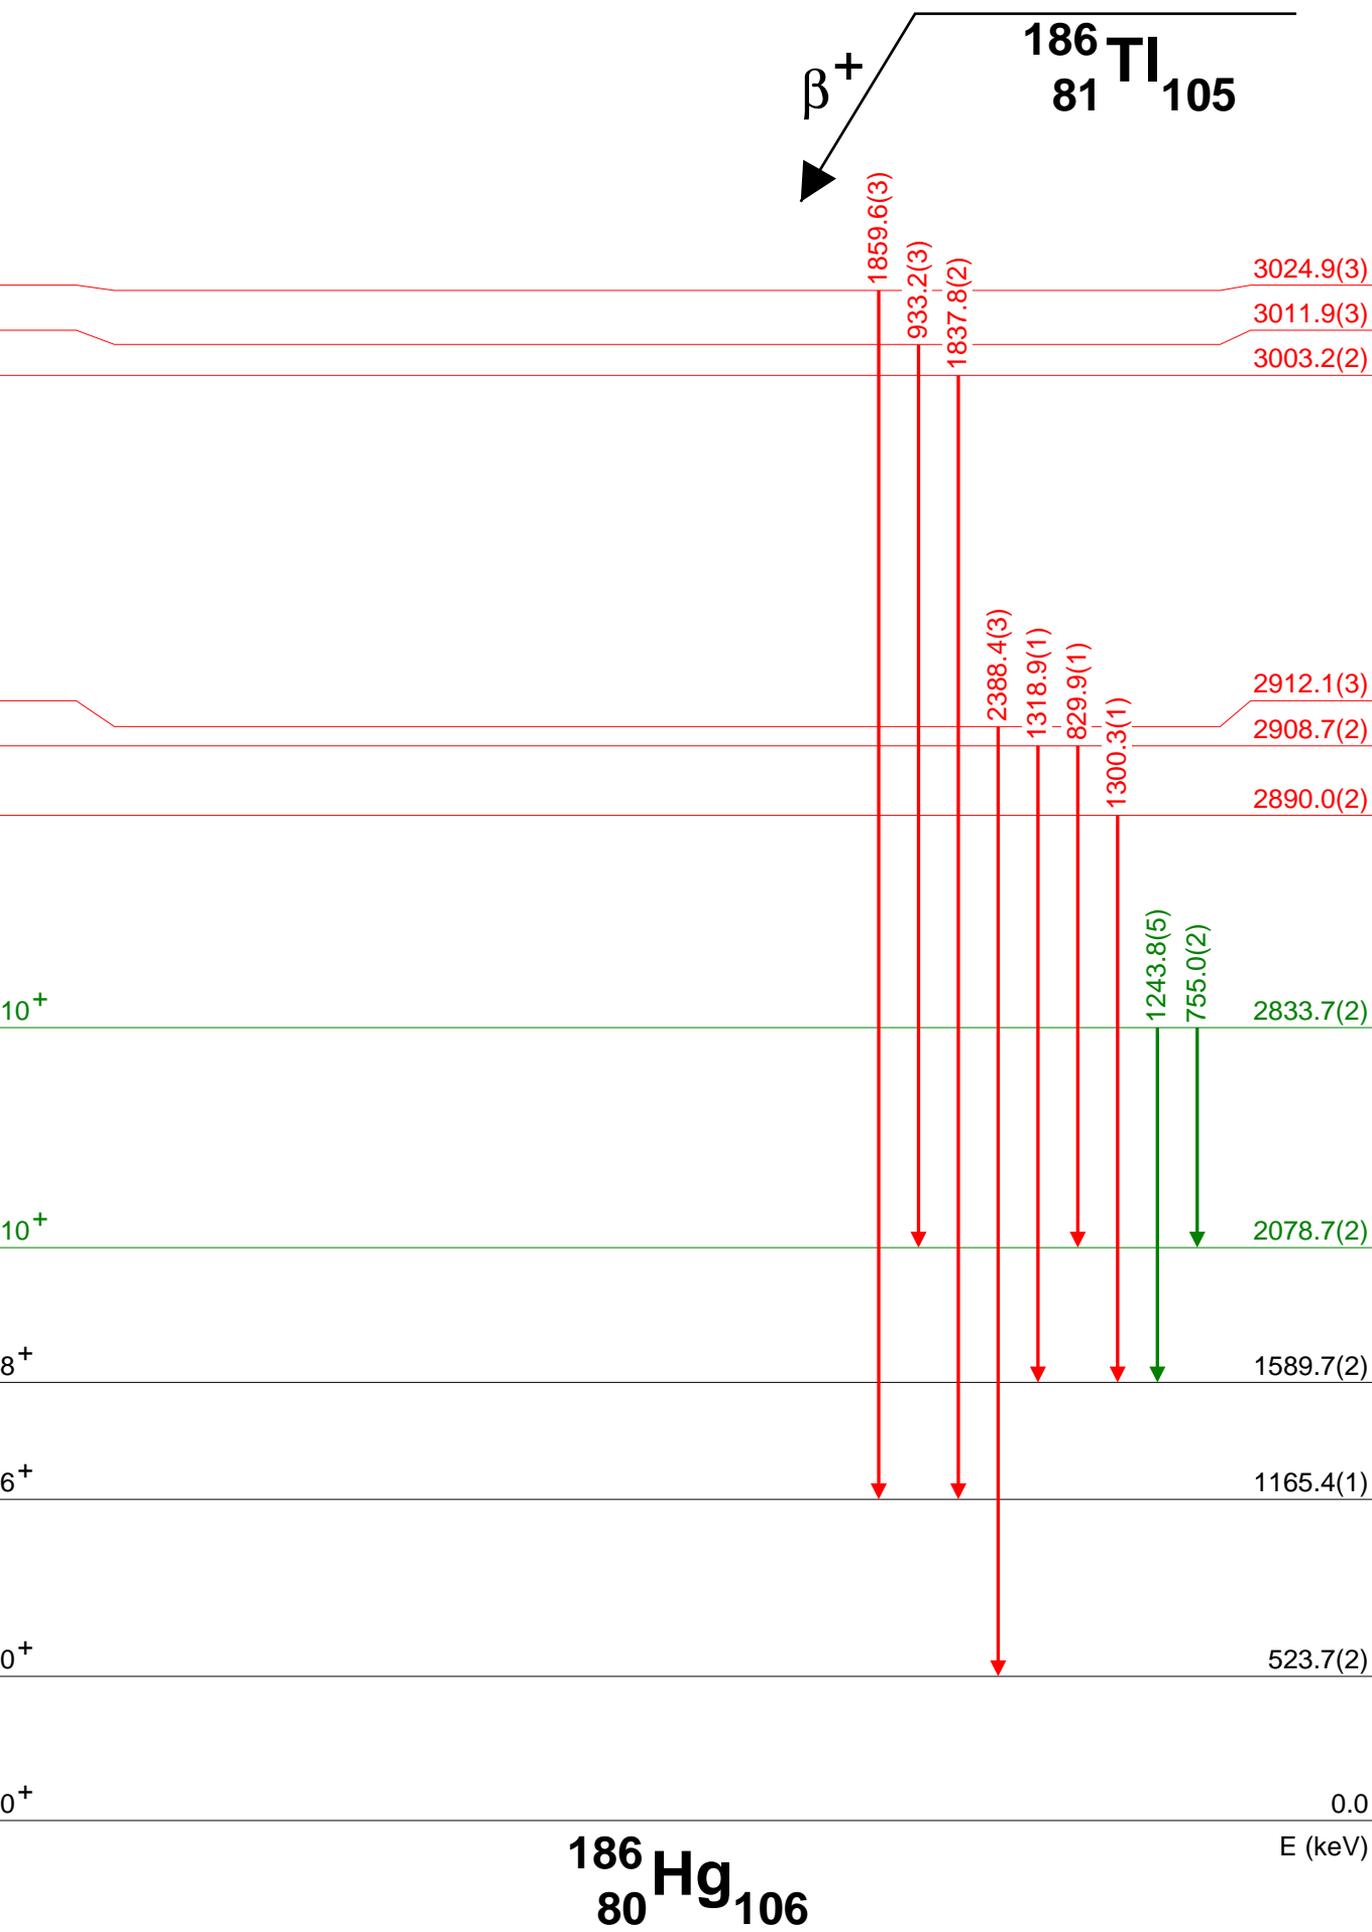

Supplement: Supplementary file 4 [file 20230329_186Hg_decayscheme.pdf]
